# Supplementary material for: Dielectronic recombination studies of ions relevant to kilonovae and non-LTE plasma
Source: arXiv:2504.06639 source file (2025-06-19)
Supplement: Supplementary file 1 [file Supplementary-data.pdf]

**$Y^+$ : Energy vs DR cross section**

| Energy (eV) | Barn | | | | | | | | |
|---|---|---|---|---|---|---|---|---|---|
| | | 0.245 | 6.79001E6 | 0.510 | 1.82724E6 | 0.775 | 6.881E+05 | 1.040 | 8.229E+05 |
| | | 0.250 | 6.91656E6 | 0.515 | 1.9309E6 | 0.780 | 6.767E+05 | 1.045 | 8.006E+05 |
| | | 0.255 | 7.05561E6 | 0.520 | 2.07121E6 | 0.785 | 6.649E+05 | 1.050 | 7.807E+05 |
| | | 0.260 | 7.20583E6 | 0.525 | 2.24643E6 | 0.790 | 6.533E+05 | 1.055 | 7.635E+05 |
| 0.000 | 7.61075E7 | 0.265 | 7.36545E6 | 0.530 | 2.45388E6 | 0.795 | 6.422E+05 | 1.060 | 7.492E+05 |
| 0.005 | 7.64364E7 | 0.270 | 7.53286E6 | 0.535 | 2.68987E6 | 0.800 | 6.325E+05 | 1.065 | 7.379E+05 |
| 0.010 | 7.59255E7 | 0.275 | 7.706E6 | 0.540 | 2.94963E6 | 0.805 | 6.247E+05 | 1.070 | 7.301E+05 |
| 0.015 | 7.46E7 | 0.280 | 7.88255E6 | 0.545 | 3.2273E6 | 0.810 | 6.197E+05 | 1.075 | 7.256E+05 |
| 0.020 | 7.25136E7 | 0.285 | 8.06002E6 | 0.550 | 3.516E6 | 0.815 | 6.184E+05 | 1.080 | 7.247E+05 |
| 0.025 | 6.9746E7 | 0.290 | 8.23561E6 | 0.555 | 3.80797E6 | 0.820 | 6.214E+05 | 1.085 | 7.274E+05 |
| 0.030 | 6.63974E7 | 0.295 | 8.40637E6 | 0.560 | 4.09478E6 | 0.825 | 6.296E+05 | 1.090 | 7.336E+05 |
| 0.035 | 6.2583E7 | 0.300 | 8.56915E6 | 0.565 | 4.36764E6 | 0.830 | 6.434E+05 | 1.095 | 7.433E+05 |
| 0.040 | 5.84261E7 | 0.305 | 8.72069E6 | 0.570 | 4.61768E6 | 0.835 | 6.633E+05 | 1.100 | 7.564E+05 |
| 0.045 | 5.40522E7 | 0.310 | 8.85777E6 | 0.575 | 4.83639E6 | 0.840 | 6.895E+05 | 1.105 | 7.727E+05 |
| 0.050 | 4.95824E7 | 0.315 | 8.97714E6 | 0.580 | 5.01602E6 | 0.845 | 7.219E+05 | 1.110 | 7.919E+05 |
| 0.055 | 4.51284E7 | 0.320 | 9.07573E6 | 0.585 | 5.14997E6 | 0.850 | 7.603E+05 | 1.115 | 8.138E+05 |
| 0.060 | 4.07883E7 | 0.325 | 9.15073E6 | 0.590 | 5.23311E6 | 0.855 | 8.039E+05 | 1.120 | 8.382E+05 |
| 0.065 | 3.66439E7 | 0.330 | 9.19955E6 | 0.595 | 5.2621E6 | 0.860 | 8.520E+05 | 1.125 | 8.645E+05 |
| 0.070 | 3.27587E7 | 0.335 | 9.22004E6 | 0.600 | 5.2356E6 | 0.865 | 9.034E+05 | 1.130 | 8.925E+05 |
| 0.075 | 2.91783E7 | 0.340 | 9.21047E6 | 0.605 | 5.1543E6 | 0.870 | 9.569E+05 | 1.135 | 9.218E+05 |
| 0.080 | 2.59305E7 | 0.345 | 9.16955E6 | 0.610 | 5.02088E6 | 0.875 | 1.01116E6 | 1.140 | 9.518E+05 |
| 0.085 | 2.30273E7 | 0.350 | 9.09659E6 | 0.615 | 4.83991E6 | 0.880 | 1.06474E6 | 1.145 | 9.823E+05 |
| 0.090 | 2.04671E7 | 0.355 | 8.9913E6 | 0.620 | 4.61755E6 | 0.885 | 1.11626E6 | 1.150 | 1.01261E6 |
| 0.095 | 1.82373E7 | 0.360 | 8.85395E6 | 0.625 | 4.36121E6 | 0.890 | 1.16446E6 | 1.155 | 1.04231E6 |
| 0.100 | 1.6317E7 | 0.365 | 8.68526E6 | 0.630 | 4.07911E6 | 0.895 | 1.20824E6 | 1.160 | 1.0709E6 |
| 0.105 | 1.46795E7 | 0.370 | 8.48643E6 | 0.635 | 3.77989E6 | 0.900 | 1.24672E6 | 1.165 | 1.09786E6 |
| 0.110 | 1.32949E7 | 0.375 | 8.25904E6 | 0.640 | 3.47212E6 | 0.905 | 1.27927E6 | 1.170 | 1.12268E6 |
| 0.115 | 1.2132E7 | 0.380 | 8.00511E6 | 0.645 | 3.16395E6 | 0.910 | 1.3055E6 | 1.175 | 1.14487E6 |
| 0.120 | 1.11601E7 | 0.385 | 7.72696E6 | 0.650 | 2.8627E6 | 0.915 | 1.32529E6 | 1.180 | 1.16394E6 |
| 0.125 | 1.03501E7 | 0.390 | 7.42716E6 | 0.655 | 2.57471E6 | 0.920 | 1.33874E6 | 1.185 | 1.17667E6 |
| 0.130 | 9.67526E6 | 0.395 | 7.10865E6 | 0.660 | 2.305E6 | 0.925 | 1.34614E6 | 1.190 | 1.18872E6 |
| 0.135 | 9.1121E6 | 0.400 | 6.77446E6 | 0.665 | 2.05735E6 | 0.930 | 1.3479E6 | 1.195 | 1.19637E6 |
| 0.140 | 8.64033E6 | 0.405 | 6.42784E6 | 0.670 | 1.83419E6 | 0.935 | 1.34457E6 | 1.200 | 1.19933E6 |
| 0.145 | 8.24294E6 | 0.410 | 6.07216E6 | 0.675 | 1.63673E6 | 0.940 | 1.33669E6 | 1.205 | 1.19741E6 |
| 0.150 | 7.90602E6 | 0.415 | 5.71088E6 | 0.680 | 1.46508E6 | 0.945 | 1.32485E6 | 1.210 | 1.19048E6 |
| 0.155 | 7.61855E6 | 0.420 | 5.34748E6 | 0.685 | 1.31845E6 | 0.950 | 1.30958E6 | 1.215 | 1.17852E6 |
| 0.160 | 7.37194E6 | 0.425 | 4.98545E6 | 0.690 | 1.19531E6 | 0.955 | 1.29138E6 | 1.220 | 1.16161E6 |
| 0.165 | 7.15975E6 | 0.430 | 4.62824E6 | 0.695 | 1.09362E6 | 0.960 | 1.27067E6 | 1.225 | 1.13992E6 |
| 0.170 | 6.97725E6 | 0.435 | 4.27919E6 | 0.700 | 1.01103E6 | 0.965 | 1.24784E6 | 1.230 | 1.11371E6 |
| 0.175 | 6.82108E6 | 0.440 | 3.94155E6 | 0.705 | 9.450E+05 | 0.970 | 1.22319E6 | 1.235 | 1.08335E6 |
| 0.180 | 6.68892E6 | 0.445 | 3.61844E6 | 0.710 | 8.930E+05 | 0.975 | 1.19701E6 | 1.240 | 1.04927E6 |
| 0.185 | 6.57925E6 | 0.450 | 3.3128E6 | 0.715 | 8.527E+05 | 0.980 | 1.16952E6 | 1.245 | 1.01196E6 |
| 0.190 | 6.48988E6 | 0.455 | 3.02738E6 | 0.720 | 8.217E+05 | 0.985 | 1.14095E6 | 1.250 | 9.720E+05 |
| 0.195 | 6.42273E6 | 0.460 | 2.76474E6 | 0.725 | 7.980E+05 | 0.990 | 1.11152E6 | 1.255 | 9.299E+05 |
| 0.200 | 6.37595E6 | 0.465 | 2.52727E6 | 0.730 | 7.799E+05 | 0.995 | 1.08144E6 | 1.260 | 8.864E+05 |
| 0.205 | 6.34882E6 | 0.470 | 2.31716E6 | 0.735 | 7.658E+05 | 1.000 | 1.05095E6 | 1.265 | 8.421E+05 |
| 0.210 | 6.34129E6 | 0.475 | 2.13646E6 | 0.740 | 7.544E+05 | 1.005 | 1.02027E6 | 1.270 | 7.975E+05 |
| 0.215 | 6.35291E6 | 0.480 | 1.98701E6 | 0.745 | 7.447E+05 | 1.010 | 9.897E+05 | 1.275 | 7.533E+05 |
| 0.220 | 6.38307E6 | 0.485 | 1.87052E6 | 0.750 | 7.359E+05 | 1.015 | 9.594E+05 | 1.280 | 7.101E+05 |
| 0.225 | 6.43133E6 | 0.490 | 1.78852E6 | 0.755 | 7.273E+05 | 1.020 | 9.297E+05 | 1.285 | 6.683E+05 |
| 0.230 | 6.49692E6 | 0.495 | 1.74231E6 | 0.760 | 7.185E+05 | 1.025 | 9.009E+05 | 1.290 | 6.284E+05 |
| 0.235 | 6.57915E6 | 0.500 | 1.73296E6 | 0.765 | 7.091E+05 | 1.030 | 8.733E+05 | 1.295 | 5.909E+05 |
| 0.240 | 6.67718E6 | 0.505 | 1.76118E6 | 0.770 | 6.990E+05 | 1.035 | 8.472E+05 | 1.300 | 5.562E+05 |

| | | | | | | | | | |
|---|---|---|---|---|---|---|---|---|---|
| 1.305 | 5.246E+05 | 1.570 | 5.642E+05 | 1.835 | 1.65155E6 | 2.100 | 1.27989E6 | 2.365 | 7.203E+04 |
| 1.310 | 4.965E+05 | 1.575 | 5.763E+05 | 1.840 | 1.67611E6 | 2.105 | 1.27458E6 | 2.370 | 7.143E+04 |
| 1.315 | 4.721E+05 | 1.580 | 5.884E+05 | 1.845 | 1.70324E6 | 2.110 | 1.25999E6 | 2.375 | 7.080E+04 |
| 1.320 | 4.517E+05 | 1.585 | 6.004E+05 | 1.850 | 1.73341E6 | 2.115 | 1.23532E6 | 2.380 | 7.018E+04 |
| 1.325 | 4.357E+05 | 1.590 | 6.119E+05 | 1.855 | 1.767E6 | 2.120 | 1.20033E6 | 2.385 | 6.958E+04 |
| 1.330 | 4.241E+05 | 1.595 | 6.227E+05 | 1.860 | 1.80433E6 | 2.125 | 1.15535E6 | 2.390 | 6.906E+04 |
| 1.335 | 4.173E+05 | 1.600 | 6.326E+05 | 1.865 | 1.84561E6 | 2.130 | 1.10126E6 | 2.395 | 6.865E+04 |
| 1.340 | 4.153E+05 | 1.605 | 6.415E+05 | 1.870 | 1.89094E6 | 2.135 | 1.03936E6 | 2.400 | 6.842E+04 |
| 1.345 | 4.182E+05 | 1.610 | 6.494E+05 | 1.875 | 1.94027E6 | 2.140 | 9.713E+05 | 2.405 | 6.841E+04 |
| 1.350 | 4.261E+05 | 1.615 | 6.563E+05 | 1.880 | 1.99339E6 | 2.145 | 8.990E+05 | 2.410 | 6.866E+04 |
| 1.355 | 4.390E+05 | 1.620 | 6.624E+05 | 1.885 | 2.04991E6 | 2.150 | 8.243E+05 | 2.415 | 6.920E+04 |
| 1.360 | 4.566E+05 | 1.625 | 6.676E+05 | 1.890 | 2.10926E6 | 2.155 | 7.491E+05 | 2.420 | 7.005E+04 |
| 1.365 | 4.787E+05 | 1.630 | 6.724E+05 | 1.895 | 2.17069E6 | 2.160 | 6.754E+05 | 2.425 | 7.120E+04 |
| 1.370 | 5.048E+05 | 1.635 | 6.768E+05 | 1.900 | 2.23325E6 | 2.165 | 6.046E+05 | 2.430 | 7.261E+04 |
| 1.375 | 5.344E+05 | 1.640 | 6.812E+05 | 1.905 | 2.29586E6 | 2.170 | 5.380E+05 | 2.435 | 7.421E+04 |
| 1.380 | 5.667E+05 | 1.645 | 6.859E+05 | 1.910 | 2.35727E6 | 2.175 | 4.765E+05 | 2.440 | 7.594E+04 |
| 1.385 | 6.009E+05 | 1.650 | 6.911E+05 | 1.915 | 2.41614E6 | 2.180 | 4.209E+05 | 2.445 | 7.768E+04 |
| 1.390 | 6.360E+05 | 1.655 | 6.973E+05 | 1.920 | 2.47105E6 | 2.185 | 3.713E+05 | 2.450 | 7.932E+04 |
| 1.395 | 6.708E+05 | 1.660 | 7.046E+05 | 1.925 | 2.52057E6 | 2.190 | 3.280E+05 | 2.455 | 8.073E+04 |
| 1.400 | 7.044E+05 | 1.665 | 7.135E+05 | 1.930 | 2.56331E6 | 2.195 | 2.905E+05 | 2.460 | 8.179E+04 |
| 1.405 | 7.355E+05 | 1.670 | 7.241E+05 | 1.935 | 2.5979E6 | 2.200 | 2.587E+05 | 2.465 | 8.239E+04 |
| 1.410 | 7.632E+05 | 1.675 | 7.368E+05 | 1.940 | 2.62314E6 | 2.205 | 2.319E+05 | 2.470 | 8.242E+04 |
| 1.415 | 7.865E+05 | 1.680 | 7.517E+05 | 1.945 | 2.63798E6 | 2.210 | 2.097E+05 | 2.475 | 8.180E+04 |
| 1.420 | 8.047E+05 | 1.685 | 7.690E+05 | 1.950 | 2.64156E6 | 2.215 | 1.913E+05 | 2.480 | 8.050E+04 |
| 1.425 | 8.172E+05 | 1.690 | 7.888E+05 | 1.955 | 2.63328E6 | 2.220 | 1.762E+05 | 2.485 | 7.849E+04 |
| 1.430 | 8.237E+05 | 1.695 | 8.113E+05 | 1.960 | 2.61278E6 | 2.225 | 1.637E+05 | 2.490 | 7.579E+04 |
| 1.435 | 8.242E+05 | 1.700 | 8.364E+05 | 1.965 | 2.57998E6 | 2.230 | 1.534E+05 | 2.495 | 7.245E+04 |
| 1.440 | 8.188E+05 | 1.705 | 8.642E+05 | 1.970 | 2.53511E6 | 2.235 | 1.448E+05 | 2.500 | 6.854E+04 |
| 1.445 | 8.079E+05 | 1.710 | 8.945E+05 | 1.975 | 2.47869E6 | 2.240 | 1.375E+05 | | |
| 1.450 | 7.923E+05 | 1.715 | 9.271E+05 | 1.980 | 2.41152E6 | 2.245 | 1.312E+05 | | |
| 1.455 | 7.726E+05 | 1.720 | 9.620E+05 | 1.985 | 2.33469E6 | 2.250 | 1.256E+05 | | |
| 1.460 | 7.498E+05 | 1.725 | 9.987E+05 | 1.990 | 2.24957E6 | 2.255 | 1.206E+05 | | |
| 1.465 | 7.248E+05 | 1.730 | 1.03684E6 | 1.995 | 2.15776E6 | 2.260 | 1.159E+05 | | |
| 1.470 | 6.986E+05 | 1.735 | 1.07614E6 | 2.000 | 2.06107E6 | 2.265 | 1.116E+05 | | |
| 1.475 | 6.720E+05 | 1.740 | 1.1161E6 | 2.005 | 1.96149E6 | 2.270 | 1.075E+05 | | |
| 1.480 | 6.458E+05 | 1.745 | 1.15627E6 | 2.010 | 1.86113E6 | 2.275 | 1.036E+05 | | |
| 1.485 | 6.208E+05 | 1.750 | 1.19617E6 | 2.015 | 1.76216E6 | 2.280 | 9.986E+04 | | |
| 1.490 | 5.976E+05 | 1.755 | 1.23535E6 | 2.020 | 1.66675E6 | 2.285 | 9.637E+04 | | |
| 1.495 | 5.767E+05 | 1.760 | 1.27339E6 | 2.025 | 1.57697E6 | 2.290 | 9.311E+04 | | |
| 1.500 | 5.582E+05 | 1.765 | 1.3099E6 | 2.030 | 1.49474E6 | 2.295 | 9.010E+04 | | |
| 1.505 | 5.425E+05 | 1.770 | 1.34458E6 | 2.035 | 1.42173E6 | 2.300 | 8.735E+04 | | |
| 1.510 | 5.297E+05 | 1.775 | 1.37721E6 | 2.040 | 1.35927E6 | 2.305 | 8.487E+04 | | |
| 1.515 | 5.198E+05 | 1.780 | 1.40766E6 | 2.045 | 1.30827E6 | 2.310 | 8.270E+04 | | |
| 1.520 | 5.127E+05 | 1.785 | 1.4359E6 | 2.050 | 1.26916E6 | 2.315 | 8.081E+04 | | |
| 1.525 | 5.084E+05 | 1.790 | 1.46198E6 | 2.055 | 1.24185E6 | 2.320 | 7.920E+04 | | |
| 1.530 | 5.067E+05 | 1.795 | 1.48608E6 | 2.060 | 1.22571E6 | 2.325 | 7.784E+04 | | |
| 1.535 | 5.075E+05 | 1.800 | 1.50845E6 | 2.065 | 1.21958E6 | 2.330 | 7.671E+04 | | |
| 1.540 | 5.106E+05 | 1.805 | 1.52942E6 | 2.070 | 1.22178E6 | 2.335 | 7.578E+04 | | |
| 1.545 | 5.158E+05 | 1.810 | 1.5494E6 | 2.075 | 1.23026E6 | 2.340 | 7.500E+04 | | |
| 1.550 | 5.228E+05 | 1.815 | 1.56885E6 | 2.080 | 1.24263E6 | 2.345 | 7.433E+04 | | |
| 1.555 | 5.315E+05 | 1.820 | 1.58826E6 | 2.085 | 1.25631E6 | 2.350 | 7.373E+04 | | |
| 1.560 | 5.414E+05 | 1.825 | 1.60815E6 | 2.090 | 1.26871E6 | 2.355 | 7.317E+04 | | |
| 1.565 | 5.524E+05 | 1.830 | 1.62907E6 | 2.095 | 1.27732E6 | 2.360 | 7.261E+04 | | |

**$Sr^+$ : Energy vs DR cross section**

| Energy (eV) | Barn |
|---|---|
| 0 | 623518.5 |
| 0.005 | 623367.41 |
| 0.01 | 622638.42 |
| 0.015 | 621335.03 |
| 0.02 | 619463.65 |
| 0.025 | 617033.56 |
| 0.03 | 614056.88 |
| 0.035 | 610547.6 |
| 0.04 | 606522.62 |
| 0.045 | 602000.94 |
| 0.05 | 597003.36 |
| 0.055 | 591552.88 |
| 0.06 | 585673.51 |
| 0.065 | 579390.84 |
| 0.07 | 572731.66 |
| 0.075 | 565723.29 |
| 0.08 | 558394.03 |
| 0.085 | 550772.06 |
| 0.09 | 542886.19 |
| 0.095 | 534764.63 |
| 0.1 | 526435.77 |
| 0.105 | 517927.21 |
| 0.11 | 509266.11 |
| 0.115 | 500478.86 |
| 0.12 | 491590.62 |
| 0.125 | 482625.98 |
| 0.13 | 473608.14 |
| 0.135 | 464559.01 |
| 0.14 | 455499.5 |
| 0.145 | 446448.98 |
| 0.15 | 437425.75 |
| 0.155 | 428446.53 |
| 0.16 | 419526.82 |
| 0.165 | 410680.8 |
| 0.17 | 401921.39 |
| 0.175 | 393260.18 |
| 0.18 | 384707.56 |
| 0.185 | 376272.76 |
| 0.19 | 367963.95 |
| 0.195 | 359788.04 |
| 0.2 | 351751.14 |
| 0.205 | 343858.43 |
| 0.21 | 336114.03 |
| 0.215 | 328521.53 |
| 0.22 | 321083.33 |
| 0.225 | 313801.53 |
| 0.23 | 306677.43 |
| 0.235 | 299711.64 |
| 0.24 | 292904.45 |
| 0.245 | 286255.66 |
| 0.25 | 279764.47 |
| 0.255 | 273429.79 |
| 0.26 | 267250.3 |
| 0.265 | 261224.23 |
| 0.27 | 255349.95 |
| 0.275 | 249624.88 |
| 0.28 | 244046.81 |
| 0.285 | 238613.15 |
| 0.29 | 233321.49 |
| 0.295 | 228169.13 |
| 0.3 | 223153.47 |
| 0.305 | 218271.72 |
| 0.31 | 213521.28 |
| 0.315 | 208899.74 |
| 0.32 | 204404.6 |
| 0.325 | 200033.77 |
| 0.33 | 195785.34 |
| 0.335 | 191657.42 |
| 0.34 | 187648.8 |
| 0.345 | 183758.08 |
| 0.35 | 179984.58 |
| 0.355 | 176327.57 |
| 0.36 | 172786.57 |
| 0.365 | 169361.08 |
| 0.37 | 166050.39 |
| 0.375 | 162853.71 |
| 0.38 | 159769.64 |
| 0.385 | 156795.97 |
| 0.39 | 153929.7 |
| 0.395 | 151166.85 |
| 0.4 | 148501.6 |
| 0.405 | 145927.45 |
| 0.41 | 143436.42 |
| 0.415 | 141019.49 |
| 0.42 | 138666.46 |
| 0.425 | 136366.85 |
| 0.43 | 134109.94 |
| 0.435 | 131885.34 |
| 0.44 | 129683.55 |
| 0.445 | 127496.17 |
| 0.45 | 125316.79 |
| 0.455 | 123140.93 |
| 0.46 | 120966.27 |
| 0.465 | 118793.03 |
| 0.47 | 116622.99 |
| 0.475 | 114460.46 |
| 0.48 | 112310.85 |
| 0.485 | 110180.84 |
| 0.49 | 108077.65 |
| 0.495 | 106008.67 |
| 0.5 | 103980.8 |
| 0.505 | 102000.24 |
| 0.51 | 100072.29 |
| 0.515 | 98200.7 |
| 0.52 | 96388.24 |
| 0.525 | 94636.09 |
| 0.53 | 92944.36 |
| 0.535 | 91312.09 |
| 0.54 | 89737.45 |
| 0.545 | 88217.95 |
| 0.55 | 86750.68 |
| 0.555 | 85332.51 |
| 0.56 | 83960.23 |
| 0.565 | 82630.71 |
| 0.57 | 81341.03 |
| 0.575 | 80088.45 |
| 0.58 | 78870.43 |
| 0.585 | 77684.87 |
| 0.59 | 76529.9 |
| 0.595 | 75403.91 |
| 0.6 | 74305.56 |
| 0.605 | 73234.03 |
| 0.61 | 72187.99 |
| 0.615 | 71166.93 |
| 0.62 | 70170.37 |
| 0.625 | 69198.24 |
| 0.63 | 68250.12 |
| 0.635 | 67326.36 |
| 0.64 | 66427.47 |
| 0.645 | 65553.94 |
| 0.65 | 64707.45 |
| 0.655 | 63889.01 |
| 0.66 | 63100.56 |
| 0.665 | 62344.4 |
| 0.67 | 61623.18 |
| 0.675 | 60939.92 |
| 0.68 | 60297.89 |
| 0.685 | 59700.56 |
| 0.69 | 59151.38 |
| 0.695 | 58653.57 |
| 0.7 | 58210.01 |
| 0.705 | 57822.82 |
| 0.71 | 57493.21 |
| 0.715 | 57221.19 |
| 0.72 | 57005.34 |
| 0.725 | 56842.56 |
| 0.73 | 56728.21 |
| 0.735 | 56655.81 |
| 0.74 | 56617.27 |
| 0.745 | 56603.29 |
| 0.75 | 56603.52 |
| 0.755 | 56607.02 |
| 0.76 | 56602.85 |
| 0.765 | 56580.59 |
| 0.77 | 56530.88 |
| 0.775 | 56446.36 |
| 0.78 | 56321.05 |
| 0.785 | 56151.65 |
| 0.79 | 55937.79 |
| 0.795 | 55681.75 |
| 0.8 | 55388.45 |
| 0.805 | 55065.58 |
| 0.81 | 54722.6 |
| 0.815 | 54371.07 |
| 0.82 | 54023.92 |
| 0.825 | 53694.79 |
| 0.83 | 53397.6 |
| 0.835 | 53145.84 |
| 0.84 | 52952.07 |
| 0.845 | 52827.26 |
| 0.85 | 52780.32 |
| 0.855 | 52817.34 |
| 0.86 | 52941.41 |
| 0.865 | 53152.08 |
| 0.87 | 53445.13 |
| 0.875 | 53812.55 |
| 0.88 | 54242.19 |
| 0.885 | 54718.6 |
| 0.89 | 55222.95 |
| 0.895 | 55733.97 |
| 0.9 | 56228.59 |
| 0.905 | 56682.95 |
| 0.91 | 57073.36 |
| 0.915 | 57377.28 |
| 0.92 | 57574.56 |
| 0.925 | 57648.02 |
| 0.93 | 57584.53 |
| 0.935 | 57375.36 |
| 0.94 | 57016.68 |
| 0.945 | 56509.27 |
| 0.95 | 55858.78 |
| 0.955 | 55075.18 |
| 0.96 | 54172.02 |
| 0.965 | 53165.85 |
| 0.97 | 52075.3 |
| 0.975 | 50920.44 |
| 0.98 | 49721.74 |
| 0.985 | 48498.87 |
| 0.99 | 47270.41 |
| 0.995 | 46053.41 |
| 1 | 44862.69 |
| 1.005 | 43710.54 |
| 1.01 | 42606.72 |
| 1.015 | 41557.83 |
| 1.02 | 40568.59 |
| 1.025 | 39640.82 |
| 1.03 | 38774.77 |
| 1.035 | 37968.73 |
| 1.04 | 37220.07 |
| 1.045 | 36525.26 |
| 1.05 | 35880.68 |
| 1.055 | 35282.83 |
| 1.06 | 34728.68 |
| 1.065 | 34216.11 |
| 1.07 | 33744.07 |
| 1.075 | 33312.71 |
| 1.08 | 32923.52 |
| 1.085 | 32578.93 |
| 1.09 | 32283.11 |
| 1.095 | 32040.59 |
| 1.1 | 31856.89 |
| 1.105 | 31737.68 |
| 1.11 | 31688.76 |
| 1.115 | 31715.29 |
| 1.12 | 31821.48 |
| 1.125 | 32010.28 |
| 1.13 | 32281.68 |
| 1.135 | 32634.12 |
| 1.14 | 33062.32 |
| 1.145 | 33558.01 |
| 1.15 | 34109.24 |
| 1.155 | 34700.2 |
| 1.16 | 35312.49 |
| 1.165 | 35923.8 |
| 1.17 | 36510.55 |
| 1.175 | 37047.73 |
| 1.18 | 37510.56 |
| 1.185 | 37875.2 |
| 1.19 | 38120.88 |
| 1.195 | 38230.78 |
| 1.2 | 38192.98 |
| 1.205 | 38001.68 |
| 1.21 | 37657.78 |
| 1.215 | 37168.71 |
| 1.22 | 36548.8 |
| 1.225 | 35818.32 |
| 1.23 | 35002.79 |
| 1.235 | 34131.69 |
| 1.24 | 33237.16 |
| 1.245 | 32352.43 |
| 1.25 | 31510.26 |
| 1.255 | 30742.36 |
| 1.26 | 30075.25 |
| 1.265 | 29532.71 |
| 1.27 | 29132.55 |
| 1.275 | 28886.99 |
| 1.28 | 28801.29 |
| 1.285 | 28874.08 |
| 1.29 | 29097.66 |
| 1.295 | 29458.49 |

| | | | | | | | | | |
|---|---|---|---|---|---|---|---|---|---|
| 1.3 | 29937.2 | 1.565 | 25889.98 | 1.83 | 29414.16 | 2.095 | 48900.46 | 2.36 | 198036 |
| 1.305 | 30510.09 | 1.57 | 25912.46 | 1.835 | 29423.33 | 2.1 | 49279.11 | 2.365 | 193856.32 |
| 1.31 | 31149.18 | 1.575 | 26093.08 | 1.84 | 29451.32 | 2.105 | 49508.18 | 2.37 | 188981.22 |
| 1.315 | 31824.86 | 1.58 | 26423.68 | 1.845 | 29491.89 | 2.11 | 49575.81 | 2.375 | 183665.97 |
| 1.32 | 32506.2 | 1.585 | 26894.78 | 1.85 | 29540.86 | 2.115 | 49474.69 | 2.38 | 178160.01 |
| 1.325 | 33162.95 | 1.59 | 27494.77 | 1.855 | 29596.81 | 2.12 | 49205.41 | 2.385 | 172691.83 |
| 1.33 | 33766.53 | 1.595 | 28211.84 | 1.86 | 29661.05 | 2.125 | 48774.65 | 2.39 | 167459.93 |
| 1.335 | 34291.85 | 1.6 | 29032.94 | 1.865 | 29737.27 | 2.13 | 48195.57 | 2.395 | 162621.98 |
| 1.34 | 34718.54 | 1.605 | 29944 | 1.87 | 29831.78 | 2.135 | 47487.71 | 2.4 | 158292.66 |
| 1.345 | 35032.43 | 1.61 | 30929.85 | 1.875 | 29952.05 | 2.14 | 46675.75 | 2.405 | 154541.03 |
| 1.35 | 35225.24 | 1.615 | 31974.26 | 1.88 | 30107.21 | 2.145 | 45787.28 | 2.41 | 151395.02 |
| 1.355 | 35296.85 | 1.62 | 33059.76 | 1.885 | 30305.28 | 2.15 | 44853.9 | 2.415 | 148844.46 |
| 1.36 | 35254.48 | 1.625 | 34167.9 | 1.89 | 30553.53 | 2.155 | 43907.28 | 2.42 | 146850.04 |
| 1.365 | 35112.82 | 1.63 | 35279.12 | 1.895 | 30857.41 | 2.16 | 42979.18 | 2.425 | 145350.31 |
| 1.37 | 34892.56 | 1.635 | 36372.61 | 1.9 | 31219.09 | 2.165 | 42102.47 | 2.43 | 144273.53 |
| 1.375 | 34620.7 | 1.64 | 37428.1 | 1.905 | 31637.51 | 2.17 | 41308.85 | 2.435 | 143540.88 |
| 1.38 | 34328.08 | 1.645 | 38424.72 | 1.91 | 32108.66 | 2.175 | 40627.87 | 2.44 | 143078.62 |
| 1.385 | 34048.15 | 1.65 | 39342.94 | 1.915 | 32624.14 | 2.18 | 40088.2 | 2.445 | 142820.51 |
| 1.39 | 33814.41 | 1.655 | 40164.52 | 1.92 | 33173.29 | 2.185 | 39717.25 | 2.45 | 142712 |
| 1.395 | 33658.5 | 1.66 | 40873.91 | 1.925 | 33743.05 | 2.19 | 39541.6 | 2.455 | 142712.69 |
| 1.4 | 33608.56 | 1.665 | 41458.55 | 1.93 | 34318.9 | 2.195 | 39587.18 | 2.46 | 142797.27 |
| 1.405 | 33686.86 | 1.67 | 41909.16 | 1.935 | 34886.14 | 2.2 | 39880.33 | 2.465 | 142951.75 |
| 1.41 | 33906.94 | 1.675 | 42220.79 | 1.94 | 35430.63 | 2.205 | 40448.83 | 2.47 | 143174.25 |
| 1.415 | 34274.44 | 1.68 | 42392.45 | 1.945 | 35939.95 | 2.21 | 41322.55 | 2.475 | 143471.49 |
| 1.42 | 34785.12 | 1.685 | 42428.07 | 1.95 | 36404.36 | 2.215 | 42534.47 | 2.48 | 143855.8 |
| 1.425 | 35424.37 | 1.69 | 42334.58 | 1.955 | 36817.77 | 2.22 | 44121.54 | 2.485 | 144342.98 |
| 1.43 | 36168.44 | 1.695 | 42122.31 | 1.96 | 37176.4 | 2.225 | 46125.35 | 2.49 | 144951.38 |
| 1.435 | 36985.18 | 1.7 | 41804.1 | 1.965 | 37480.7 | 2.23 | 48590.89 | 2.495 | 145699.36 |
| 1.44 | 37835.28 | 1.705 | 41394.13 | 1.97 | 37734.54 | 2.235 | 51568.61 | 2.5 | 146605.67 |
| 1.445 | 38676.66 | 1.71 | 40907.37 | 1.975 | 37943.81 | 2.24 | 55110.46 | 2.505 | 147688.84 |
| 1.45 | 39462.84 | 1.715 | 40358.31 | 1.98 | 38117.29 | 2.245 | 59269.72 | 2.51 | 148968.58 |
| 1.455 | 40149.53 | 1.72 | 39760.22 | 1.985 | 38265.54 | 2.25 | 64097.18 | 2.515 | 150466.21 |
| 1.46 | 40695.62 | 1.725 | 39125.2 | 1.99 | 38399.63 | 2.255 | 69636.46 | 2.52 | 152205.07 |
| 1.465 | 41066.26 | 1.73 | 38463.48 | 1.995 | 38530.8 | 2.26 | 75920.28 | 2.525 | 154210.96 |
| 1.47 | 41233.81 | 1.735 | 37783.78 | 2 | 38670.23 | 2.265 | 82963.83 | 2.53 | 156513.65 |
| 1.475 | 41181.08 | 1.74 | 37093.2 | 2.005 | 38829.56 | 2.27 | 90759.62 | 2.535 | 159144.62 |
| 1.48 | 40901.2 | 1.745 | 36397.82 | 2.01 | 39018.37 | 2.275 | 99270.88 | 2.54 | 162131.93 |
| 1.485 | 40397.79 | 1.75 | 35703.37 | 2.015 | 39246.06 | 2.28 | 108429.37 | 2.545 | 165502.39 |
| 1.49 | 39684.68 | 1.755 | 35015.39 | 2.02 | 39520.81 | 2.285 | 118127.69 | 2.55 | 169280.78 |
| 1.495 | 38785.22 | 1.76 | 34339.53 | 2.025 | 39850.25 | 2.29 | 128222.17 | 2.555 | 173480.6 |
| 1.5 | 37730.1 | 1.765 | 33682.4 | 2.03 | 40240.16 | 2.295 | 138531.66 | 2.56 | 178103.29 |
| 1.505 | 36555.53 | 1.77 | 33050.94 | 2.035 | 40694.72 | 2.3 | 148843.62 | 2.565 | 183138.42 |
| 1.51 | 35301.23 | 1.775 | 32452.79 | 2.04 | 41216.34 | 2.305 | 158921.75 | 2.57 | 188557.48 |
| 1.515 | 34008.65 | 1.78 | 31895.54 | 2.045 | 41804.78 | 2.31 | 168513.5 | 2.575 | 194315.2 |
| 1.52 | 32717.84 | 1.785 | 31386.44 | 2.05 | 42457.1 | 2.315 | 177366.68 | 2.58 | 200346.85 |
| 1.525 | 31466.66 | 1.79 | 30931.83 | 2.055 | 43166.47 | 2.32 | 185240.58 | 2.585 | 206571.35 |
| 1.53 | 30289.43 | 1.795 | 30536.92 | 2.06 | 43922.44 | 2.325 | 191921.59 | 2.59 | 212892.74 |
| 1.535 | 29215.12 | 1.8 | 30204.89 | 2.065 | 44710.63 | 2.33 | 197236.65 | 2.595 | 219205.58 |
| 1.54 | 28268.04 | 1.805 | 29937.24 | 2.07 | 45512.54 | 2.335 | 201065.08 | 2.6 | 225401.17 |
| 1.545 | 27465.39 | 1.81 | 29730.61 | 2.075 | 46306.63 | 2.34 | 203346.69 | 2.605 | 231375.36 |
| 1.55 | 26821.11 | 1.815 | 29582.04 | 2.08 | 47068.35 | 2.345 | 204086.86 | 2.61 | 237035.7 |
| 1.555 | 26342.21 | 1.82 | 29484.69 | 2.085 | 47771.56 | 2.35 | 203351.8 | 2.615 | 242311.65 |
| 1.56 | 26032.1 | 1.825 | 29431.76 | 2.09 | 48390.77 | 2.355 | 201274.66 | 2.62 | 247161.25 |

| | | | | | | | | | |
|---|---|---|---|---|---|---|---|---|---|
| 2.625 | 251580.08 | 2.89 | 52136.66 | 3.155 | 23088.03 | 3.42 | 3100.1 | 3.685 | 2357.52 |
| 2.63 | 255602.8 | 2.895 | 50806.32 | 3.16 | 23619.14 | 3.425 | 3073.2 | 3.69 | 2348.93 |
| 2.635 | 259308.61 | 2.9 | 49408.05 | 3.165 | 24186.59 | 3.43 | 3047.75 | 3.695 | 2340.41 |
| 2.64 | 262816.14 | 2.905 | 47942.84 | 3.17 | 24745.22 | 3.435 | 3023.38 | 3.7 | 2331.99 |
| 2.645 | 266279.62 | 2.91 | 46421.62 | 3.175 | 25250.36 | 3.44 | 3000.01 | 3.705 | 2323.65 |
| 2.65 | 269876.44 | 2.915 | 44863.69 | 3.18 | 25659.12 | 3.445 | 2977.56 | 3.71 | 2315.4 |
| 2.655 | 273793.91 | 2.92 | 43293.39 | 3.185 | 25933.59 | 3.45 | 2955.94 | 3.715 | 2307.11 |
| 2.66 | 278212.83 | 2.925 | 41738.92 | 3.19 | 26042.4 | 3.455 | 2935.13 | 3.72 | 2299.02 |
| 2.665 | 283285.26 | 2.93 | 40233.52 | 3.195 | 25962.24 | 3.46 | 2915.04 | 3.725 | 2291.02 |
| 2.67 | 289117.79 | 2.935 | 38809.14 | 3.2 | 25678.99 | 3.465 | 2895.63 | 3.73 | 2283.06 |
| 2.675 | 295751.34 | 2.94 | 37499.76 | 3.205 | 25188.13 | 3.47 | 2876.46 | 3.735 | 2275.21 |
| 2.68 | 303146.69 | 2.945 | 36335.5 | 3.21 | 24494.7 | 3.475 | 2858.33 | 3.74 | 2267.43 |
| 2.685 | 311175.58 | 2.95 | 35344.3 | 3.215 | 23613.03 | 3.48 | 2840.71 | 3.745 | 2259.71 |
| 2.69 | 319618.37 | 2.955 | 34548.7 | 3.22 | 22565.49 | 3.485 | 2823.58 | 3.75 | 2252.06 |
| 2.695 | 328167.51 | 2.96 | 33965.53 | 3.225 | 21379.5 | 3.49 | 2806.9 | 3.755 | 2244.46 |
| 2.7 | 336442.62 | 2.965 | 33605.45 | 3.23 | 20088 | 3.495 | 2790.65 | 3.76 | 2236.93 |
| 2.705 | 344007.31 | 2.97 | 33470.53 | 3.235 | 18725.43 | 3.5 | 2774.75 | 3.765 | 2229.39 |
| 2.71 | 350399.35 | 2.975 | 33554.67 | 3.24 | 17327.02 | 3.505 | 2759.29 | 3.77 | 2221.98 |
| 2.715 | 355160.08 | 2.98 | 33843.7 | 3.245 | 15926.48 | 3.51 | 2744.19 | 3.775 | 2214.64 |
| 2.72 | 357864.62 | 2.985 | 34315.74 | 3.25 | 14554.19 | 3.515 | 2729.32 | 3.78 | 2207.34 |
| 2.725 | 358154.98 | 2.99 | 34941.89 | 3.255 | 13236.44 | 3.52 | 2714.87 | 3.785 | 2200.04 |
| 2.73 | 355764.61 | 2.995 | 35686.49 | 3.26 | 11994.45 | 3.525 | 2700.79 | 3.79 | 2192.86 |
| 2.735 | 350541.09 | 3 | 36509.13 | 3.265 | 10844.01 | 3.53 | 2687.02 | 3.795 | 2185.74 |
| 2.74 | 342457.6 | 3.005 | 37367.78 | 3.27 | 9795.52 | 3.535 | 2673.53 | 3.8 | 2178.67 |
| 2.745 | 331615.75 | 3.01 | 38216.69 | 3.275 | 8854.33 | 3.54 | 2660.32 | 3.805 | 2171.64 |
| 2.75 | 318238.46 | 3.015 | 39011.87 | 3.28 | 8021.27 | 3.545 | 2647.37 | 3.81 | 2164.67 |
| 2.755 | 302656.64 | 3.02 | 39711.15 | 3.285 | 7293.34 | 3.55 | 2634.68 | 3.815 | 2157.74 |
| 2.76 | 285287.01 | 3.025 | 40276.07 | 3.29 | 6664.76 | 3.555 | 2622.24 | 3.82 | 2150.86 |
| 2.765 | 266605.22 | 3.03 | 40673.83 | 3.295 | 6127.62 | 3.56 | 2610.04 | 3.825 | 2144.03 |
| 2.77 | 247115.57 | 3.035 | 40878.23 | 3.3 | 5672.58 | 3.565 | 2598.06 | 3.83 | 2137.25 |
| 2.775 | 227323.43 | 3.04 | 40870.56 | 3.305 | 5290.04 | 3.57 | 2586.3 | 3.835 | 2130.24 |
| 2.78 | 207707.18 | 3.045 | 40640.35 | 3.31 | 4970.11 | 3.575 | 2574.75 | 3.84 | 2123.6 |
| 2.785 | 188695.42 | 3.05 | 40184.73 | 3.315 | 4703.42 | 3.58 | 2563.4 | 3.845 | 2117 |
| 2.79 | 170651.97 | 3.055 | 39510.38 | 3.32 | 4481.29 | 3.585 | 2552.23 | 3.85 | 2110.44 |
| 2.795 | 153862.13 | 3.06 | 38630.05 | 3.325 | 4295.5 | 3.59 | 2541.24 | 3.855 | 2103.91 |
| 2.8 | 138529.71 | 3.065 | 37564.19 | 3.33 | 4140.33 | 3.595 | 2530.15 | 3.86 | 2097.43 |
| 2.805 | 124777.34 | 3.07 | 36339.5 | 3.335 | 4009.46 | 3.6 | 2519.55 | 3.865 | 2090.99 |
| 2.81 | 112653.26 | 3.075 | 34987.38 | 3.34 | 3898.12 | 3.605 | 2509.09 | 3.87 | 2084.59 |
| 2.815 | 102140.56 | 3.08 | 33544.54 | 3.345 | 3802.41 | 3.61 | 2498.76 | 3.875 | 2078.23 |
| 2.82 | 93167.67 | 3.085 | 32048.92 | 3.35 | 3719.18 | 3.615 | 2488.56 | 3.88 | 2071.92 |
| 2.825 | 85623 | 3.09 | 30540.55 | 3.355 | 3645.92 | 3.62 | 2478.49 | 3.885 | 2065.65 |
| 2.83 | 79366.76 | 3.095 | 29060.61 | 3.36 | 3580.7 | 3.625 | 2468.54 | 3.89 | 2059.43 |
| 2.835 | 74241.29 | 3.1 | 27647.99 | 3.365 | 3521.97 | 3.63 | 2458.71 | 3.895 | 2052.73 |
| 2.84 | 70084.08 | 3.105 | 26339.45 | 3.37 | 3468.58 | 3.635 | 2448.99 | 3.9 | 2046.68 |
| 2.845 | 66731.61 | 3.11 | 25168.19 | 3.375 | 3419.61 | 3.64 | 2439.38 | 3.905 | 2040.67 |
| 2.85 | 64030.44 | 3.115 | 24162.32 | 3.38 | 3374.29 | 3.645 | 2429.88 | 3.91 | 2034.69 |
| 2.855 | 61837.8 | 3.12 | 23344.03 | 3.385 | 3332.28 | 3.65 | 2420.49 | 3.915 | 2028.75 |
| 2.86 | 60026.98 | 3.125 | 22728.52 | 3.39 | 3292.29 | 3.655 | 2411.2 | 3.92 | 2022.84 |
| 2.865 | 58487.23 | 3.13 | 22322.53 | 3.395 | 3255.45 | 3.66 | 2402.01 | 3.925 | 2016.97 |
| 2.87 | 57124.56 | 3.135 | 22124.65 | 3.4 | 3220.98 | 3.665 | 2392.85 | 3.93 | 2011.12 |
| 2.875 | 55861.94 | 3.14 | 22124.76 | 3.405 | 3188.39 | 3.67 | 2383.88 | 3.935 | 2005.31 |
| 2.88 | 54638.42 | 3.145 | 22304.34 | 3.41 | 3157.47 | 3.675 | 2375 | 3.94 | 1999.54 |
| 2.885 | 53407.41 | 3.15 | 22636.65 | 3.415 | 3128.08 | 3.68 | 2366.22 | 3.945 | 1993.79 |

| | | | | | | | |
|---|---|---|---|---|---|---|---|
| 3.95 | 1988.07 | 4.215 | 1722.87 | 4.48 | 1513.4 | 4.745 | 1342.7 |
| 3.955 | 1982.38 | 4.22 | 1718.47 | 4.485 | 1509.88 | 4.75 | 1339.78 |
| 3.96 | 1976.72 | 4.225 | 1714.1 | 4.49 | 1506.36 | 4.755 | 1336.87 |
| 3.965 | 1971.09 | 4.23 | 1709.73 | 4.495 | 1502.86 | 4.76 | 1333.98 |
| 3.97 | 1965.49 | 4.235 | 1705.39 | 4.5 | 1499.37 | 4.765 | 1331.09 |
| 3.975 | 1959.92 | 4.24 | 1701.04 | 4.505 | 1495.9 | 4.77 | 1328.21 |
| 3.98 | 1954.37 | 4.245 | 1696.74 | 4.51 | 1492.43 | 4.775 | 1325.34 |
| 3.985 | 1948.85 | 4.25 | 1692.44 | 4.515 | 1488.98 | 4.78 | 1322.48 |
| 3.99 | 1943.36 | 4.255 | 1688.17 | 4.52 | 1485.55 | 4.785 | 1319.63 |
| 3.995 | 1937.89 | 4.26 | 1683.91 | 4.525 | 1482.12 | 4.79 | 1316.79 |
| 4 | 1932.46 | 4.265 | 1679.67 | 4.53 | 1478.71 | 4.795 | 1313.96 |
| 4.005 | 1927.05 | 4.27 | 1675.45 | 4.535 | 1475.31 | 4.8 | 1311.14 |
| 4.01 | 1921.66 | 4.275 | 1671.24 | 4.54 | 1471.92 | 4.805 | 1308.33 |
| 4.015 | 1916.31 | 4.28 | 1667.05 | 4.545 | 1468.55 | 4.81 | 1305.53 |
| 4.02 | 1910.98 | 4.285 | 1662.88 | 4.55 | 1465.19 | 4.815 | 1302.74 |
| 4.025 | 1905.68 | 4.29 | 1658.73 | 4.555 | 1461.84 | 4.82 | 1299.96 |
| 4.03 | 1900.4 | 4.295 | 1654.6 | 4.56 | 1458.5 | 4.825 | 1297.18 |
| 4.035 | 1895.11 | 4.3 | 1650.37 | 4.565 | 1455.18 | 4.83 | 1294.42 |
| 4.04 | 1889.91 | 4.305 | 1646.29 | 4.57 | 1451.86 | 4.835 | 1291.66 |
| 4.045 | 1884.72 | 4.31 | 1642.19 | 4.575 | 1448.56 | 4.84 | 1288.92 |
| 4.05 | 1879.57 | 4.315 | 1638.16 | 4.58 | 1445.27 | 4.845 | 1286.18 |
| 4.055 | 1874.44 | 4.32 | 1634.14 | 4.585 | 1442 | 4.85 | 1283.45 |
| 4.06 | 1869.34 | 4.325 | 1630.14 | 4.59 | 1438.73 | 4.855 | 1280.73 |
| 4.065 | 1864.26 | 4.33 | 1626.16 | 4.595 | 1435.48 | 4.86 | 1278.02 |
| 4.07 | 1859.13 | 4.335 | 1622.19 | 4.6 | 1432.23 | 4.865 | 1275.32 |
| 4.075 | 1854.12 | 4.34 | 1618.23 | 4.605 | 1429 | 4.87 | 1272.63 |
| 4.08 | 1849.12 | 4.345 | 1614.29 | 4.61 | 1425.78 | 4.875 | 1269.94 |
| 4.085 | 1844.16 | 4.35 | 1610.37 | 4.615 | 1422.57 | 4.88 | 1267.27 |
| 4.09 | 1839.23 | 4.355 | 1606.46 | 4.62 | 1419.37 | 4.885 | 1264.6 |
| 4.095 | 1834.31 | 4.36 | 1602.56 | 4.625 | 1416.18 | 4.89 | 1261.95 |
| 4.1 | 1829.42 | 4.365 | 1598.68 | 4.63 | 1413.01 | 4.895 | 1259.3 |
| 4.105 | 1824.55 | 4.37 | 1594.82 | 4.635 | 1409.84 | 4.9 | 1256.66 |
| 4.11 | 1819.7 | 4.375 | 1590.97 | 4.64 | 1406.68 | 4.905 | 1254.03 |
| 4.115 | 1814.88 | 4.38 | 1587.13 | 4.645 | 1403.54 | 4.91 | 1251.4 |
| 4.12 | 1810.08 | 4.385 | 1583.31 | 4.65 | 1400.4 | 4.915 | 1248.79 |
| 4.125 | 1805.3 | 4.39 | 1579.5 | 4.655 | 1397.27 | 4.92 | 1246.18 |
| 4.13 | 1800.54 | 4.395 | 1575.7 | 4.66 | 1394.16 | 4.925 | 1243.59 |
| 4.135 | 1795.8 | 4.4 | 1571.92 | 4.665 | 1391.05 | 4.93 | 1241 |
| 4.14 | 1791.09 | 4.405 | 1568.16 | 4.67 | 1387.95 | 4.935 | 1238.42 |
| 4.145 | 1786.39 | 4.41 | 1564.4 | 4.675 | 1384.86 | 4.94 | 1235.84 |
| 4.15 | 1781.72 | 4.415 | 1560.67 | 4.68 | 1381.79 | 4.945 | 1233.28 |
| 4.155 | 1777.07 | 4.42 | 1556.94 | 4.685 | 1378.72 | 4.95 | 1230.72 |
| 4.16 | 1772.45 | 4.425 | 1553.23 | 4.69 | 1375.66 | 4.955 | 1228.17 |
| 4.165 | 1767.79 | 4.43 | 1549.54 | 4.695 | 1372.62 | 4.96 | 1225.64 |
| 4.17 | 1763.21 | 4.435 | 1545.86 | 4.7 | 1369.58 | 4.965 | 1223.1 |
| 4.175 | 1758.65 | 4.44 | 1542.2 | 4.705 | 1366.55 | 4.97 | 1220.58 |
| 4.18 | 1754.12 | 4.445 | 1538.55 | 4.71 | 1363.54 | 4.975 | 1218.06 |
| 4.185 | 1749.6 | 4.45 | 1534.92 | 4.715 | 1360.53 | 4.98 | 1215.56 |
| 4.19 | 1745.1 | 4.455 | 1531.24 | 4.72 | 1357.54 | 4.985 | 1213.05 |
| 4.195 | 1740.62 | 4.46 | 1527.65 | 4.725 | 1354.56 | 4.99 | 1210.56 |
| 4.2 | 1736.15 | 4.465 | 1524.07 | 4.73 | 1351.59 | 4.995 | 1208.08 |
| 4.205 | 1731.71 | 4.47 | 1520.5 | 4.735 | 1348.56 | 5 | 1205.6 |
| 4.21 | 1727.28 | 4.475 | 1516.95 | 4.74 | 1345.63 | | |

**$Te^{2+}$ : Energy vs DR cross section**

| Energy (eV) | Barn |
|---|---|
| 0 | 766008.6 |
| 0.005 | 815515.71 |
| 0.01 | 864987.12 |
| 0.015 | 913740.43 |
| 0.02 | 961039.04 |
| 0.025 | 1.00611E6 |
| 0.03 | 1.04817E6 |
| 0.035 | 1.08645E6 |
| 0.04 | 1.12022E6 |
| 0.045 | 1.14882E6 |
| 0.05 | 1.17168E6 |
| 0.055 | 1.18835E6 |
| 0.06 | 1.19852E6 |
| 0.065 | 1.20204E6 |
| 0.07 | 1.19889E6 |
| 0.075 | 1.18926E6 |
| 0.08 | 1.17346E6 |
| 0.085 | 1.15195E6 |
| 0.09 | 1.12535E6 |
| 0.095 | 1.09435E6 |
| 0.1 | 1.05976E6 |
| 0.105 | 1.02242E6 |
| 0.11 | 983214.02 |
| 0.115 | 943035.93 |
| 0.12 | 902754.54 |
| 0.125 | 863200.25 |
| 0.13 | 825145.46 |
| 0.135 | 789288.87 |
| 0.14 | 756244.18 |
| 0.145 | 726531.49 |
| 0.15 | 700571.01 |
| 0.155 | 678679.02 |
| 0.16 | 661066.33 |
| 0.165 | 647834.94 |
| 0.17 | 638980.15 |
| 0.175 | 634389.56 |
| 0.18 | 633844.97 |
| 0.185 | 637025.68 |
| 0.19 | 643512.89 |
| 0.195 | 652796.71 |
| 0.2 | 664286.22 |
| 0.205 | 677322.53 |
| 0.21 | 691195.04 |
| 0.215 | 705161.35 |
| 0.22 | 718469.26 |
| 0.225 | 730381.67 |
| 0.23 | 740202.09 |
| 0.235 | 747299.5 |
| 0.24 | 751131.91 |
| 0.245 | 751267.12 |
| 0.25 | 747398.03 |
| 0.255 | 739353.54 |
| 0.26 | 727102.36 |
| 0.265 | 710750.17 |
| 0.27 | 690532.28 |
| 0.275 | 666797.69 |
| 0.28 | 639990.3 |
| 0.285 | 610625.82 |
| 0.29 | 579267.63 |
| 0.295 | 546500.84 |
| 0.3 | 512908.65 |
| 0.305 | 479050.07 |
| 0.31 | 445441.18 |
| 0.315 | 412541.29 |
| 0.32 | 380742 |
| 0.325 | 350361.92 |
| 0.33 | 321644.93 |
| 0.335 | 294761.84 |
| 0.34 | 269816.15 |
| 0.345 | 246850.27 |
| 0.35 | 225854.88 |
| 0.355 | 206778.19 |
| 0.36 | 189535.11 |
| 0.365 | 174016.42 |
| 0.37 | 160097.13 |
| 0.375 | 147643.55 |
| 0.38 | 136519.26 |
| 0.385 | 126589.77 |
| 0.39 | 117726.09 |
| 0.395 | 109807.5 |
| 0.4 | 102722.51 |
| 0.405 | 96370.25 |
| 0.41 | 90660.37 |
| 0.415 | 85512.71 |
| 0.42 | 80857.24 |
| 0.425 | 76632.47 |
| 0.43 | 72785.27 |
| 0.435 | 69269.72 |
| 0.44 | 66046.21 |
| 0.445 | 63080.82 |
| 0.45 | 60344.04 |
| 0.455 | 57810.7 |
| 0.46 | 55459.05 |
| 0.465 | 53270.23 |
| 0.47 | 51227.88 |
| 0.475 | 49317.74 |
| 0.48 | 47527.38 |
| 0.485 | 45845.74 |
| 0.49 | 44263.52 |
| 0.495 | 42772.04 |
| 0.5 | 41363.75 |
| 0.505 | 40031.99 |
| 0.51 | 38770.75 |
| 0.515 | 37574.67 |
| 0.52 | 36438.92 |
| 0.525 | 35359.15 |
| 0.53 | 34331.41 |
| 0.535 | 33352.13 |
| 0.54 | 32418.06 |
| 0.545 | 31526.23 |
| 0.55 | 30673.94 |
| 0.555 | 29858.69 |
| 0.56 | 29078.22 |
| 0.565 | 28330.44 |
| 0.57 | 27613.41 |
| 0.575 | 26925.35 |
| 0.58 | 26264.62 |
| 0.585 | 25629.71 |
| 0.59 | 25019.18 |
| 0.595 | 24431.75 |
| 0.6 | 23866.18 |
| 0.605 | 23321.33 |
| 0.61 | 22796.16 |
| 0.615 | 22289.68 |
| 0.62 | 21800.95 |
| 0.625 | 21329.12 |
| 0.63 | 20873.38 |
| 0.635 | 20432.95 |
| 0.64 | 20007.15 |
| 0.645 | 19595.29 |
| 0.65 | 19196.75 |
| 0.655 | 18810.91 |
| 0.66 | 18437.25 |
| 0.665 | 18075.22 |
| 0.67 | 17724.32 |
| 0.675 | 17384.08 |
| 0.68 | 17054.07 |
| 0.685 | 16733.86 |
| 0.69 | 16423.05 |
| 0.695 | 16121.27 |
| 0.7 | 15828.14 |
| 0.705 | 15543.36 |
| 0.71 | 15266.57 |
| 0.715 | 14997.48 |
| 0.72 | 14735.8 |
| 0.725 | 14481.25 |
| 0.73 | 14233.56 |
| 0.735 | 13992.48 |
| 0.74 | 13757.86 |
| 0.745 | 13529.32 |
| 0.75 | 13306.71 |
| 0.755 | 13089.83 |
| 0.76 | 12878.47 |
| 0.765 | 12672.44 |
| 0.77 | 12471.56 |
| 0.775 | 12275.66 |
| 0.78 | 12084.57 |
| 0.785 | 11898.14 |
| 0.79 | 11716.2 |
| 0.795 | 11538.63 |
| 0.8 | 11365.26 |
| 0.805 | 11195.98 |
| 0.81 | 11030.66 |
| 0.815 | 10869.16 |
| 0.82 | 10711.38 |
| 0.825 | 10557.19 |
| 0.83 | 10406.5 |
| 0.835 | 10259.18 |
| 0.84 | 10115.16 |
| 0.845 | 9974.32 |
| 0.85 | 9836.58 |
| 0.855 | 9701.84 |
| 0.86 | 9570.02 |
| 0.865 | 9441.03 |
| 0.87 | 9314.8 |
| 0.875 | 9191.25 |
| 0.88 | 9070.31 |
| 0.885 | 8951.9 |
| 0.89 | 8835.95 |
| 0.895 | 8722.4 |
| 0.9 | 8611.18 |
| 0.905 | 8502.24 |
| 0.91 | 8395.5 |
| 0.915 | 8290.92 |
| 0.92 | 8188.44 |
| 0.925 | 8088.06 |
| 0.93 | 7989.63 |
| 0.935 | 7893.14 |
| 0.94 | 7798.55 |
| 0.945 | 7705.8 |
| 0.95 | 7614.86 |
| 0.955 | 7525.67 |
| 0.96 | 7438.2 |
| 0.965 | 7352.41 |
| 0.97 | 7268.25 |
| 0.975 | 7185.69 |
| 0.98 | 7104.68 |
| 0.985 | 7025.2 |
| 0.99 | 6947.23 |
| 0.995 | 6870.7 |
| 1 | 6795.59 |
| 1.005 | 6721.87 |
| 1.01 | 6649.52 |
| 1.015 | 6578.49 |
| 1.02 | 6508.77 |
| 1.025 | 6440.33 |
| 1.03 | 6373.14 |
| 1.035 | 6307.17 |
| 1.04 | 6242.39 |
| 1.045 | 6178.79 |
| 1.05 | 6116.34 |
| 1.055 | 6055.02 |
| 1.06 | 5994.81 |
| 1.065 | 5935.68 |
| 1.07 | 5877.61 |
| 1.075 | 5820.59 |
| 1.08 | 5764.6 |
| 1.085 | 5709.61 |
| 1.09 | 5655.61 |
| 1.095 | 5602.59 |
| 1.1 | 5550.52 |
| 1.105 | 5499.4 |
| 1.11 | 5449.19 |
| 1.115 | 5399.9 |
| 1.12 | 5351.51 |
| 1.125 | 5303.99 |
| 1.13 | 5257.4 |
| 1.135 | 5211.62 |
| 1.14 | 5166.69 |
| 1.145 | 5122.59 |
| 1.15 | 5079.32 |
| 1.155 | 5036.85 |
| 1.16 | 4995.2 |
| 1.165 | 4954.33 |
| 1.17 | 4914.26 |
| 1.175 | 4874.96 |
| 1.18 | 4836.43 |
| 1.185 | 4798.66 |
| 1.19 | 4761.65 |
| 1.195 | 4725.39 |
| 1.2 | 4689.87 |
| 1.205 | 4655.11 |
| 1.21 | 4621.07 |
| 1.215 | 4587.77 |
| 1.22 | 4555.27 |
| 1.225 | 4523.44 |
| 1.23 | 4492.33 |
| 1.235 | 4461.96 |
| 1.24 | 4432.31 |
| 1.245 | 4403.4 |
| 1.25 | 4375.22 |
| 1.255 | 4347.77 |
| 1.26 | 4321.05 |
| 1.265 | 4295.08 |
| 1.27 | 4269.86 |
| 1.275 | 4245.39 |
| 1.28 | 4221.69 |
| 1.285 | 4198.76 |
| 1.29 | 4176.61 |

| | | | | | | | | | |
|---|---|---|---|---|---|---|---|---|---|
| 1.295 | 4155.26 | 1.56 | 8144.23 | 1.825 | 3799.5 | 2.09 | 1770.28 | 2.355 | 1230.04 |
| 1.3 | 4134.71 | 1.565 | 8657.73 | 1.83 | 3693.31 | 2.095 | 1758 | 2.36 | 1217.04 |
| 1.305 | 4115 | 1.57 | 9215.05 | 1.835 | 3596.54 | 2.1 | 1746.02 | 2.365 | 1204.9 |
| 1.31 | 4096.12 | 1.575 | 9814.99 | 1.84 | 3507.81 | 2.105 | 1734.32 | 2.37 | 1193.73 |
| 1.315 | 4078.11 | 1.58 | 10455.02 | 1.845 | 3425.9 | 2.11 | 1722.9 | 2.375 | 1133.12 |
| 1.32 | 4060.98 | 1.585 | 11131.16 | 1.85 | 3349.74 | 2.115 | 1711.74 | 2.38 | 1132.17 |
| 1.325 | 4044.77 | 1.59 | 11837.56 | 1.855 | 3278.42 | 2.12 | 1700.84 | 2.385 | 1131.37 |
| 1.33 | 4029.49 | 1.595 | 12566.87 | 1.86 | 3211.13 | 2.125 | 1690.19 | 2.39 | 1130.71 |
| 1.335 | 4015.18 | 1.6 | 13310.01 | 1.865 | 3147.22 | 2.13 | 1679.78 | 2.395 | 1130.2 |
| 1.34 | 4001.87 | 1.605 | 14056.27 | 1.87 | 3086.13 | 2.135 | 1669.6 | 2.4 | 1129.83 |
| 1.345 | 3989.59 | 1.61 | 14793.56 | 1.875 | 3027.41 | 2.14 | 1659.64 | 2.405 | 1129.62 |
| 1.35 | 3978.4 | 1.615 | 15508.68 | 1.88 | 2971.09 | 2.145 | 1649.91 | 2.41 | 1129.56 |
| 1.355 | 3968.32 | 1.62 | 16187.68 | 1.885 | 2916.24 | 2.15 | 1640.39 | 2.415 | 1129.65 |
| 1.36 | 3959.42 | 1.625 | 16816.32 | 1.89 | 2862.98 | 2.155 | 1631.07 | 2.42 | 1129.9 |
| 1.365 | 3951.76 | 1.63 | 17380.57 | 1.895 | 2811.2 | 2.16 | 1621.96 | 2.425 | 1130.31 |
| 1.37 | 3945.38 | 1.635 | 17867.19 | 1.9 | 2760.84 | 2.165 | 1613.05 | 2.43 | 1130.87 |
| 1.375 | 3940.36 | 1.64 | 18264.26 | 1.905 | 2711.88 | 2.17 | 1604.33 | 2.435 | 1131.6 |
| 1.38 | 3936.78 | 1.645 | 18561.66 | 1.91 | 2664.32 | 2.175 | 1595.8 | 2.44 | 1132.5 |
| 1.385 | 3934.71 | 1.65 | 18751.53 | 1.915 | 2618.2 | 2.18 | 1587.46 | 2.445 | 1133.57 |
| 1.39 | 3934.26 | 1.655 | 18828.68 | 1.92 | 2573.55 | 2.185 | 1579.29 | 2.45 | 1134.81 |
| 1.395 | 3935.53 | 1.66 | 18790.81 | 1.925 | 2530.43 | 2.19 | 1571.29 | 2.455 | 1136.22 |
| 1.4 | 3938.64 | 1.665 | 18638.57 | 1.93 | 2488.86 | 2.195 | 1563.46 | 2.46 | 1137.82 |
| 1.405 | 3943.72 | 1.67 | 18375.56 | 1.935 | 2448.88 | 2.2 | 1556.08 | 2.465 | 1139.59 |
| 1.41 | 3950.91 | 1.675 | 18008.22 | 1.94 | 2410.51 | 2.205 | 1548.6 | 2.47 | 1141.55 |
| 1.415 | 3960.39 | 1.68 | 17553.01 | 1.945 | 2373.74 | 2.21 | 1541.26 | 2.475 | 1143.7 |
| 1.42 | 3972.34 | 1.685 | 16998.18 | 1.95 | 2338.56 | 2.215 | 1534.04 | 2.48 | 1146.03 |
| 1.425 | 3986.97 | 1.69 | 16379.04 | 1.955 | 2304.96 | 2.22 | 1526.92 | 2.485 | 1148.59 |
| 1.43 | 4004.54 | 1.695 | 15701.71 | 1.96 | 2272.87 | 2.225 | 1519.88 | 2.49 | 1151.3 |
| 1.435 | 4025.3 | 1.7 | 14980.35 | 1.965 | 2242.26 | 2.23 | 1512.89 | 2.495 | 1154.2 |
| 1.44 | 4049.59 | 1.705 | 14229.16 | 1.97 | 2213.05 | 2.235 | 1505.9 | 2.5 | 1157.28 |
| 1.445 | 4077.77 | 1.71 | 13461.81 | 1.975 | 2185.18 | 2.24 | 1498.89 | 2.505 | 1160.53 |
| 1.45 | 4110.21 | 1.715 | 12691.1 | 1.98 | 2158.58 | 2.245 | 1491.78 | 2.51 | 1163.96 |
| 1.455 | 4147.42 | 1.72 | 11928.55 | 1.985 | 2133.17 | 2.25 | 1484.53 | 2.515 | 1167.56 |
| 1.46 | 4189.93 | 1.725 | 11184.19 | 1.99 | 2108.87 | 2.255 | 1477.08 | 2.52 | 1171.32 |
| 1.465 | 4238.35 | 1.73 | 10466.39 | 1.995 | 2085.6 | 2.26 | 1469.34 | 2.525 | 1175.23 |
| 1.47 | 4293.42 | 1.735 | 9781.84 | 2 | 2063.31 | 2.265 | 1461.26 | 2.53 | 1179.29 |
| 1.475 | 4355.96 | 1.74 | 9135.54 | 2.005 | 2041.98 | 2.27 | 1452.74 | 2.535 | 1183.48 |
| 1.48 | 4426.92 | 1.745 | 8530.9 | 2.01 | 2021.43 | 2.275 | 1443.73 | 2.54 | 1187.82 |
| 1.485 | 4507.38 | 1.75 | 7969.88 | 2.015 | 2001.65 | 2.28 | 1434.14 | 2.545 | 1192.36 |
| 1.49 | 4598.61 | 1.755 | 7453.17 | 2.02 | 1982.59 | 2.285 | 1423.93 | 2.55 | 1196.97 |
| 1.495 | 4702.03 | 1.76 | 6980.38 | 2.025 | 1964.2 | 2.29 | 1413.04 | 2.555 | 1201.7 |
| 1.5 | 4819.26 | 1.765 | 6550.26 | 2.03 | 1946.43 | 2.295 | 1401.46 | 2.56 | 1206.57 |
| 1.505 | 4952.12 | 1.77 | 6160.9 | 2.035 | 1929.24 | 2.3 | 1389.16 | 2.565 | 1211.56 |
| 1.51 | 5102.65 | 1.775 | 5809.92 | 2.04 | 1912.6 | 2.305 | 1376.19 | 2.57 | 1216.76 |
| 1.515 | 5273.1 | 1.78 | 5494.6 | 2.045 | 1896.47 | 2.31 | 1362.56 | 2.575 | 1222.03 |
| 1.52 | 5465.94 | 1.785 | 5212.07 | 2.05 | 1880.81 | 2.315 | 1348.36 | 2.58 | 1227.44 |
| 1.525 | 5683.81 | 1.79 | 4959.4 | 2.055 | 1865.61 | 2.32 | 1333.69 | 2.585 | 1232.97 |
| 1.53 | 5929.49 | 1.795 | 4733.67 | 2.06 | 1850.93 | 2.325 | 1318.67 | 2.59 | 1238.62 |
| 1.535 | 6205.9 | 1.8 | 4532.09 | 2.065 | 1836.58 | 2.33 | 1303.44 | 2.595 | 1244.39 |
| 1.54 | 6515.92 | 1.805 | 4351.99 | 2.07 | 1822.62 | 2.335 | 1288.17 | 2.6 | 1250.28 |
| 1.545 | 6862.37 | 1.81 | 4190.88 | 2.075 | 1809.02 | 2.34 | 1273.03 | 2.605 | 1256.25 |
| 1.55 | 7247.85 | 1.815 | 4046.46 | 2.08 | 1795.78 | 2.345 | 1258.19 | 2.61 | 1262.31 |
| 1.555 | 7674.58 | 1.82 | 3916.64 | 2.085 | 1782.87 | 2.35 | 1243.8 | 2.615 | 1268.43 |

| | | | | | | | | | |
|---|---|---|---|---|---|---|---|---|---|
| 2.62 | 1274.6 | 2.885 | 1299.68 | 3.15 | 1483.37 | 3.415 | 6071.91 | 3.68 | 1578.4 |
| 2.625 | 1280.79 | 2.89 | 1292.77 | 3.155 | 1508.64 | 3.42 | 5865.84 | 3.685 | 1568.35 |
| 2.63 | 1286.99 | 2.895 | 1285.87 | 3.16 | 1536.11 | 3.425 | 5666.6 | 3.69 | 1562.9 |
| 2.635 | 1293.16 | 2.9 | 1279.01 | 3.165 | 1566.19 | 3.43 | 5476.43 | 3.695 | 1561.93 |
| 2.64 | 1299.3 | 2.905 | 1272.23 | 3.17 | 1599.41 | 3.435 | 5297.05 | 3.7 | 1568.51 |
| 2.645 | 1305.39 | 2.91 | 1265.55 | 3.175 | 1636.37 | 3.44 | 5129.74 | 3.705 | 1576.39 |
| 2.65 | 1311.4 | 2.915 | 1258.99 | 3.18 | 1677.76 | 3.445 | 4975.28 | 3.71 | 1588.03 |
| 2.655 | 1317.32 | 2.92 | 1252.59 | 3.185 | 1724.33 | 3.45 | 4834.06 | 3.715 | 1603.01 |
| 2.66 | 1323.14 | 2.925 | 1246.36 | 3.19 | 1776.92 | 3.455 | 4706.08 | 3.72 | 1620.79 |
| 2.665 | 1328.85 | 2.93 | 1240.34 | 3.195 | 1836.43 | 3.46 | 4591.02 | 3.725 | 1640.73 |
| 2.67 | 1334.44 | 2.935 | 1234.54 | 3.2 | 1903.79 | 3.465 | 4488.25 | 3.73 | 1662.11 |
| 2.675 | 1339.88 | 2.94 | 1228.99 | 3.205 | 1979.98 | 3.47 | 4396.92 | 3.735 | 1684.08 |
| 2.68 | 1345.19 | 2.945 | 1223.71 | 3.21 | 2065.99 | 3.475 | 4315.96 | 3.74 | 1705.79 |
| 2.685 | 1350.34 | 2.95 | 1218.72 | 3.215 | 2162.81 | 3.48 | 4244.13 | 3.745 | 1726.21 |
| 2.69 | 1355.32 | 2.955 | 1214.03 | 3.22 | 2271.4 | 3.485 | 4181.14 | 3.75 | 1744.43 |
| 2.695 | 1360.13 | 2.96 | 1209.67 | 3.225 | 2305.47 | 3.49 | 4123.53 | 3.755 | 1759.5 |
| 2.7 | 1364.74 | 2.965 | 1205.66 | 3.23 | 2453.7 | 3.495 | 4070.7 | 3.76 | 1770.56 |
| 2.705 | 1369.15 | 2.97 | 1202.01 | 3.235 | 2614.84 | 3.5 | 4021.06 | 3.765 | 1776.87 |
| 2.71 | 1373.34 | 2.975 | 1198.74 | 3.24 | 2789.4 | 3.505 | 3973.07 | 3.77 | 1777.76 |
| 2.715 | 1377.28 | 2.98 | 1195.87 | 3.245 | 2977.87 | 3.51 | 3925.21 | 3.775 | 1772.78 |
| 2.72 | 1380.97 | 2.985 | 1193.42 | 3.25 | 3180.54 | 3.515 | 3876.05 | 3.78 | 1761.69 |
| 2.725 | 1384.39 | 2.99 | 1191.4 | 3.255 | 3397.46 | 3.52 | 3824.31 | 3.785 | 1744.44 |
| 2.73 | 1387.51 | 2.995 | 1189.83 | 3.26 | 3628.4 | 3.525 | 3768.86 | 3.79 | 1721.15 |
| 2.735 | 1390.31 | 3 | 1188.72 | 3.265 | 3872.82 | 3.53 | 3708.79 | 3.795 | 1692.21 |
| 2.74 | 1392.78 | 3.005 | 1188.1 | 3.27 | 4129.82 | 3.535 | 3643.42 | 3.8 | 1658.16 |
| 2.745 | 1394.89 | 3.01 | 1187.99 | 3.275 | 4398.07 | 3.54 | 3572.35 | 3.805 | 1619.7 |
| 2.75 | 1396.64 | 3.015 | 1188.4 | 3.28 | 4675.84 | 3.545 | 3495.41 | 3.81 | 1577.68 |
| 2.755 | 1398 | 3.02 | 1189.35 | 3.285 | 4960.92 | 3.55 | 3412.73 | 3.815 | 1533.01 |
| 2.76 | 1398.97 | 3.025 | 1190.87 | 3.29 | 5250.67 | 3.555 | 3324.69 | 3.82 | 1486.69 |
| 2.765 | 1399.52 | 3.03 | 1192.98 | 3.295 | 5542.01 | 3.56 | 3231.87 | 3.825 | 1439.69 |
| 2.77 | 1399.65 | 3.035 | 1195.69 | 3.3 | 5831.49 | 3.565 | 3135.06 | 3.83 | 1393 |
| 2.775 | 1399.36 | 3.04 | 1199.04 | 3.305 | 6115.3 | 3.57 | 3035.2 | 3.835 | 1347.52 |
| 2.78 | 1398.63 | 3.045 | 1203.06 | 3.31 | 6389.43 | 3.575 | 2933.33 | 3.84 | 1304.11 |
| 2.785 | 1397.46 | 3.05 | 1209.26 | 3.315 | 6649.72 | 3.58 | 2830.54 | 3.845 | 1263.52 |
| 2.79 | 1395.86 | 3.055 | 1214.89 | 3.32 | 6891.99 | 3.585 | 2727.92 | 3.85 | 1226.39 |
| 2.795 | 1393.83 | 3.06 | 1221.28 | 3.325 | 7112.21 | 3.59 | 2626.57 | 3.855 | 1193.26 |
| 2.8 | 1391.37 | 3.065 | 1228.44 | 3.33 | 7306.6 | 3.595 | 2527.39 | 3.86 | 1164.54 |
| 2.805 | 1388.48 | 3.07 | 1236.39 | 3.335 | 7471.79 | 3.6 | 2431.28 | 3.865 | 1140.57 |
| 2.81 | 1385.18 | 3.075 | 1245.15 | 3.34 | 7605.04 | 3.605 | 2339 | 3.87 | 1121.56 |
| 2.815 | 1381.49 | 3.08 | 1254.75 | 3.345 | 7704.07 | 3.61 | 2251.14 | 3.875 | 1107.65 |
| 2.82 | 1377.41 | 3.085 | 1265.18 | 3.35 | 7767.55 | 3.615 | 2168.19 | 3.88 | 1098.88 |
| 2.825 | 1372.96 | 3.09 | 1276.47 | 3.355 | 7794.88 | 3.62 | 2090.48 | 3.885 | 1095.23 |
| 2.83 | 1368.17 | 3.095 | 1288.61 | 3.36 | 7786.38 | 3.625 | 2018.23 | 3.89 | 1096.61 |
| 2.835 | 1363.05 | 3.1 | 1301.61 | 3.365 | 7743.08 | 3.63 | 1951.54 | 3.895 | 1102.86 |
| 2.84 | 1357.63 | 3.105 | 1315.47 | 3.37 | 7666.91 | 3.635 | 1890.44 | 3.9 | 1113.79 |
| 2.845 | 1351.93 | 3.11 | 1330.2 | 3.375 | 7560.49 | 3.64 | 1834.9 | 3.905 | 1129.15 |
| 2.85 | 1345.98 | 3.115 | 1345.79 | 3.38 | 7427.06 | 3.645 | 1784.85 | 3.91 | 1148.66 |
| 2.855 | 1339.8 | 3.12 | 1362.28 | 3.385 | 7270.32 | 3.65 | 1740.14 | 3.915 | 1172.04 |
| 2.86 | 1333.43 | 3.125 | 1379.67 | 3.39 | 7094.32 | 3.655 | 1700.68 | 3.92 | 1198.94 |
| 2.865 | 1326.89 | 3.13 | 1398.04 | 3.395 | 6903.29 | 3.66 | 1666.35 | 3.925 | 1229.08 |
| 2.87 | 1320.22 | 3.135 | 1417.45 | 3.4 | 6701.49 | 3.665 | 1637.04 | 3.93 | 1262.15 |
| 2.875 | 1313.44 | 3.14 | 1438.02 | 3.405 | 6493.16 | 3.67 | 1612.67 | 3.935 | 1297.94 |
| 2.88 | 1306.58 | 3.145 | 1459.92 | 3.41 | 6282.08 | 3.675 | 1593.15 | 3.94 | 1336.25 |

| | | | | | | | | | |
|---|---|---|---|---|---|---|---|---|---|
| 3.945 | 1376.97 | 4.21 | 4324.53 | 4.475 | 1551.09 | 4.74 | 904.94 | 5.005 | 2959.73 |
| 3.95 | 1420.08 | 4.215 | 4306.98 | 4.48 | 1449.64 | 4.745 | 956.09 | 5.01 | 2909.85 |
| 3.955 | 1465.66 | 4.22 | 4301.15 | 4.485 | 1361 | 4.75 | 1010.64 | 5.015 | 2843.03 |
| 3.96 | 1513.85 | 4.225 | 4307.56 | 4.49 | 1283.35 | 4.755 | 1068.15 | 5.02 | 2761.27 |
| 3.965 | 1564.9 | 4.23 | 4327.01 | 4.495 | 1214.99 | 4.76 | 1128.47 | 5.025 | 2667.26 |
| 3.97 | 1619.08 | 4.235 | 4360.69 | 4.5 | 1154.56 | 4.765 | 1190.23 | 5.03 | 2563.84 |
| 3.975 | 1676.75 | 4.24 | 4410.27 | 4.505 | 1100.9 | 4.77 | 1252.96 | 5.035 | 2454.01 |
| 3.98 | 1738.18 | 4.245 | 4477.91 | 4.51 | 1053 | 4.775 | 1315.75 | 5.04 | 2340.72 |
| 3.985 | 1803.68 | 4.25 | 4566.19 | 4.515 | 1010.04 | 4.78 | 1377.61 | 5.045 | 2226.75 |
| 3.99 | 1873.48 | 4.255 | 4677.99 | 4.52 | 971.33 | 4.785 | 1437.44 | 5.05 | 2114.78 |
| 3.995 | 1947.72 | 4.26 | 4816.28 | 4.525 | 936.27 | 4.79 | 1494.13 | 5.055 | 2007.05 |
| 4 | 2026.8 | 4.265 | 4983.92 | 4.53 | 904.41 | 4.795 | 1546.53 | 5.06 | 1907.2 |
| 4.005 | 2110.07 | 4.27 | 5183.14 | 4.535 | 875.32 | 4.8 | 1593.56 | 5.065 | 1813.62 |
| 4.01 | 2197.7 | 4.275 | 5415.52 | 4.54 | 848.67 | 4.805 | 1634.39 | 5.07 | 1728.8 |
| 4.015 | 2289.49 | 4.28 | 5681.45 | 4.545 | 824.2 | 4.81 | 1667.85 | 5.075 | 1653.84 |
| 4.02 | 2385.29 | 4.285 | 5979.89 | 4.55 | 801.61 | 4.815 | 1693.47 | 5.08 | 1588.75 |
| 4.025 | 2484.92 | 4.29 | 6308.13 | 4.555 | 780.73 | 4.82 | 1710.84 | 5.085 | 1533.74 |
| 4.03 | 2588.3 | 4.295 | 6661.6 | 4.56 | 761.44 | 4.825 | 1719.89 | 5.09 | 1488.66 |
| 4.035 | 2695.45 | 4.3 | 7033.86 | 4.565 | 743.48 | 4.83 | 1720.85 | 5.095 | 1453.11 |
| 4.04 | 2806.48 | 4.305 | 7416.64 | 4.57 | 726.76 | 4.835 | 1714.27 | 5.1 | 1426.55 |
| 4.045 | 2921.63 | 4.31 | 7800.06 | 4.575 | 711.16 | 4.84 | 1701.01 | 5.105 | 1408.29 |
| 4.05 | 3041.2 | 4.315 | 8173 | 4.58 | 696.58 | 4.845 | 1682.23 | 5.11 | 1397.52 |
| 4.055 | 3165.49 | 4.32 | 8523.51 | 4.585 | 682.94 | 4.85 | 1659.31 | 5.115 | 1393.53 |
| 4.06 | 3294.75 | 4.325 | 8839.38 | 4.59 | 670.17 | 4.855 | 1633.82 | 5.12 | 1395.34 |
| 4.065 | 3429.09 | 4.33 | 9108.81 | 4.595 | 658.21 | 4.86 | 1607.44 | 5.125 | 1402.14 |
| 4.07 | 3568.32 | 4.335 | 9320.97 | 4.6 | 647.01 | 4.865 | 1581.92 | 5.13 | 1413.04 |
| 4.075 | 3711.23 | 4.34 | 9466.62 | 4.605 | 636.54 | 4.87 | 1558.98 | 5.135 | 1427.29 |
| 4.08 | 3858.38 | 4.345 | 9538.7 | 4.61 | 626.77 | 4.875 | 1540.3 | 5.14 | 1444.15 |
| 4.085 | 4007.77 | 4.35 | 9532.63 | 4.615 | 617.71 | 4.88 | 1527.45 | 5.145 | 1462.96 |
| 4.09 | 4157.05 | 4.355 | 9446.78 | 4.62 | 609.4 | 4.885 | 1521.84 | 5.15 | 1483.19 |
| 4.095 | 4304.07 | 4.36 | 9282.29 | 4.625 | 601.77 | 4.89 | 1524.73 | 5.155 | 1504.58 |
| 4.1 | 4446.1 | 4.365 | 9043.15 | 4.63 | 594.89 | 4.895 | 1537.19 | 5.16 | 1526.6 |
| 4.105 | 4580.2 | 4.37 | 8735.89 | 4.635 | 588.82 | 4.9 | 1560.08 | 5.165 | 1549.29 |
| 4.11 | 4703.29 | 4.375 | 8369.21 | 4.64 | 583.6 | 4.905 | 1594.04 | 5.17 | 1572.7 |
| 4.115 | 4812.44 | 4.38 | 7953.46 | 4.645 | 579.3 | 4.91 | 1639.46 | 5.175 | 1597.11 |
| 4.12 | 4904.99 | 4.385 | 7500.01 | 4.65 | 576.06 | 4.915 | 1696.44 | 5.18 | 1622.95 |
| 4.125 | 4978.74 | 4.39 | 7020.71 | 4.655 | 573.94 | 4.92 | 1764.8 | 5.185 | 1650.84 |
| 4.13 | 5032.12 | 4.395 | 6527.26 | 4.66 | 573.03 | 4.925 | 1844.02 | 5.19 | 1684.2 |
| 4.135 | 5064.34 | 4.4 | 6030.73 | 4.665 | 573.66 | 4.93 | 1933.18 | 5.195 | 1719.01 |
| 4.14 | 5075.42 | 4.405 | 5541.04 | 4.67 | 575.92 | 4.935 | 2030.99 | 5.2 | 1758.55 |
| 4.145 | 5066.23 | 4.41 | 5066.77 | 4.675 | 580.04 | 4.94 | 2135.77 | 5.205 | 1803.84 |
| 4.15 | 5038.44 | 4.415 | 4614.88 | 4.68 | 586.18 | 4.945 | 2245.41 | 5.21 | 1855.91 |
| 4.155 | 4994.44 | 4.42 | 4190.64 | 4.685 | 594.59 | 4.95 | 2357.45 | 5.215 | 1915.68 |
| 4.16 | 4937.16 | 4.425 | 3797.66 | 4.69 | 605.55 | 4.955 | 2469.17 | 5.22 | 1983.94 |
| 4.165 | 4869.92 | 4.43 | 3438.13 | 4.695 | 619.31 | 4.96 | 2577.51 | 5.225 | 2061.51 |
| 4.17 | 4796.23 | 4.435 | 3112.59 | 4.7 | 636.47 | 4.965 | 2679.41 | 5.23 | 2148.23 |
| 4.175 | 4719.61 | 4.44 | 2820.7 | 4.705 | 656.36 | 4.97 | 2772.05 | 5.235 | 2244.19 |
| 4.18 | 4643.35 | 4.445 | 2561.15 | 4.71 | 680.15 | 4.975 | 2852.02 | 5.24 | 2348.92 |
| 4.185 | 4570.4 | 4.45 | 2331.94 | 4.715 | 707.67 | 4.98 | 2916.92 | 5.245 | 2461.44 |
| 4.19 | 4503.26 | 4.455 | 2130.66 | 4.72 | 739.08 | 4.985 | 2964.56 | 5.25 | 2580.51 |
| 4.195 | 4443.9 | 4.46 | 1954.64 | 4.725 | 774.5 | 4.99 | 2993.3 | 5.255 | 2704 |
| 4.2 | 4393.18 | 4.465 | 1801.14 | 4.73 | 813.99 | 4.995 | 3002.22 | 5.26 | 2829.75 |
| 4.205 | 4353.41 | 4.47 | 1667.48 | 4.735 | 857.51 | 5 | 2990.87 | 5.265 | 2955.13 |

| | | | | | | | | | |
|---|---|---|---|---|---|---|---|---|---|
| 5.27 | 3077.65 | 5.535 | 1233.9 | 5.8 | 7339.8 | 6.065 | 33681.02 | 6.33 | 72532.4 |
| 5.275 | 3193.69 | 5.54 | 1259.66 | 5.805 | 7690.18 | 6.07 | 35794.98 | 6.335 | 72943.11 |
| 5.28 | 3300.6 | 5.545 | 1291.4 | 5.81 | 8023.15 | 6.075 | 37897.31 | 6.34 | 73116.3 |
| 5.285 | 3395.63 | 5.55 | 1328.73 | 5.815 | 8335.24 | 6.08 | 39950.66 | 6.345 | 73051.11 |
| 5.29 | 3476.36 | 5.555 | 1371.06 | 5.82 | 8624.02 | 6.085 | 41912.18 | 6.35 | 72749.33 |
| 5.295 | 3540.85 | 5.56 | 1417.9 | 5.825 | 8888.19 | 6.09 | 43735.8 | 6.355 | 72215.24 |
| 5.3 | 3587.72 | 5.565 | 1468.66 | 5.83 | 9127.39 | 6.095 | 45374.96 | 6.36 | 71456.65 |
| 5.305 | 3616.79 | 5.57 | 1522.46 | 5.835 | 9341.92 | 6.1 | 46783.68 | 6.365 | 70484.41 |
| 5.31 | 3627.04 | 5.575 | 1578.67 | 5.84 | 9532.42 | 6.105 | 47918.44 | 6.37 | 69311.93 |
| 5.315 | 3619.57 | 5.58 | 1636.48 | 5.845 | 9699.61 | 6.11 | 48744.73 | 6.375 | 67955.66 |
| 5.32 | 3595.61 | 5.585 | 1695.18 | 5.85 | 9844.13 | 6.115 | 49235.96 | 6.38 | 66434.29 |
| 5.325 | 3556.96 | 5.59 | 1754.14 | 5.855 | 9966.35 | 6.12 | 49376.36 | 6.385 | 64768.69 |
| 5.33 | 3505.67 | 5.595 | 1812.87 | 5.86 | 10065.22 | 6.125 | 49162.64 | 6.39 | 62980.89 |
| 5.335 | 3444.26 | 5.6 | 1871.05 | 5.865 | 10139.86 | 6.13 | 48603.97 | 6.395 | 61093.93 |
| 5.34 | 3374.95 | 5.605 | 1928.58 | 5.87 | 10188.46 | 6.135 | 47722.88 | 6.4 | 59130.79 |
| 5.345 | 3300.2 | 5.61 | 1985.42 | 5.875 | 10208.76 | 6.14 | 46553.78 | 6.405 | 57114.31 |
| 5.35 | 3222.21 | 5.615 | 2041.81 | 5.88 | 10198.53 | 6.145 | 45141.86 | 6.41 | 55067.15 |
| 5.355 | 3144.37 | 5.62 | 2098.13 | 5.885 | 10155.47 | 6.15 | 43540.88 | 6.415 | 53009.31 |
| 5.36 | 3065.21 | 5.625 | 2154.85 | 5.89 | 10078.19 | 6.155 | 41810.76 | 6.42 | 50961.21 |
| 5.365 | 2987.18 | 5.63 | 2212.48 | 5.895 | 9965.87 | 6.16 | 40015.31 | 6.425 | 48941.41 |
| 5.37 | 2910.95 | 5.635 | 2271.47 | 5.9 | 9819.51 | 6.165 | 38219.35 | 6.43 | 46967.14 |
| 5.375 | 2836.78 | 5.64 | 2332.2 | 5.905 | 9641.35 | 6.17 | 36486.04 | 6.435 | 45054.8 |
| 5.38 | 2764.68 | 5.645 | 2394.81 | 5.91 | 9435.91 | 6.175 | 34874.96 | 6.44 | 43219.12 |
| 5.385 | 2694.26 | 5.65 | 2459.28 | 5.915 | 9209.3 | 6.18 | 33439.75 | 6.445 | 41473.96 |
| 5.39 | 2625.09 | 5.655 | 2525.26 | 5.92 | 8969.9 | 6.185 | 32227.15 | 6.45 | 39831.77 |
| 5.395 | 2556.6 | 5.66 | 2592.15 | 5.925 | 8727.35 | 6.19 | 31275.18 | 6.455 | 38303.63 |
| 5.4 | 2488.2 | 5.665 | 2659.12 | 5.93 | 8493.99 | 6.195 | 30613.17 | 6.46 | 36898.9 |
| 5.405 | 2419.37 | 5.67 | 2725.2 | 5.935 | 8281.58 | 6.2 | 30261.5 | 6.465 | 35625.07 |
| 5.41 | 2349.65 | 5.675 | 2789.39 | 5.94 | 8103.98 | 6.205 | 30231.36 | 6.47 | 34487.14 |
| 5.415 | 2278.78 | 5.68 | 2850.76 | 5.945 | 7974.92 | 6.21 | 30525.49 | 6.475 | 33487.5 |
| 5.42 | 2206.64 | 5.685 | 2908.69 | 5.95 | 7907.78 | 6.215 | 31138.95 | 6.48 | 32625.73 |
| 5.425 | 2133.27 | 5.69 | 2962.86 | 5.955 | 7915.12 | 6.22 | 32059.56 | 6.485 | 31898.21 |
| 5.43 | 2058.9 | 5.695 | 3013.82 | 5.96 | 8008.63 | 6.225 | 33269.05 | 6.49 | 31298.42 |
| 5.435 | 1983.97 | 5.7 | 3062.31 | 5.965 | 8197.97 | 6.23 | 34744.05 | 6.495 | 30816.84 |
| 5.44 | 1908.89 | 5.705 | 3110.14 | 5.97 | 8491.01 | 6.235 | 36457.15 | 6.5 | 30441.34 |
| 5.445 | 1834.35 | 5.71 | 3159.78 | 5.975 | 8893.41 | 6.24 | 38377.58 | 6.505 | 30158.07 |
| 5.45 | 1760.98 | 5.715 | 3214.4 | 5.98 | 9408.68 | 6.245 | 40473.06 | 6.51 | 29951.35 |
| 5.455 | 1689.5 | 5.72 | 3278.32 | 5.985 | 10038 | 6.25 | 42707.67 | 6.515 | 29804.88 |
| 5.46 | 1620.72 | 5.725 | 3355.51 | 5.99 | 10780.83 | 6.255 | 45046.47 | 6.52 | 29702.29 |
| 5.465 | 1555.41 | 5.73 | 3449.14 | 5.995 | 11635.02 | 6.26 | 47454.52 | 6.525 | 29627.97 |
| 5.47 | 1494.02 | 5.735 | 3564.64 | 6 | 12597.35 | 6.265 | 49897.5 | 6.53 | 29567.34 |
| 5.475 | 1437.23 | 5.74 | 3704.81 | 6.005 | 13664.1 | 6.27 | 52341.42 | 6.535 | 29507.77 |
| 5.48 | 1385.56 | 5.745 | 3873.22 | 6.01 | 14831.51 | 6.275 | 54754.91 | 6.54 | 29438.49 |
| 5.485 | 1339.49 | 5.75 | 4071.92 | 6.015 | 16096.37 | 6.28 | 57108.5 | 6.545 | 29350.63 |
| 5.49 | 1299.35 | 5.755 | 4302.01 | 6.02 | 17456.29 | 6.285 | 59374.69 | 6.55 | 29238.37 |
| 5.495 | 1265.44 | 5.76 | 4563.12 | 6.025 | 18909.8 | 6.29 | 61528.82 | 6.555 | 29097.08 |
| 5.5 | 1237.95 | 5.765 | 4853.62 | 6.03 | 20456.25 | 6.295 | 63548.33 | 6.56 | 28923.97 |
| 5.505 | 1217.1 | 5.77 | 5170.49 | 6.035 | 22095.34 | 6.3 | 65413.81 | 6.565 | 28717.84 |
| 5.51 | 1203.02 | 5.775 | 5509.77 | 6.04 | 23826.46 | 6.305 | 67107.24 | 6.57 | 28478.25 |
| 5.515 | 1195.72 | 5.78 | 5866.01 | 6.045 | 25647.58 | 6.31 | 68613.56 | 6.575 | 28205 |
| 5.52 | 1195.21 | 5.785 | 6233.42 | 6.05 | 27554.69 | 6.315 | 69919.7 | 6.58 | 27898 |
| 5.525 | 1201.47 | 5.79 | 6605.69 | 6.055 | 29538.8 | 6.32 | 71014.17 | 6.585 | 27557.05 |
| 5.53 | 1214.4 | 5.795 | 6976.51 | 6.06 | 31587.19 | 6.325 | 71887.48 | 6.59 | 27181.19 |

| | | | | | | | | | |
|---|---|---|---|---|---|---|---|---|---|
| 6.595 | 26769.07 | 6.86 | 7930.9 | 7.125 | 6763.8 | 7.39 | 2398.84 | 7.655 | 9171.46 |
| 6.6 | 26318.84 | 6.865 | 7605.28 | 7.13 | 6580.94 | 7.395 | 2498.3 | 7.66 | 9609.12 |
| 6.605 | 25828.19 | 6.87 | 7312.42 | 7.135 | 6398.56 | 7.4 | 2604.1 | 7.665 | 10107.93 |
| 6.61 | 25294.9 | 6.875 | 7053.16 | 7.14 | 6221.64 | 7.405 | 2714.93 | 7.67 | 10667.3 |
| 6.615 | 24717.14 | 6.88 | 6828.94 | 7.145 | 6054.55 | 7.41 | 2828.79 | 7.675 | 11284.15 |
| 6.62 | 24094.19 | 6.885 | 6639.21 | 7.15 | 5900.72 | 7.415 | 2944.91 | 7.68 | 11951.36 |
| 6.625 | 23426.3 | 6.89 | 6483.37 | 7.155 | 5762.55 | 7.42 | 3060.8 | 7.685 | 12664.28 |
| 6.63 | 22715.87 | 6.895 | 6359.24 | 7.16 | 5641.19 | 7.425 | 3174.51 | 7.69 | 13411.09 |
| 6.635 | 21966.67 | 6.9 | 6264.88 | 7.165 | 5536.75 | 7.43 | 3283.99 | 7.695 | 14180.23 |
| 6.64 | 21185.17 | 6.905 | 6197.63 | 7.17 | 5448.25 | 7.435 | 3387.23 | 7.7 | 14958.99 |
| 6.645 | 20379.54 | 6.91 | 6154.34 | 7.175 | 5373.65 | 7.44 | 3482.36 | 7.705 | 15734 |
| 6.65 | 19559.9 | 6.915 | 6131.6 | 7.18 | 5310.17 | 7.445 | 3567.91 | 7.71 | 16491.94 |
| 6.655 | 18738.26 | 6.92 | 6125.79 | 7.185 | 5254.47 | 7.45 | 3642.7 | 7.715 | 17220.33 |
| 6.66 | 17927.11 | 6.925 | 6133.21 | 7.19 | 5202.81 | 7.455 | 3706.12 | 7.72 | 17906.93 |
| 6.665 | 17140.68 | 6.93 | 6150.23 | 7.195 | 5151.36 | 7.46 | 3758.08 | 7.725 | 18541.34 |
| 6.67 | 16391.29 | 6.935 | 6173.34 | 7.2 | 5096.83 | 7.465 | 3799.02 | 7.73 | 19114.51 |
| 6.675 | 15691.77 | 6.94 | 6199.35 | 7.205 | 5034.52 | 7.47 | 3830.05 | 7.735 | 19618.93 |
| 6.68 | 15053.26 | 6.945 | 6225.46 | 7.21 | 4962.87 | 7.475 | 3852.96 | 7.74 | 20048.54 |
| 6.685 | 14485.08 | 6.95 | 6249.83 | 7.215 | 4879.24 | 7.48 | 3869.8 | 7.745 | 20398.62 |
| 6.69 | 13994.18 | 6.955 | 6269.87 | 7.22 | 4782.1 | 7.485 | 3883.65 | 7.75 | 20665.78 |
| 6.695 | 13585.12 | 6.96 | 6284.94 | 7.225 | 4670.77 | 7.49 | 3896.79 | 7.755 | 20846.95 |
| 6.7 | 13259.64 | 6.965 | 6294.76 | 7.23 | 4545.35 | 7.495 | 3912.82 | 7.76 | 20939.98 |
| 6.705 | 13016.7 | 6.97 | 6299.21 | 7.235 | 4406.69 | 7.5 | 3934.75 | 7.765 | 20943.49 |
| 6.71 | 12852.98 | 6.975 | 6299.38 | 7.24 | 4256.19 | 7.505 | 3965.79 | 7.77 | 20856.55 |
| 6.715 | 12762.48 | 6.98 | 6296.78 | 7.245 | 4095.84 | 7.51 | 4008.87 | 7.775 | 20678.9 |
| 6.72 | 12737.24 | 6.985 | 6294.29 | 7.25 | 3927.97 | 7.515 | 4066.45 | 7.78 | 20411.35 |
| 6.725 | 12767.63 | 6.99 | 6292.65 | 7.255 | 3755.19 | 7.52 | 4140.57 | 7.785 | 20055.83 |
| 6.73 | 12842.69 | 6.995 | 6295.27 | 7.26 | 3580.21 | 7.525 | 4232.76 | 7.79 | 19615.86 |
| 6.735 | 12950.59 | 7 | 6304.71 | 7.265 | 3405.82 | 7.53 | 4343.63 | 7.795 | 19097.3 |
| 6.74 | 13078.99 | 7.005 | 6323.58 | 7.27 | 3236.09 | 7.535 | 4473.33 | 7.8 | 18507.35 |
| 6.745 | 13215.95 | 7.01 | 6353.84 | 7.275 | 3070.13 | 7.54 | 4620.45 | 7.805 | 17856.41 |
| 6.75 | 13349.38 | 7.015 | 6397.9 | 7.28 | 2911.51 | 7.545 | 4785.18 | 7.81 | 17157.14 |
| 6.755 | 13468.18 | 7.02 | 6456.58 | 7.285 | 2761.91 | 7.55 | 4964.57 | 7.815 | 16424.23 |
| 6.76 | 13562.29 | 7.025 | 6530.29 | 7.29 | 2622.7 | 7.555 | 5155.92 | 7.82 | 15674.29 |
| 6.765 | 13622.88 | 7.03 | 6618.25 | 7.295 | 2494.95 | 7.56 | 5356 | 7.825 | 14925.38 |
| 6.77 | 13642.82 | 7.035 | 6719.74 | 7.3 | 2379.4 | 7.565 | 5561.38 | 7.83 | 14195.31 |
| 6.775 | 13616.57 | 7.04 | 6832.04 | 7.305 | 2276.56 | 7.57 | 5768.32 | 7.835 | 13502.42 |
| 6.78 | 13540.28 | 7.045 | 6952.02 | 7.31 | 2186.93 | 7.575 | 5973.2 | 7.84 | 12863.66 |
| 6.785 | 13412.09 | 7.05 | 7075.66 | 7.315 | 2110.22 | 7.58 | 6172.64 | 7.845 | 12294.37 |
| 6.79 | 13231.61 | 7.055 | 7198.23 | 7.32 | 2046.58 | 7.585 | 6363.83 | 7.85 | 11807.23 |
| 6.795 | 13002.03 | 7.06 | 7314.74 | 7.325 | 1995.92 | 7.59 | 6544.99 | 7.855 | 11412.12 |
| 6.8 | 12724.03 | 7.065 | 7419.99 | 7.33 | 1957.99 | 7.595 | 6714.55 | 7.86 | 11115.76 |
| 6.805 | 12403.02 | 7.07 | 7508.83 | 7.335 | 1932.57 | 7.6 | 6872.94 | 7.865 | 10921.7 |
| 6.81 | 12044.58 | 7.075 | 7576.6 | 7.34 | 1919.41 | 7.605 | 7021.58 | 7.87 | 10830.1 |
| 6.815 | 11654.84 | 7.08 | 7619.26 | 7.345 | 1918.22 | 7.61 | 7163.45 | 7.875 | 10838.68 |
| 6.82 | 11241.56 | 7.085 | 7633.86 | 7.35 | 1928.74 | 7.615 | 7303.26 | 7.88 | 10942.68 |
| 6.825 | 10811.8 | 7.09 | 7618.22 | 7.355 | 1950.83 | 7.62 | 7445.85 | 7.885 | 11135.52 |
| 6.83 | 10373.04 | 7.095 | 7571.73 | 7.36 | 1983.95 | 7.625 | 7598.56 | 7.89 | 11409.34 |
| 6.835 | 9932.67 | 7.1 | 7495.03 | 7.365 | 2028.42 | 7.63 | 7769.08 | 7.895 | 11755.46 |
| 6.84 | 9497.73 | 7.105 | 7390.08 | 7.37 | 2082.94 | 7.635 | 7965.65 | 7.9 | 12164.95 |
| 6.845 | 9074.67 | 7.11 | 7259.95 | 7.375 | 2147.58 | 7.64 | 8196.69 | 7.905 | 12628.61 |
| 6.85 | 8669.3 | 7.115 | 7108.82 | 7.38 | 2221.88 | 7.645 | 8470.14 | 7.91 | 13137.63 |
| 6.855 | 8286.66 | 7.12 | 6941.62 | 7.385 | 2305.21 | 7.65 | 8793.13 | 7.915 | 13683.34 |

| | | | | | | | | | |
|---|---|---|---|---|---|---|---|---|---|
| 7.92 | 14257.42 | 8.185 | 49516.24 | 8.45 | 38958.51 | 8.715 | 55095.73 | 8.98 | 30217.51 |
| 7.925 | 14851.68 | 8.19 | 49879.05 | 8.455 | 37488.14 | 8.72 | 52539.01 | 8.985 | 29943.95 |
| 7.93 | 15458.02 | 8.195 | 50123.2 | 8.46 | 36048.09 | 8.725 | 50081.28 | 8.99 | 29614.23 |
| 7.935 | 16068.4 | 8.2 | 50244.11 | 8.465 | 34649 | 8.73 | 47743.62 | 8.995 | 29232.55 |
| 7.94 | 16674.68 | 8.205 | 50240.43 | 8.47 | 33299.35 | 8.735 | 45537.3 | 9 | 28810.26 |
| 7.945 | 17269.13 | 8.21 | 50114.74 | 8.475 | 32005.74 | 8.74 | 43465.38 | 9.005 | 28352.84 |
| 7.95 | 17844.26 | 8.215 | 49873.59 | 8.48 | 30774.1 | 8.745 | 41524.42 | 9.01 | 27866.69 |
| 7.955 | 18392.48 | 8.22 | 49526.78 | 8.485 | 29610.18 | 8.75 | 39706.34 | 9.015 | 27357.84 |
| 7.96 | 18907.87 | 8.225 | 49086.85 | 8.49 | 28519.19 | 8.755 | 37999.61 | 9.02 | 26832.16 |
| 7.965 | 19385.61 | 8.23 | 48569.13 | 8.495 | 27507.57 | 8.76 | 36391.26 | 9.025 | 26295.44 |
| 7.97 | 19822.75 | 8.235 | 47990.61 | 8.5 | 26582.16 | 8.765 | 34868.99 | 9.03 | 25753.89 |
| 7.975 | 20218.93 | 8.24 | 47369.27 | 8.505 | 25752.07 | 8.77 | 33420.99 | 9.035 | 25214.34 |
| 7.98 | 20575.34 | 8.245 | 46723.81 | 8.51 | 25026.71 | 8.775 | 32037.8 | 9.04 | 24683.97 |
| 7.985 | 20896.75 | 8.25 | 46072.29 | 8.515 | 24417.39 | 8.78 | 30711.94 | 9.045 | 24171.68 |
| 7.99 | 21190.41 | 8.255 | 45432.44 | 8.52 | 23937.01 | 8.785 | 29438.85 | 9.05 | 23684.72 |
| 7.995 | 21465.93 | 8.26 | 44821.45 | 8.525 | 23599.65 | 8.79 | 28216.66 | 9.055 | 23233.81 |
| 8 | 21735.05 | 8.265 | 44254.63 | 8.53 | 23420.65 | 8.795 | 27046.83 | 9.06 | 22828.32 |
| 8.005 | 22011.02 | 8.27 | 43746.7 | 8.535 | 23416.59 | 8.8 | 25930.44 | 9.065 | 22477.47 |
| 8.01 | 22308.81 | 8.275 | 43310.33 | 8.54 | 23604.22 | 8.805 | 24872.66 | 9.07 | 22191.21 |
| 8.015 | 22637.37 | 8.28 | 42957.69 | 8.545 | 24001.43 | 8.81 | 23879.68 | 9.075 | 21976.84 |
| 8.02 | 23014.03 | 8.285 | 42699.23 | 8.55 | 24625.67 | 8.815 | 22958.71 | 9.08 | 21840.39 |
| 8.025 | 23447.33 | 8.29 | 42544.22 | 8.555 | 25493.38 | 8.82 | 22117.71 | 9.085 | 21785.46 |
| 8.03 | 23945.47 | 8.295 | 42500.37 | 8.56 | 26619.85 | 8.825 | 21365.59 | 9.09 | 21812.76 |
| 8.035 | 24512.91 | 8.3 | 42573.78 | 8.565 | 28017.68 | 8.83 | 20709.51 | 9.095 | 21919.92 |
| 8.04 | 25151.32 | 8.305 | 42768.24 | 8.57 | 29696.23 | 8.835 | 20158.13 | 9.1 | 22101.05 |
| 8.045 | 25858.47 | 8.31 | 43084.43 | 8.575 | 31659.73 | 8.84 | 19720.46 | 9.105 | 22346.45 |
| 8.05 | 26629.08 | 8.315 | 43520.35 | 8.58 | 33906.43 | 8.845 | 19400 | 9.11 | 22643.38 |
| 8.055 | 27455.27 | 8.32 | 44070.23 | 8.585 | 36426.79 | 8.85 | 19203 | 9.115 | 22976.63 |
| 8.06 | 28327.32 | 8.325 | 44724.05 | 8.59 | 39203.58 | 8.855 | 19133.39 | 9.12 | 23327.85 |
| 8.065 | 29233.88 | 8.33 | 45467.5 | 8.595 | 42208.7 | 8.86 | 19191.21 | 9.125 | 23679.01 |
| 8.07 | 30163.91 | 8.335 | 46282.46 | 8.6 | 45404.64 | 8.865 | 19375.96 | 9.13 | 24010.3 |
| 8.075 | 31106.45 | 8.34 | 47146.07 | 8.605 | 48742.86 | 8.87 | 19683.96 | 9.135 | 24304.44 |
| 8.08 | 32051.67 | 8.345 | 48032.28 | 8.61 | 52165.4 | 8.875 | 20108.71 | 9.14 | 24544.79 |
| 8.085 | 32992.34 | 8.35 | 48912.23 | 8.615 | 55604.9 | 8.88 | 20641.08 | 9.145 | 24718.55 |
| 8.09 | 33922.69 | 8.355 | 49755.45 | 8.62 | 58987.76 | 8.885 | 21268.71 | 9.15 | 24818.22 |
| 8.095 | 34840.15 | 8.36 | 50530.85 | 8.625 | 62235.27 | 8.89 | 21976.99 | 9.155 | 24840.1 |
| 8.1 | 35743.98 | 8.365 | 51208.63 | 8.63 | 65267.82 | 8.895 | 22748.92 | 9.16 | 24786.55 |
| 8.105 | 36635.79 | 8.37 | 51759.72 | 8.635 | 68007.63 | 8.9 | 23566.82 | 9.165 | 24666.9 |
| 8.11 | 37518.74 | 8.375 | 52159.8 | 8.64 | 70383.11 | 8.905 | 24410.85 | 9.17 | 24495.75 |
| 8.115 | 38396.48 | 8.38 | 52388.55 | 8.645 | 72331.42 | 8.91 | 25257.74 | 9.175 | 24294.22 |
| 8.12 | 39273.13 | 8.385 | 52431.18 | 8.65 | 73803.53 | 8.915 | 26093.81 | 9.18 | 24089.39 |
| 8.125 | 40152.13 | 8.39 | 52278.6 | 8.655 | 74765.58 | 8.92 | 26895.9 | 9.185 | 23913.53 |
| 8.13 | 41035.84 | 8.395 | 51928.11 | 8.66 | 75199.43 | 8.925 | 27648.82 | 9.19 | 23803.01 |
| 8.135 | 41925.58 | 8.4 | 51383.09 | 8.665 | 75106.43 | 8.93 | 28336.25 | 9.195 | 23799.26 |
| 8.14 | 42816.54 | 8.405 | 50653.78 | 8.67 | 74505.53 | 8.935 | 28945.33 | 9.2 | 23945.36 |
| 8.145 | 43707.02 | 8.41 | 49752.33 | 8.675 | 73431.76 | 8.94 | 29466.32 | 9.205 | 24287.94 |
| 8.15 | 44589.02 | 8.415 | 48698.65 | 8.68 | 71933.97 | 8.945 | 29892.31 | 9.21 | 24874.36 |
| 8.155 | 45452.86 | 8.42 | 47513.86 | 8.685 | 70072.39 | 8.95 | 30219.63 | 9.215 | 25752.91 |
| 8.16 | 46286.82 | 8.425 | 46221.18 | 8.69 | 67914.61 | 8.955 | 30447.34 | 9.22 | 26971.89 |
| 8.165 | 47077.31 | 8.43 | 44844.87 | 8.695 | 65531.72 | 8.96 | 30576.99 | 9.225 | 28578.09 |
| 8.17 | 47809.67 | 8.435 | 43408.75 | 8.7 | 62994.57 | 8.965 | 30612.55 | 9.23 | 30617.12 |
| 8.175 | 48469.69 | 8.44 | 41935.42 | 8.705 | 60370.5 | 8.97 | 30559.71 | 9.235 | 33130.87 |
| 8.18 | 49042.84 | 8.445 | 40446.3 | 8.71 | 57720.19 | 8.975 | 30425.54 | 9.24 | 36157.04 |

| | | | | | | | | | |
|---|---|---|---|---|---|---|---|---|---|
| 9.245 | 39727.23 | 9.51 | 50360.18 | 9.775 | 41182.16 | 10.04 | 22916.31 | 10.305 | 32063.74 |
| 9.25 | 43864.82 | 9.515 | 52231.04 | 9.78 | 39466.18 | 10.045 | 21960.45 | 10.31 | 33031.88 |
| 9.255 | 48583.75 | 9.52 | 54337.3 | 9.785 | 38072.85 | 10.05 | 21088.86 | 10.315 | 33952.09 |
| 9.26 | 53885.57 | 9.525 | 56714.4 | 9.79 | 36992.25 | 10.055 | 20308.7 | 10.32 | 34800.19 |
| 9.265 | 59757.5 | 9.53 | 59407.12 | 9.795 | 36213.54 | 10.06 | 19624.22 | 10.325 | 35554.79 |
| 9.27 | 66170.1 | 9.535 | 62464.18 | 9.8 | 35725.4 | 10.065 | 19037.81 | 10.33 | 36198.18 |
| 9.275 | 73075.2 | 9.54 | 65934.98 | 9.805 | 35515.88 | 10.07 | 18549.25 | 10.335 | 36716.77 |
| 9.28 | 80404.95 | 9.545 | 69865.47 | 9.81 | 35572.14 | 10.075 | 18155.41 | 10.34 | 37102.02 |
| 9.285 | 88070.53 | 9.55 | 74293.99 | 9.815 | 35880.76 | 10.08 | 17854.4 | 10.345 | 37350.09 |
| 9.29 | 95961.55 | 9.555 | 79244.74 | 9.82 | 36424.73 | 10.085 | 17640.56 | 10.35 | 37461.77 |
| 9.295 | 103948.51 | 9.56 | 84723.35 | 9.825 | 37187.96 | 10.09 | 17508.56 | 10.355 | 37444.6 |
| 9.3 | 111884.03 | 9.565 | 90713.67 | 9.83 | 38148.32 | 10.095 | 17452.33 | 10.36 | 37304.32 |
| 9.305 | 119606.94 | 9.57 | 97173.67 | 9.835 | 39281.94 | 10.1 | 17467.29 | 10.365 | 37053.7 |
| 9.31 | 126946.69 | 9.575 | 104032.69 | 9.84 | 40562.92 | 10.105 | 17548.75 | 10.37 | 36707.3 |
| 9.315 | 133730.68 | 9.58 | 111192.66 | 9.845 | 41960.69 | 10.11 | 17693.09 | 10.375 | 36280.3 |
| 9.32 | 139788.42 | 9.585 | 118528.69 | 9.85 | 43442.38 | 10.115 | 17897.27 | 10.38 | 35788.04 |
| 9.325 | 144960.28 | 9.59 | 125893.9 | 9.855 | 44971.61 | 10.12 | 18158.69 | 10.385 | 35244.92 |
| 9.33 | 149106.76 | 9.595 | 133123.19 | 9.86 | 46511.26 | 10.125 | 18474.41 | 10.39 | 34663.96 |
| 9.335 | 152112.51 | 9.6 | 140042.19 | 9.865 | 48021.79 | 10.13 | 18841.78 | 10.395 | 34055.3 |
| 9.34 | 153889.67 | 9.605 | 146474.01 | 9.87 | 49464.4 | 10.135 | 19257.25 | 10.4 | 33426.43 |
| 9.345 | 154389.49 | 9.61 | 152248.87 | 9.875 | 50800.36 | 10.14 | 19715.75 | 10.405 | 32782.65 |
| 9.35 | 153600.08 | 9.615 | 157212.61 | 9.88 | 51994.4 | 10.145 | 20210.63 | 10.41 | 32125.44 |
| 9.355 | 151549.42 | 9.62 | 161234.12 | 9.885 | 53014.23 | 10.15 | 20733.69 | 10.415 | 31454.07 |
| 9.36 | 148302.11 | 9.625 | 164212.44 | 9.89 | 53831.68 | 10.155 | 21274.88 | 10.42 | 30765.51 |
| 9.365 | 143958.66 | 9.63 | 166081.33 | 9.895 | 54424.99 | 10.16 | 21822.31 | 10.425 | 30056.78 |
| 9.37 | 138649.88 | 9.635 | 166810.47 | 9.9 | 54779.02 | 10.165 | 22362.97 | 10.43 | 29326.04 |
| 9.375 | 132530.04 | 9.64 | 166408.84 | 9.905 | 54885.11 | 10.17 | 22883.14 | 10.435 | 28565.75 |
| 9.38 | 125769.84 | 9.645 | 164915.63 | 9.91 | 54743.24 | 10.175 | 23369 | 10.44 | 27776.33 |
| 9.385 | 118554.31 | 9.65 | 162403.15 | 9.915 | 54360.12 | 10.18 | 23807.39 | 10.445 | 26959.02 |
| 9.39 | 111061.8 | 9.655 | 158970.87 | 9.92 | 53748.49 | 10.185 | 24187.34 | 10.45 | 26118.03 |
| 9.395 | 103471.95 | 9.66 | 154732.35 | 9.925 | 52931.4 | 10.19 | 24499.35 | 10.455 | 25261.17 |
| 9.4 | 95951.03 | 9.665 | 149813.1 | 9.93 | 51932.03 | 10.195 | 24738.24 | 10.46 | 24399.34 |
| 9.405 | 88648.63 | 9.67 | 144344.18 | 9.935 | 50778.53 | 10.2 | 24901.58 | 10.465 | 23547.04 |
| 9.41 | 81694.89 | 9.675 | 138452.77 | 9.94 | 49501.27 | 10.205 | 24991.64 | 10.47 | 22721 |
| 9.415 | 75196.53 | 9.68 | 132260.91 | 9.945 | 48130.85 | 10.21 | 25014.93 | 10.475 | 21939.85 |
| 9.42 | 69236.3 | 9.685 | 125879.24 | 9.95 | 46695.75 | 10.215 | 24981.84 | 10.48 | 21222.66 |
| 9.425 | 63873.22 | 9.69 | 119406.09 | 9.955 | 45222.64 | 10.22 | 24906.74 | 10.485 | 20588.11 |
| 9.43 | 59144.02 | 9.695 | 112925.98 | 9.96 | 43733.66 | 10.225 | 24807.34 | 10.49 | 20055.53 |
| 9.435 | 55064.22 | 9.7 | 106510.33 | 9.965 | 42247.02 | 10.23 | 24703.38 | 10.495 | 19635.29 |
| 9.44 | 51630.13 | 9.705 | 100218.44 | 9.97 | 40775.34 | 10.235 | 24615.92 | 10.5 | 19339.61 |
| 9.445 | 48823.7 | 9.71 | 94098.72 | 9.975 | 39326.86 | 10.24 | 24566.69 | 10.505 | 19175.84 |
| 9.45 | 46612.28 | 9.715 | 88190.45 | 9.98 | 37905.53 | 10.245 | 24576.03 | 10.51 | 19144.01 |
| 9.455 | 44956.77 | 9.72 | 82526.86 | 9.985 | 36511.93 | 10.25 | 24662.81 | 10.515 | 19241.55 |
| 9.46 | 43810.03 | 9.725 | 77133.87 | 9.99 | 35144.62 | 10.255 | 24842.95 | 10.52 | 19460.78 |
| 9.465 | 43121.7 | 9.73 | 72033.47 | 9.995 | 33800.61 | 10.26 | 25128.66 | 10.525 | 19789.99 |
| 9.47 | 42839.96 | 9.735 | 67243.73 | 10 | 32477.51 | 10.265 | 25528.59 | 10.53 | 20213.84 |
| 9.475 | 42915.31 | 9.74 | 62779.04 | 10.005 | 31173.5 | 10.27 | 26042.74 | 10.535 | 20715.12 |
| 9.48 | 43300.45 | 9.745 | 58652.38 | 10.01 | 29890.16 | 10.275 | 26670.81 | 10.54 | 21275.34 |
| 9.485 | 43953.98 | 9.75 | 54867.95 | 10.015 | 28629.21 | 10.28 | 27404.36 | 10.545 | 21875.83 |
| 9.49 | 44841.4 | 9.755 | 51434.11 | 10.02 | 27396.21 | 10.285 | 28230.52 | 10.55 | 22499.54 |
| 9.495 | 45936.87 | 9.76 | 48351.01 | 10.025 | 26198.64 | 10.29 | 29132.02 | 10.555 | 23131.3 |
| 9.5 | 47223.65 | 9.765 | 45617.61 | 10.03 | 25046.51 | 10.295 | 30087.66 | 10.56 | 23761.66 |
| 9.505 | 48696.25 | 9.77 | 43230.02 | 10.035 | 23947.87 | 10.3 | 31073.49 | 10.565 | 24379.33 |

| | | | | | | | | | |
|---|---|---|---|---|---|---|---|---|---|
| 10.57 | 24983.23 | 10.835 | 63403.92 | 11.1 | 215215.28 | 11.365 | 88174.68 | 11.63 | 72947.59 |
| 10.575 | 25574.92 | 10.84 | 59906.61 | 11.105 | 220982.43 | 11.37 | 89778.28 | 11.635 | 73817.9 |
| 10.58 | 26161.35 | 10.845 | 56566.87 | 11.11 | 226741.93 | 11.375 | 91676.77 | 11.64 | 74647.79 |
| 10.585 | 26752.48 | 10.85 | 53468.03 | 11.115 | 232482 | 11.38 | 93838.16 | 11.645 | 75424.63 |
| 10.59 | 27364.78 | 10.855 | 50681.85 | 11.12 | 238162.01 | 11.385 | 96216.8 | 11.65 | 76139.44 |
| 10.595 | 28009.48 | 10.86 | 48270.71 | 11.125 | 243709.69 | 11.39 | 98750.32 | 11.655 | 76794.45 |
| 10.6 | 28705.29 | 10.865 | 46283.52 | 11.13 | 249022.42 | 11.395 | 101365.23 | 11.66 | 77390.23 |
| 10.605 | 29469.27 | 10.87 | 44750.86 | 11.135 | 253966.85 | 11.4 | 103979.57 | 11.665 | 77936.66 |
| 10.61 | 30315.89 | 10.875 | 43693.67 | 11.14 | 258388.51 | 11.405 | 106507.5 | 11.67 | 78443.88 |
| 10.615 | 31257.47 | 10.88 | 43115.26 | 11.145 | 262116 | 11.41 | 108858.69 | 11.675 | 78929.09 |
| 10.62 | 32302.91 | 10.885 | 43005.78 | 11.15 | 264975.64 | 11.415 | 110950.65 | 11.68 | 79412.4 |
| 10.625 | 33457.33 | 10.89 | 43342 | 11.155 | 266794.53 | 11.42 | 112706.82 | 11.685 | 79915.17 |
| 10.63 | 34720.27 | 10.895 | 44090.22 | 11.16 | 267423.03 | 11.425 | 114064.76 | 11.69 | 80458.92 |
| 10.635 | 36088.35 | 10.9 | 45205.71 | 11.165 | 266738.98 | 11.43 | 114975.45 | 11.695 | 81063.61 |
| 10.64 | 37556.16 | 10.905 | 46638.69 | 11.17 | 264655.18 | 11.435 | 115408.41 | 11.7 | 81746.11 |
| 10.645 | 39113.95 | 10.91 | 48327.92 | 11.175 | 261136.59 | 11.44 | 115350.74 | 11.705 | 82518.6 |
| 10.65 | 40752.15 | 10.915 | 50215.51 | 11.18 | 256188.83 | 11.445 | 114808.1 | 11.71 | 83386.56 |
| 10.655 | 42460.24 | 10.92 | 52239.95 | 11.185 | 249876.8 | 11.45 | 113802.55 | 11.715 | 84348.15 |
| 10.66 | 44231.65 | 10.925 | 54345.14 | 11.19 | 242310.39 | 11.455 | 112372.27 | 11.72 | 85392.47 |
| 10.665 | 46059.37 | 10.93 | 56479.5 | 11.195 | 233643.32 | 11.46 | 110564.92 | 11.725 | 86500.59 |
| 10.67 | 47939.9 | 10.935 | 58600.38 | 11.2 | 224064.98 | 11.465 | 108437.3 | 11.73 | 87644.33 |
| 10.675 | 49876.49 | 10.94 | 60677.55 | 11.205 | 213789.74 | 11.47 | 106050.84 | 11.735 | 88789.05 |
| 10.68 | 51866.31 | 10.945 | 62697.82 | 11.21 | 203052.55 | 11.475 | 103468.13 | 11.74 | 89892.25 |
| 10.685 | 53913.43 | 10.95 | 64655.07 | 11.215 | 192086.99 | 11.48 | 100750.25 | 11.745 | 90908.83 |
| 10.69 | 56024.22 | 10.955 | 66567.27 | 11.22 | 181121.05 | 11.485 | 97954.58 | 11.75 | 91792.11 |
| 10.695 | 58202.4 | 10.96 | 68465.38 | 11.225 | 170367.61 | 11.49 | 95128.47 | 11.755 | 92495.59 |
| 10.7 | 60451.97 | 10.965 | 70395.12 | 11.23 | 160014 | 11.495 | 92324.64 | 11.76 | 92978.42 |
| 10.705 | 62768.11 | 10.97 | 72412.92 | 11.235 | 150219.23 | 11.5 | 89577.09 | 11.765 | 93206.16 |
| 10.71 | 65146.49 | 10.975 | 74584.57 | 11.24 | 141108.87 | 11.505 | 86916.93 | 11.77 | 93153.84 |
| 10.715 | 67575.55 | 10.98 | 76981.13 | 11.245 | 132770.1 | 11.51 | 84369.18 | 11.775 | 92807.56 |
| 10.72 | 70037 | 10.985 | 79673.29 | 11.25 | 125258.27 | 11.515 | 81953.6 | 11.78 | 92166.31 |
| 10.725 | 72507.74 | 10.99 | 82725.44 | 11.255 | 118594.63 | 11.52 | 79685.58 | 11.785 | 91242.01 |
| 10.73 | 74959.11 | 10.995 | 86193.08 | 11.26 | 112771.21 | 11.525 | 77577.07 | 11.79 | 90057.7 |
| 10.735 | 77355.56 | 11 | 90118.58 | 11.265 | 107754.07 | 11.53 | 75636.71 | 11.795 | 88646.78 |
| 10.74 | 79659.14 | 11.005 | 94529.23 | 11.27 | 103489.97 | 11.535 | 73872.53 | 11.8 | 87051.14 |
| 10.745 | 81827.99 | 11.01 | 99430.79 | 11.275 | 99910.37 | 11.54 | 72290.4 | 11.805 | 85318.44 |
| 10.75 | 83817.93 | 11.015 | 104815.71 | 11.28 | 96935.86 | 11.545 | 70895.33 | 11.81 | 83498.17 |
| 10.755 | 85584.78 | 11.02 | 110648.78 | 11.285 | 94483.75 | 11.55 | 69690.51 | 11.815 | 81639.08 |
| 10.76 | 87081.52 | 11.025 | 116886.67 | 11.29 | 92470.91 | 11.555 | 68679.08 | 11.82 | 79786.98 |
| 10.765 | 88265.36 | 11.03 | 123462.79 | 11.295 | 90818.13 | 11.56 | 67863.82 | 11.825 | 77980.3 |
| 10.77 | 89094.09 | 11.035 | 130302.44 | 11.3 | 89454.75 | 11.565 | 67243.84 | 11.83 | 76250.69 |
| 10.775 | 89530.83 | 11.04 | 137327.54 | 11.305 | 88321.47 | 11.57 | 66818.18 | 11.835 | 74619.6 |
| 10.78 | 89544.17 | 11.045 | 144446.09 | 11.31 | 87370.41 | 11.575 | 66583.73 | 11.84 | 73099.38 |
| 10.785 | 89110.3 | 11.05 | 151580.44 | 11.315 | 86569.23 | 11.58 | 66532.35 | 11.845 | 71693.55 |
| 10.79 | 88215.61 | 11.055 | 158655.24 | 11.32 | 85900.89 | 11.585 | 66660.18 | 11.85 | 70398.08 |
| 10.795 | 86856.69 | 11.06 | 165613.27 | 11.325 | 85361.19 | 11.59 | 66953.85 | 11.855 | 69200.72 |
| 10.8 | 85044.19 | 11.065 | 172406.44 | 11.33 | 84958.13 | 11.595 | 67396.37 | 11.86 | 68086.32 |
| 10.805 | 82801.93 | 11.07 | 179008.33 | 11.335 | 84713.55 | 11.6 | 67970.03 | 11.865 | 67037.66 |
| 10.81 | 80169.4 | 11.075 | 185410.75 | 11.34 | 84653.39 | 11.605 | 68654.46 | 11.87 | 66035.04 |
| 10.815 | 77198.95 | 11.08 | 191623.88 | 11.345 | 84809.96 | 11.61 | 69429.87 | 11.875 | 65061.73 |
| 10.82 | 73956.83 | 11.085 | 197673.04 | 11.35 | 85214.89 | 11.615 | 70270.48 | 11.88 | 64103.43 |
| 10.825 | 70519.6 | 11.09 | 203594.47 | 11.355 | 85897.53 | 11.62 | 71154.63 | 11.885 | 63152.6 |
| 10.83 | 66972.11 | 11.095 | 209429.01 | 11.36 | 86881.06 | 11.625 | 72052.78 | 11.89 | 62194.77 |

| | | | | | | | | | |
|---|---|---|---|---|---|---|---|---|---|
| 11.895 | 61238.14 | 12.16 | 54650.72 | 12.425 | 38274.75 | 12.69 | 136311.5 | 12.955 | 138222.5 |
| 11.9 | 60283.26 | 12.165 | 53116.67 | 12.43 | 38472.17 | 12.695 | 136859.28 | 12.96 | 136054.82 |
| 11.905 | 59341.65 | 12.17 | 51676.13 | 12.435 | 38765.58 | 12.7 | 138243.27 | 12.965 | 134218.67 |
| 11.91 | 58422.91 | 12.175 | 50358.79 | 12.44 | 39170.46 | 12.705 | 140429.78 | 12.97 | 132688.31 |
| 11.915 | 57545.3 | 12.18 | 49190.92 | 12.445 | 39704.72 | 12.71 | 143369.56 | 12.975 | 131431.12 |
| 11.92 | 56727.7 | 12.185 | 48192.18 | 12.45 | 40388.9 | 12.715 | 146988.86 | 12.98 | 130418.74 |
| 11.925 | 55989.25 | 12.19 | 47377.43 | 12.455 | 41245.62 | 12.72 | 151197.44 | 12.985 | 129618.62 |
| 11.93 | 55354.57 | 12.195 | 46755.99 | 12.46 | 42299.81 | 12.725 | 155897.29 | 12.99 | 128974.85 |
| 11.935 | 54841.79 | 12.2 | 46332.18 | 12.465 | 43577.82 | 12.73 | 160968.97 | 12.995 | 128457.66 |
| 11.94 | 54469.59 | 12.205 | 46101.53 | 12.47 | 45107.14 | 12.735 | 166295.46 | 13 | 128029.46 |
| 11.945 | 54252.77 | 12.21 | 46056.84 | 12.475 | 46917.57 | 12.74 | 171756.31 | 13.005 | 127654.55 |
| 11.95 | 54203.32 | 12.215 | 46184.39 | 12.48 | 49037.12 | 12.745 | 177234.33 | 13.01 | 127300.06 |
| 11.955 | 54328.26 | 12.22 | 46466.94 | 12.485 | 51494.89 | 12.75 | 182621.66 | 13.015 | 126938.13 |
| 11.96 | 54629.33 | 12.225 | 46881.56 | 12.49 | 54318.06 | 12.755 | 187827.8 | 13.02 | 126545.93 |
| 11.965 | 55103.95 | 12.23 | 47403.25 | 12.495 | 57535.13 | 12.76 | 192775.94 | 13.025 | 126110.68 |
| 11.97 | 55741.8 | 12.235 | 48007.02 | 12.5 | 61168.99 | 12.765 | 197412.68 | 13.03 | 125632.67 |
| 11.975 | 56527.63 | 12.24 | 48657.17 | 12.505 | 65240.3 | 12.77 | 201703.33 | 13.035 | 125123.79 |
| 11.98 | 57443.22 | 12.245 | 49329.12 | 12.51 | 69763.89 | 12.775 | 205636.45 | 13.04 | 124612.23 |
| 11.985 | 58463.91 | 12.25 | 49988.62 | 12.515 | 74748.69 | 12.78 | 209222.16 | 13.045 | 124151.7 |
| 11.99 | 59563.36 | 12.255 | 50608.43 | 12.52 | 80195.58 | 12.785 | 212470.44 | 13.05 | 123811.32 |
| 11.995 | 60713.08 | 12.26 | 51161.12 | 12.525 | 86089.49 | 12.79 | 215411.43 | 13.055 | 123683.94 |
| 12 | 61879.93 | 12.265 | 51622.89 | 12.53 | 92418.24 | 12.795 | 218072.82 | 13.06 | 123884.84 |
| 12.005 | 63036.72 | 12.27 | 51973.84 | 12.535 | 99142.38 | 12.8 | 220477.47 | 13.065 | 124553.98 |
| 12.01 | 64156.55 | 12.275 | 52198.56 | 12.54 | 106209.23 | 12.805 | 222639.25 | 13.07 | 125832.76 |
| 12.015 | 65214.39 | 12.28 | 52286.55 | 12.545 | 113552.65 | 12.81 | 224557.44 | 13.075 | 127883.5 |
| 12.02 | 66190.98 | 12.285 | 52233.09 | 12.55 | 121087.03 | 12.815 | 226216 | 13.08 | 130866.48 |
| 12.025 | 67072.09 | 12.29 | 52037.65 | 12.555 | 128712.02 | 12.82 | 227582.92 | 13.085 | 134932.06 |
| 12.03 | 67848.14 | 12.295 | 51706.6 | 12.56 | 136311.94 | 12.825 | 228612.45 | 13.09 | 140210.59 |
| 12.035 | 68515.4 | 12.3 | 51246.36 | 12.565 | 143757.51 | 12.83 | 229250.71 | 13.095 | 146798.55 |
| 12.04 | 69074.65 | 12.305 | 50671.61 | 12.57 | 150910.14 | 12.835 | 229440.36 | 13.1 | 154746.43 |
| 12.045 | 69531.07 | 12.31 | 49997.77 | 12.575 | 157631.33 | 12.84 | 229120.33 | 13.105 | 164052.83 |
| 12.05 | 69893.05 | 12.315 | 49243.1 | 12.58 | 163774.52 | 12.845 | 228245.67 | 13.11 | 174645.63 |
| 12.055 | 70168.32 | 12.32 | 48426.72 | 12.585 | 169207.55 | 12.85 | 226775.79 | 13.115 | 186388.33 |
| 12.06 | 70366.68 | 12.325 | 47567.87 | 12.59 | 173811.51 | 12.855 | 224693.18 | 13.12 | 199068.89 |
| 12.065 | 70495.62 | 12.33 | 46685.29 | 12.595 | 177483.31 | 12.86 | 222002.76 | 13.125 | 212416.62 |
| 12.07 | 70559.1 | 12.335 | 45798.82 | 12.6 | 180147.45 | 12.865 | 218722.03 | 13.13 | 226080.51 |
| 12.075 | 70560.86 | 12.34 | 44921.64 | 12.605 | 181761.2 | 12.87 | 214900.2 | 13.135 | 239682.82 |
| 12.08 | 70496.56 | 12.345 | 44069.78 | 12.61 | 182313.15 | 12.875 | 210586.21 | 13.14 | 252807.3 |
| 12.085 | 70359.03 | 12.35 | 43255.62 | 12.615 | 181828.68 | 12.88 | 205860.22 | 13.145 | 265034.01 |
| 12.09 | 70141.5 | 12.355 | 42489.06 | 12.62 | 180367.77 | 12.885 | 200805.51 | 13.15 | 275958.28 |
| 12.095 | 69824.53 | 12.36 | 41778.01 | 12.625 | 178024.52 | 12.89 | 195514.94 | 13.155 | 285220.51 |
| 12.1 | 69397.27 | 12.365 | 41129.66 | 12.63 | 174921.1 | 12.895 | 190074.65 | 13.16 | 292519.2 |
| 12.105 | 68844.52 | 12.37 | 40543.51 | 12.635 | 171204.46 | 12.9 | 184577.56 | 13.165 | 297632.61 |
| 12.11 | 68154.51 | 12.375 | 40022.87 | 12.64 | 167038.31 | 12.905 | 179107.85 | 13.17 | 300447.66 |
| 12.115 | 67318.94 | 12.38 | 39573.92 | 12.645 | 162596.04 | 12.91 | 173743.19 | 13.175 | 300938.6 |
| 12.12 | 66334.22 | 12.385 | 39184.19 | 12.65 | 158061.05 | 12.915 | 168551.71 | 13.18 | 299181 |
| 12.125 | 65201.63 | 12.39 | 38857.53 | 12.655 | 153604.61 | 12.92 | 163592.95 | 13.185 | 295356.16 |
| 12.13 | 63931.05 | 12.395 | 38591.72 | 12.66 | 149393.22 | 12.925 | 158915.33 | 13.19 | 289726.68 |
| 12.135 | 62537.71 | 12.4 | 38384.98 | 12.665 | 145581.61 | 12.93 | 154556.79 | 13.195 | 282621.71 |
| 12.14 | 61042.94 | 12.405 | 38237.34 | 12.67 | 142296.59 | 12.935 | 150546.43 | 13.2 | 274424.63 |
| 12.145 | 59477.42 | 12.41 | 38148.45 | 12.675 | 139651.66 | 12.94 | 146902.61 | 13.205 | 265521.61 |
| 12.15 | 57865.66 | 12.415 | 38121.45 | 12.68 | 137734.43 | 12.945 | 143634.85 | 13.21 | 256322.21 |
| 12.155 | 56244.78 | 12.42 | 38161.24 | 12.685 | 136608.01 | 12.95 | 140744.31 | 13.215 | 247215.1 |

| | | | | | | | | | |
|---|---|---|---|---|---|---|---|---|---|
| 13.22 | 238546.89 | 13.485 | 201032.48 | 13.75 | 326138.89 | 14.015 | 695492.87 | 14.28 | 421953.43 |
| 13.225 | 230631.49 | 13.49 | 202129 | 13.755 | 329798.12 | 14.02 | 719088.11 | 14.285 | 427198.82 |
| 13.23 | 223726.61 | 13.495 | 204873.14 | 13.76 | 334536.82 | 14.025 | 740272.65 | 14.29 | 440817.63 |
| 13.235 | 218033.99 | 13.5 | 209277.68 | 13.765 | 340310.38 | 14.03 | 758392.09 | 14.295 | 463745.75 |
| 13.24 | 213701.26 | 13.505 | 215364.16 | 13.77 | 347014.35 | 14.035 | 772889.64 | 14.3 | 496856.62 |
| 13.245 | 210826.45 | 13.51 | 223173.5 | 13.775 | 354497.57 | 14.04 | 783352.91 | 14.305 | 540928.8 |
| 13.25 | 209457.92 | 13.515 | 232733.15 | 13.78 | 362553.57 | 14.045 | 789534.61 | 14.31 | 596632.95 |
| 13.255 | 209605.36 | 13.52 | 244090.01 | 13.785 | 370942.98 | 14.05 | 791371.51 | 14.315 | 664448.86 |
| 13.26 | 211245.49 | 13.525 | 257267.21 | 13.79 | 379396.29 | 14.055 | 788992.35 | 14.32 | 744641.73 |
| 13.265 | 214326.54 | 13.53 | 272266.22 | 13.795 | 387635.66 | 14.06 | 782690.14 | 14.325 | 837201.65 |
| 13.27 | 218781.38 | 13.535 | 289050.35 | 13.8 | 395399.19 | 14.065 | 772936 | 14.33 | 941779.97 |
| 13.275 | 224516.36 | 13.54 | 307524.75 | 13.805 | 402444.92 | 14.07 | 760338.81 | 14.335 | 1.05766E6 |
| 13.28 | 231426.05 | 13.545 | 327526.82 | 13.81 | 408569.79 | 14.075 | 745600.81 | 14.34 | 1.18369E6 |
| 13.285 | 239403.6 | 13.55 | 348826.35 | 13.815 | 413634.05 | 14.08 | 729501.46 | 14.345 | 1.31824E6 |
| 13.29 | 248332.88 | 13.555 | 371095.94 | 13.82 | 417548.16 | 14.085 | 712826.78 | 14.35 | 1.45925E6 |
| 13.295 | 258095.15 | 13.56 | 393934.56 | 13.825 | 420296.26 | 14.09 | 696356.76 | 14.355 | 1.60417E6 |
| 13.3 | 268565.42 | 13.565 | 416860.6 | 13.83 | 421919.3 | 14.095 | 680816.09 | 14.36 | 1.75007E6 |
| 13.305 | 279610.06 | 13.57 | 439332.53 | 13.835 | 422517.37 | 14.1 | 666844.94 | 14.365 | 1.89367E6 |
| 13.31 | 291108.72 | 13.575 | 460773.15 | 13.84 | 422236.18 | 14.105 | 654978.09 | 14.37 | 2.03145E6 |
| 13.315 | 302915.73 | 13.58 | 480591.21 | 13.845 | 421250.38 | 14.11 | 645626.48 | 14.375 | 2.15981E6 |
| 13.32 | 314887.18 | 13.585 | 498204.98 | 13.85 | 419751.02 | 14.115 | 639068.7 | 14.38 | 2.27515E6 |
| 13.325 | 326861.52 | 13.59 | 513095.04 | 13.855 | 417934.06 | 14.12 | 635446.73 | 14.385 | 2.37416E6 |
| 13.33 | 338665.98 | 13.595 | 524819.36 | 13.86 | 415980.82 | 14.125 | 634775.73 | 14.39 | 2.4538E6 |
| 13.335 | 350110.19 | 13.6 | 533049.27 | 13.865 | 414052.45 | 14.13 | 636925.12 | 14.395 | 2.51159E6 |
| 13.34 | 360984.56 | 13.605 | 537596.85 | 13.87 | 412282.71 | 14.135 | 641676.33 | 14.4 | 2.5457E6 |
| 13.345 | 371065.7 | 13.61 | 538385.94 | 13.875 | 410787.69 | 14.14 | 648699.75 | 14.405 | 2.55503E6 |
| 13.35 | 380118.83 | 13.615 | 535547.44 | 13.88 | 409612.42 | 14.145 | 657571.61 | 14.41 | 2.53931E6 |
| 13.355 | 387902.5 | 13.62 | 529323.51 | 13.885 | 408809.15 | 14.15 | 667807.03 | 14.415 | 2.49908E6 |
| 13.36 | 394174.39 | 13.625 | 520088.4 | 13.89 | 408387.82 | 14.155 | 678863.33 | 14.42 | 2.43566E6 |
| 13.365 | 398734.95 | 13.63 | 508323.11 | 13.895 | 408346.05 | 14.16 | 690152.9 | 14.425 | 2.35111E6 |
| 13.37 | 401382 | 13.635 | 494574.53 | 13.9 | 408672.21 | 14.165 | 701075.87 | 14.43 | 2.24809E6 |
| 13.375 | 401969.13 | 13.64 | 479441.97 | 13.905 | 409353.51 | 14.17 | 711034.26 | 14.435 | 2.12976E6 |
| 13.38 | 400402.12 | 13.645 | 463518.62 | 13.91 | 410384.59 | 14.175 | 719449.17 | 14.44 | 1.99954E6 |
| 13.385 | 396649.62 | 13.65 | 447359.66 | 13.915 | 411782.91 | 14.18 | 725780.83 | 14.445 | 1.86107E6 |
| 13.39 | 390749.35 | 13.655 | 431469.38 | 13.92 | 413585.79 | 14.185 | 729558.93 | 14.45 | 1.71794E6 |
| 13.395 | 382809.85 | 13.66 | 416263.7 | 13.925 | 415864.61 | 14.19 | 730378.65 | 14.455 | 1.57358E6 |
| 13.4 | 373006.65 | 13.665 | 402067.98 | 13.93 | 418735.72 | 14.195 | 727913.58 | 14.46 | 1.43116E6 |
| 13.405 | 361573.69 | 13.67 | 389102.85 | 13.935 | 422333.49 | 14.2 | 721982.92 | 14.465 | 1.29344E6 |
| 13.41 | 348800.72 | 13.675 | 377491.58 | 13.94 | 426840.8 | 14.205 | 712488.6 | 14.47 | 1.16276E6 |
| 13.415 | 335021.32 | 13.68 | 367263.88 | 13.945 | 432474.12 | 14.21 | 699476.32 | 14.475 | 1.04096E6 |
| 13.42 | 320589.3 | 13.685 | 358388.58 | 13.95 | 439469.44 | 14.215 | 683092.73 | 14.48 | 929360.29 |
| 13.425 | 305848.31 | 13.69 | 350763.04 | 13.955 | 448068.49 | 14.22 | 663644.09 | 14.485 | 828831.3 |
| 13.43 | 291163.47 | 13.695 | 344269.22 | 13.96 | 458510.71 | 14.225 | 641515.22 | 14.49 | 739778.76 |
| 13.435 | 276860.26 | 13.7 | 338777.11 | 13.965 | 470998.84 | 14.23 | 617219.54 | 14.495 | 662221.93 |
| 13.44 | 263245.63 | 13.705 | 334152.09 | 13.97 | 485690.97 | 14.235 | 591355.55 | 14.5 | 595805.14 |
| 13.445 | 250579.41 | 13.71 | 330293.84 | 13.975 | 502672.14 | 14.24 | 564625.91 | 14.505 | 539947.3 |
| 13.45 | 239082.33 | 13.715 | 327132.85 | 13.98 | 521937.14 | 14.245 | 537797.52 | 14.51 | 493826.24 |
| 13.455 | 228930.83 | 13.72 | 324639.88 | 13.985 | 543357.79 | 14.25 | 511690.48 | 14.515 | 456454.59 |
| 13.46 | 220253.23 | 13.725 | 322824.49 | 13.99 | 566699.42 | 14.255 | 487204.99 | 14.52 | 426759.06 |
| 13.465 | 213137.54 | 13.73 | 321731.33 | 13.995 | 591596.01 | 14.26 | 465244.56 | 14.525 | 403612.13 |
| 13.47 | 207637.41 | 13.735 | 321435.95 | 14 | 617552.24 | 14.265 | 446762.07 | 14.53 | 385872.75 |
| 13.475 | 203788.67 | 13.74 | 322012.75 | 14.005 | 643983.47 | 14.27 | 432722.47 | 14.535 | 372445.12 |
| 13.48 | 201585.46 | 13.745 | 323557.89 | 14.01 | 670208.44 | 14.275 | 424125.25 | 14.54 | 362271.72 |

| | | | | | | | | | |
|---|---|---|---|---|---|---|---|---|---|
| 14.545 | 354392.67 | 14.81 | 3.33688E6 | 15.075 | 97196.29 | 15.34 | 146108.33 | 15.605 | 70560.78 |
| 14.55 | 347955.04 | 14.815 | 3.50097E6 | 15.08 | 95553.33 | 15.345 | 139618.03 | 15.61 | 71278.29 |
| 14.555 | 342222.69 | 14.82 | 3.63471E6 | 15.085 | 94145.24 | 15.35 | 133247.3 | 15.615 | 71952.3 |
| 14.56 | 336602.84 | 14.825 | 3.73389E6 | 15.09 | 92958.41 | 15.355 | 127076 | 15.62 | 72527.46 |
| 14.565 | 330631.39 | 14.83 | 3.79542E6 | 15.095 | 91975.82 | 15.36 | 121173.28 | 15.625 | 72954.57 |
| 14.57 | 324013.56 | 14.835 | 3.81744E6 | 15.1 | 91187.08 | 15.365 | 115601.74 | 15.63 | 73191.64 |
| 14.575 | 316577.33 | 14.84 | 3.79944E6 | 15.105 | 90586.5 | 15.37 | 110410.81 | 15.635 | 73203.92 |
| 14.58 | 308295.79 | 14.845 | 3.74227E6 | 15.11 | 90168.6 | 15.375 | 105641.76 | 15.64 | 72970.42 |
| 14.585 | 299237.97 | 14.85 | 3.64809E6 | 15.115 | 89932.15 | 15.38 | 101327.95 | 15.645 | 72475.23 |
| 14.59 | 289606.25 | 14.855 | 3.52023E6 | 15.12 | 89865.22 | 15.385 | 97495.93 | 15.65 | 71714.78 |
| 14.595 | 279668.32 | 14.86 | 3.36304E6 | 15.125 | 89991.92 | 15.39 | 94164.77 | 15.655 | 70695.11 |
| 14.6 | 269753.54 | 14.865 | 3.18159E6 | 15.13 | 90302.46 | 15.395 | 91347.44 | 15.66 | 69431.71 |
| 14.605 | 260213.11 | 14.87 | 2.98144E6 | 15.135 | 90803.59 | 15.4 | 89051.13 | 15.665 | 67948.01 |
| 14.61 | 251426.6 | 14.875 | 2.76835E6 | 15.14 | 91501.7 | 15.405 | 87276.8 | 15.67 | 66274.45 |
| 14.615 | 243730.36 | 14.88 | 2.548E6 | 15.145 | 92411.44 | 15.41 | 86017.31 | 15.675 | 64447.43 |
| 14.62 | 237443.24 | 14.885 | 2.32577E6 | 15.15 | 93553.64 | 15.415 | 85259.55 | 15.68 | 62505.04 |
| 14.625 | 232786.71 | 14.89 | 2.10651E6 | 15.155 | 94943.97 | 15.42 | 84980.31 | 15.685 | 60489.22 |
| 14.63 | 229960.63 | 14.895 | 1.8944E6 | 15.16 | 96605.58 | 15.425 | 85149.01 | 15.69 | 58440.4 |
| 14.635 | 229039.37 | 14.9 | 1.69281E6 | 15.165 | 98564.35 | 15.43 | 85723.87 | 15.695 | 56396.54 |
| 14.64 | 230043.41 | 14.905 | 1.50434E6 | 15.17 | 100847.41 | 15.435 | 86652.83 | 15.7 | 54396.19 |
| 14.645 | 232866.95 | 14.91 | 1.33073E6 | 15.175 | 103484.9 | 15.44 | 87875.62 | 15.705 | 52468.71 |
| 14.65 | 237374 | 14.915 | 1.17298E6 | 15.18 | 106502.97 | 15.445 | 89320.77 | 15.71 | 50640.1 |
| 14.655 | 243358.43 | 14.92 | 1.03141E6 | 15.185 | 109923.4 | 15.45 | 90909.7 | 15.715 | 48929.74 |
| 14.66 | 250580.61 | 14.925 | 905757.42 | 15.19 | 113762.08 | 15.455 | 92557.93 | 15.72 | 47350.99 |
| 14.665 | 258784.68 | 14.93 | 795310.96 | 15.195 | 118025.75 | 15.46 | 94178.68 | 15.725 | 45909.98 |
| 14.67 | 267761.35 | 14.935 | 699032.37 | 15.2 | 122708.99 | 15.465 | 95684.37 | 15.73 | 44607.43 |
| 14.675 | 277365 | 14.94 | 615666.84 | 15.205 | 127790.49 | 15.47 | 96991.09 | 15.735 | 43436.01 |
| 14.68 | 287549.47 | 14.945 | 543851.32 | 15.21 | 133236.21 | 15.475 | 98022.19 | 15.74 | 42390.66 |
| 14.685 | 298410.59 | 14.95 | 482191.82 | 15.215 | 138993.77 | 15.48 | 98711.26 | 15.745 | 41453.31 |
| 14.69 | 310234.68 | 14.955 | 429344.23 | 15.22 | 144991.94 | 15.485 | 99010 | 15.75 | 40607.62 |
| 14.695 | 323515.82 | 14.96 | 384052.55 | 15.225 | 151143.07 | 15.49 | 98881.33 | 15.755 | 39833.37 |
| 14.7 | 338984.7 | 14.965 | 345183.58 | 15.23 | 157348.09 | 15.495 | 98310.52 | 15.76 | 39109.71 |
| 14.705 | 357622.18 | 14.97 | 311741.11 | 15.235 | 163493.66 | 15.5 | 97300.32 | 15.765 | 38415.35 |
| 14.71 | 380660.9 | 14.975 | 282872.61 | 15.24 | 169458.71 | 15.505 | 95871.85 | 15.77 | 37730.64 |
| 14.715 | 409565.63 | 14.98 | 257855.02 | 15.245 | 175118.64 | 15.51 | 94067.82 | 15.775 | 37036.26 |
| 14.72 | 446012.76 | 14.985 | 236096.78 | 15.25 | 180349.89 | 15.515 | 91947.53 | 15.78 | 36315.76 |
| 14.725 | 491838.46 | 14.99 | 217106.41 | 15.255 | 185034.55 | 15.52 | 89576.77 | 15.785 | 35559.05 |
| 14.73 | 548968.38 | 14.995 | 200476.5 | 15.26 | 189062.53 | 15.525 | 87038.5 | 15.79 | 34756.79 |
| 14.735 | 619335.28 | 15 | 185905.16 | 15.265 | 192339.12 | 15.53 | 84415.32 | 15.795 | 33904.86 |
| 14.74 | 704778.14 | 15.005 | 173101.63 | 15.27 | 194784.59 | 15.535 | 81792.51 | 15.8 | 33002.93 |
| 14.745 | 806930.96 | 15.01 | 161861.91 | 15.275 | 196344.1 | 15.54 | 79252.27 | 15.805 | 32059.23 |
| 14.75 | 927067.05 | 15.015 | 151987.56 | 15.28 | 196977.79 | 15.545 | 76870.03 | 15.81 | 31083.09 |
| 14.755 | 1.06601E6 | 15.02 | 143327.01 | 15.285 | 196671.52 | 15.55 | 74711.54 | 15.815 | 30089.31 |
| 14.76 | 1.22397E6 | 15.025 | 135755.11 | 15.29 | 195430.65 | 15.555 | 72829.42 | 15.82 | 29097.17 |
| 14.765 | 1.40047E6 | 15.03 | 129133.45 | 15.295 | 193289.2 | 15.56 | 71261.51 | 15.825 | 28129.18 |
| 14.77 | 1.59421E6 | 15.035 | 123345.38 | 15.3 | 190294 | 15.565 | 70032.22 | 15.83 | 27210.28 |
| 14.775 | 1.80302E6 | 15.04 | 118288.71 | 15.305 | 186512.93 | 15.57 | 69148.98 | 15.835 | 26367.33 |
| 14.78 | 2.02385E6 | 15.045 | 113894.21 | 15.31 | 182029.2 | 15.575 | 68604.43 | 15.84 | 25628.11 |
| 14.785 | 2.25279E6 | 15.05 | 110061.78 | 15.315 | 176937.21 | 15.58 | 68378.46 | 15.845 | 25021.73 |
| 14.79 | 2.48516E6 | 15.055 | 106727.32 | 15.32 | 171341.11 | 15.585 | 68436.47 | 15.85 | 24577.97 |
| 14.795 | 2.71563E6 | 15.06 | 103825.13 | 15.325 | 165350.83 | 15.59 | 68738.76 | 15.855 | 24325.6 |
| 14.8 | 2.9384E6 | 15.065 | 101299.14 | 15.33 | 159076.18 | 15.595 | 69230.47 | 15.86 | 24293.71 |
| 14.805 | 3.14747E6 | 15.07 | 99102.4 | 15.335 | 152627.13 | 15.6 | 69858.1 | 15.865 | 24512.48 |

| | | | | | | | | | |
|---|---|---|---|---|---|---|---|---|---|
| 15.87 | 25010.7 | 16.135 | 64286.6 | 16.4 | 109129.15 | 16.665 | 16211.47 | 16.93 | 69478.66 |
| 15.875 | 25819.07 | 16.14 | 69134.25 | 16.405 | 106536.99 | 16.67 | 16189.86 | 16.935 | 64323.05 |
| 15.88 | 26971.05 | 16.145 | 74818.27 | 16.41 | 103811.93 | 16.675 | 16287.43 | 16.94 | 59945.93 |
| 15.885 | 28498.32 | 16.15 | 81335.78 | 16.415 | 100984.91 | 16.68 | 16533.18 | 16.945 | 56267.61 |
| 15.89 | 30434.01 | 16.155 | 88674.68 | 16.42 | 98090.95 | 16.685 | 16964.63 | 16.95 | 53204.99 |
| 15.895 | 32811.19 | 16.16 | 96805.02 | 16.425 | 95159.48 | 16.69 | 17622.33 | 16.955 | 50676.14 |
| 15.9 | 35662.03 | 16.165 | 105679.54 | 16.43 | 92226.29 | 16.695 | 18557.98 | 16.96 | 48603.16 |
| 15.905 | 39016 | 16.17 | 115225.89 | 16.435 | 89318.16 | 16.7 | 19826.13 | 16.965 | 46915.26 |
| 15.91 | 42897 | 16.175 | 125345.76 | 16.44 | 86457.91 | 16.705 | 21489.54 | 16.97 | 45551.89 |
| 15.915 | 47320.74 | 16.18 | 135914.5 | 16.445 | 83663.49 | 16.71 | 23618.29 | 16.975 | 44453.66 |
| 15.92 | 52293.95 | 16.185 | 146777.35 | 16.45 | 80945.1 | 16.715 | 26288.4 | 16.98 | 43583.24 |
| 15.925 | 57806.93 | 16.19 | 157753.9 | 16.455 | 78306.86 | 16.72 | 29579.8 | 16.985 | 42902.44 |
| 15.93 | 63832.21 | 16.195 | 168640.73 | 16.46 | 75746.88 | 16.725 | 33574.17 | 16.99 | 42384.49 |
| 15.935 | 70324.67 | 16.2 | 179217.73 | 16.465 | 73256.82 | 16.73 | 38352.03 | 16.995 | 42007.28 |
| 15.94 | 77217.14 | 16.205 | 189253.82 | 16.47 | 70823.65 | 16.735 | 43986.79 | 17 | 41755.21 |
| 15.945 | 84417.02 | 16.21 | 198517.04 | 16.475 | 68430.45 | 16.74 | 50543.31 | 17.005 | 41615.73 |
| 15.95 | 91810.99 | 16.215 | 206785.76 | 16.48 | 66060.82 | 16.745 | 58068.78 | 17.01 | 41580.08 |
| 15.955 | 99264.93 | 16.22 | 213856.58 | 16.485 | 63696.39 | 16.75 | 66589.14 | 17.015 | 41638.81 |
| 15.96 | 106626.9 | 16.225 | 219556.58 | 16.49 | 61321.48 | 16.755 | 76102.06 | 17.02 | 41781.82 |
| 15.965 | 113732.11 | 16.23 | 223752.18 | 16.495 | 58923.16 | 16.76 | 86578.46 | 17.025 | 42004.07 |
| 15.97 | 120408.78 | 16.235 | 226357.15 | 16.5 | 56492.76 | 16.765 | 97947.74 | 17.03 | 42292.17 |
| 15.975 | 126484.85 | 16.24 | 227337.62 | 16.505 | 54027.33 | 16.77 | 110101.93 | 17.035 | 42633.44 |
| 15.98 | 131795.6 | 16.245 | 226714.88 | 16.51 | 51529.83 | 16.775 | 122893.92 | 17.04 | 43012.48 |
| 15.985 | 136193.51 | 16.25 | 224564.81 | 16.515 | 49008.89 | 16.78 | 136135.64 | 17.045 | 43412.51 |
| 15.99 | 139549.08 | 16.255 | 221013.65 | 16.52 | 46478.52 | 16.785 | 149603.84 | 17.05 | 43814.66 |
| 15.995 | 141770.63 | 16.26 | 216231.78 | 16.525 | 43958.01 | 16.79 | 163042.29 | 17.055 | 44196.37 |
| 16 | 142792.53 | 16.265 | 210425.21 | 16.53 | 41469.53 | 16.795 | 176170.08 | 17.06 | 44536.27 |
| 16.005 | 142587.96 | 16.27 | 203822.85 | 16.535 | 39038.79 | 16.8 | 188692.1 | 17.065 | 44810.65 |
| 16.01 | 141175.73 | 16.275 | 196667.15 | 16.54 | 36690.4 | 16.805 | 200307.13 | 17.07 | 44997.99 |
| 16.015 | 138606.33 | 16.28 | 189200.38 | 16.545 | 34450.62 | 16.81 | 210721.95 | 17.075 | 45076.75 |
| 16.02 | 134969.53 | 16.285 | 181653.77 | 16.55 | 32341.84 | 16.815 | 219663.19 | 17.08 | 45028.59 |
| 16.025 | 130385.81 | 16.29 | 174237.51 | 16.555 | 30382.89 | 16.82 | 226889.22 | 17.085 | 44840.06 |
| 16.03 | 125001.67 | 16.295 | 167132.82 | 16.56 | 28588.73 | 16.825 | 232202.05 | 17.09 | 44498.6 |
| 16.035 | 118983.63 | 16.3 | 160486.22 | 16.565 | 26972.05 | 16.83 | 235457.13 | 17.095 | 43996.72 |
| 16.04 | 112508.48 | 16.305 | 154405.47 | 16.57 | 25533.68 | 16.835 | 236570.35 | 17.1 | 43333.75 |
| 16.045 | 105757.23 | 16.31 | 148960.19 | 16.575 | 24271.66 | 16.84 | 235522.88 | 17.105 | 42510.29 |
| 16.05 | 98907.19 | 16.315 | 144181.81 | 16.58 | 23178.72 | 16.845 | 232362.53 | 17.11 | 41534.74 |
| 16.055 | 92126.09 | 16.32 | 140067.44 | 16.585 | 22243.45 | 16.85 | 227201.87 | 17.115 | 40416.9 |
| 16.06 | 85567.89 | 16.325 | 136584.84 | 16.59 | 21449.43 | 16.855 | 220212.93 | 17.12 | 39170.61 |
| 16.065 | 79367.96 | 16.33 | 133677.1 | 16.595 | 20777.8 | 16.86 | 211618.83 | 17.125 | 37814.82 |
| 16.07 | 73640.48 | 16.335 | 131268.87 | 16.6 | 20208.33 | 16.865 | 201682.85 | 17.13 | 36367.29 |
| 16.075 | 68480.04 | 16.34 | 129273.29 | 16.605 | 19720.78 | 16.87 | 190696.3 | 17.135 | 34848.86 |
| 16.08 | 63958.21 | 16.345 | 127597.43 | 16.61 | 19295.42 | 16.875 | 178964.64 | 17.14 | 33280.05 |
| 16.085 | 60130.12 | 16.35 | 126146.11 | 16.615 | 18914.74 | 16.88 | 166795.25 | 17.145 | 31678.94 |
| 16.09 | 57033.43 | 16.355 | 124829.44 | 16.62 | 18564.35 | 16.885 | 154482.03 | 17.15 | 30068.79 |
| 16.095 | 54692.56 | 16.36 | 123563.74 | 16.625 | 18231.86 | 16.89 | 142298.3 | 17.155 | 28465.59 |
| 16.1 | 53122.41 | 16.365 | 122275.62 | 16.63 | 17911.72 | 16.895 | 130478.03 | 17.16 | 26885.31 |
| 16.105 | 52332.48 | 16.37 | 120903.3 | 16.635 | 17599.16 | 16.9 | 119226.76 | 17.165 | 25342.99 |
| 16.11 | 52327.84 | 16.375 | 119399.11 | 16.64 | 17295.54 | 16.905 | 108700.16 | 17.17 | 23851.39 |
| 16.115 | 53112.73 | 16.38 | 117726.08 | 16.645 | 17006.38 | 16.91 | 99011.24 | 17.175 | 22421.21 |
| 16.12 | 54692.9 | 16.385 | 115867.09 | 16.65 | 16739.9 | 16.915 | 90230.84 | 17.18 | 21061.34 |
| 16.125 | 57075.71 | 16.39 | 113811.14 | 16.655 | 16507.19 | 16.92 | 82389.02 | 17.185 | 19778.5 |
| 16.13 | 60269.91 | 16.395 | 111560.64 | 16.66 | 16324.67 | 16.925 | 75482.42 | 17.19 | 18579.23 |

| | | | | | | | | | |
|---|---|---|---|---|---|---|---|---|---|
| 17.195 | 17466.51 | 17.46 | 5630.6 | 17.725 | 6917.98 | 17.99 | 4005.58 | 18.255 | 24998.75 |
| 17.2 | 16442.73 | 17.465 | 5451.65 | 17.73 | 6911.3 | 17.995 | 4041 | 18.26 | 24169.37 |
| 17.205 | 15508.25 | 17.47 | 5287.15 | 17.735 | 6880.82 | 18 | 4083.87 | 18.265 | 23457.28 |
| 17.21 | 14662.38 | 17.475 | 5137.91 | 17.74 | 6825.35 | 18.005 | 4136.56 | 18.27 | 22858.75 |
| 17.215 | 13901.8 | 17.48 | 5004.23 | 17.745 | 6744.4 | 18.01 | 4199.66 | 18.275 | 22364.15 |
| 17.22 | 13222.32 | 17.485 | 4886.22 | 17.75 | 6638.02 | 18.015 | 4275.42 | 18.28 | 21959.1 |
| 17.225 | 12618.09 | 17.49 | 4783.82 | 17.755 | 6507.33 | 18.02 | 4366.34 | 18.285 | 21626.2 |
| 17.23 | 12081.51 | 17.495 | 4696.81 | 17.76 | 6353.86 | 18.025 | 4474.76 | 18.29 | 21346.53 |
| 17.235 | 11605.14 | 17.5 | 4625.12 | 17.765 | 6180.1 | 18.03 | 4604 | 18.295 | 21101.19 |
| 17.24 | 11179.68 | 17.505 | 4568.62 | 17.77 | 5990.09 | 18.035 | 4757.44 | 18.3 | 20872.73 |
| 17.245 | 10795.43 | 17.51 | 4526.93 | 17.775 | 5785.22 | 18.04 | 4939.94 | 18.305 | 20646.3 |
| 17.25 | 10443.62 | 17.515 | 4500.03 | 17.78 | 5572.01 | 18.045 | 5156.29 | 18.31 | 20410.57 |
| 17.255 | 10114.98 | 17.52 | 4487.24 | 17.785 | 5354.42 | 18.05 | 5412.3 | 18.315 | 20158.08 |
| 17.26 | 9802.57 | 17.525 | 4487.59 | 17.79 | 5137.01 | 18.055 | 5714.62 | 18.32 | 19885.48 |
| 17.265 | 9499.31 | 17.53 | 4499.95 | 17.795 | 4924.36 | 18.06 | 6070.32 | 18.325 | 19593.23 |
| 17.27 | 9200.54 | 17.535 | 4522.86 | 17.8 | 4720.97 | 18.065 | 6487.78 | 18.33 | 19285.24 |
| 17.275 | 8903.01 | 17.54 | 4554.42 | 17.805 | 4530.86 | 18.07 | 6975.59 | 18.335 | 18968.18 |
| 17.28 | 8606.3 | 17.545 | 4592.58 | 17.81 | 4357.36 | 18.075 | 7543.07 | 18.34 | 18650.65 |
| 17.285 | 8311.02 | 17.55 | 4635.15 | 17.815 | 4203.18 | 18.08 | 8199.46 | 18.345 | 18342.43 |
| 17.29 | 8019.95 | 17.555 | 4679.78 | 17.82 | 4070.25 | 18.085 | 8953.87 | 18.35 | 18053.06 |
| 17.295 | 7737.37 | 17.56 | 4724.4 | 17.825 | 3959.56 | 18.09 | 9814.37 | 18.355 | 17792.17 |
| 17.3 | 7468.68 | 17.565 | 4767.22 | 17.83 | 3871.06 | 18.095 | 10789.14 | 18.36 | 17567.36 |
| 17.305 | 7219.99 | 17.57 | 4806.99 | 17.835 | 3804.95 | 18.1 | 11882.75 | 18.365 | 17384.76 |
| 17.31 | 6997.88 | 17.575 | 4842.87 | 17.84 | 3759.33 | 18.105 | 13098.81 | 18.37 | 17248.26 |
| 17.315 | 6808.17 | 17.58 | 4874.65 | 17.845 | 3732.38 | 18.11 | 14436.68 | 18.375 | 17159.45 |
| 17.32 | 6656.33 | 17.585 | 4902.78 | 17.85 | 3721.64 | 18.115 | 15892.28 | 18.38 | 17117.36 |
| 17.325 | 6546.25 | 17.59 | 4928.48 | 17.855 | 3724.24 | 18.12 | 17457.15 | 18.385 | 17118.91 |
| 17.33 | 6480.4 | 17.595 | 4952.97 | 17.86 | 3737.27 | 18.125 | 19118 | 18.39 | 17158.59 |
| 17.335 | 6459.71 | 17.6 | 4978.1 | 17.865 | 3757.69 | 18.13 | 20856.42 | 18.395 | 17230.1 |
| 17.34 | 6482.73 | 17.605 | 5005.77 | 17.87 | 3782.68 | 18.135 | 22649.05 | 18.4 | 17324.8 |
| 17.345 | 6545.4 | 17.61 | 5037.94 | 17.875 | 3809.57 | 18.14 | 24467.73 | 18.405 | 17433.53 |
| 17.35 | 6643.57 | 17.615 | 5076.23 | 17.88 | 3836.23 | 18.145 | 26279.97 | 18.41 | 17546.64 |
| 17.355 | 6769.29 | 17.62 | 5122.16 | 17.885 | 3860.79 | 18.15 | 28050.21 | 18.415 | 17654.06 |
| 17.36 | 6914.34 | 17.625 | 5176.92 | 17.89 | 3882.02 | 18.155 | 29740.66 | 18.42 | 17746.14 |
| 17.365 | 7069.1 | 17.63 | 5240.84 | 17.895 | 3899.05 | 18.16 | 31312.92 | 18.425 | 17813.87 |
| 17.37 | 7223.77 | 17.635 | 5313.79 | 17.9 | 3911.55 | 18.165 | 32729.59 | 18.43 | 17848.98 |
| 17.375 | 7368.72 | 17.64 | 5396.02 | 17.905 | 3919.52 | 18.17 | 33956.01 | 18.435 | 17844.64 |
| 17.38 | 7494.75 | 17.645 | 5486.64 | 17.91 | 3923.37 | 18.175 | 34962.03 | 18.44 | 17795.18 |
| 17.385 | 7593.81 | 17.65 | 5584.56 | 17.915 | 3923.74 | 18.18 | 35723.62 | 18.445 | 17696.45 |
| 17.39 | 7660.07 | 17.655 | 5688.52 | 17.92 | 3921.33 | 18.185 | 36224.13 | 18.45 | 17545.94 |
| 17.395 | 7688.74 | 17.66 | 5797.44 | 17.925 | 3917.01 | 18.19 | 36455.71 | 18.455 | 17342.74 |
| 17.4 | 7677.61 | 17.665 | 5909.72 | 17.93 | 3911.94 | 18.195 | 36419.49 | 18.46 | 17087.45 |
| 17.405 | 7626.53 | 17.67 | 6023.28 | 17.935 | 3906.89 | 18.2 | 36126.05 | 18.465 | 16782.11 |
| 17.41 | 7536.86 | 17.675 | 6138.25 | 17.94 | 3902.51 | 18.205 | 35594.69 | 18.47 | 16429.99 |
| 17.415 | 7412.38 | 17.68 | 6252.04 | 17.945 | 3899.47 | 18.21 | 34852.91 | 18.475 | 16035.53 |
| 17.42 | 7257.47 | 17.685 | 6363.32 | 17.95 | 3898.39 | 18.215 | 33934.8 | 18.48 | 15603.86 |
| 17.425 | 7078.12 | 17.69 | 6470.23 | 17.955 | 3899.59 | 18.22 | 32879.35 | 18.485 | 15140.74 |
| 17.43 | 6880.48 | 17.695 | 6570.91 | 17.96 | 3903.5 | 18.225 | 31728.46 | 18.49 | 14652.19 |
| 17.435 | 6670.9 | 17.7 | 6663.19 | 17.965 | 3910.46 | 18.23 | 30524.76 | 18.495 | 14144.34 |
| 17.44 | 6455.16 | 17.705 | 6744.83 | 17.97 | 3920.84 | 18.235 | 29309.23 | 18.5 | 13623.08 |
| 17.445 | 6239.28 | 17.71 | 6813.59 | 17.975 | 3935.01 | 18.24 | 28119.71 | 18.505 | 13093.99 |
| 17.45 | 6025.95 | 17.715 | 6866.99 | 17.98 | 3953.35 | 18.245 | 26988.68 | 18.51 | 12562.21 |
| 17.455 | 5822.86 | 17.72 | 6902.51 | 17.985 | 3976.66 | 18.25 | 25942.15 | 18.515 | 12032.2 |

| | | | | | | | | | |
|---|---|---|---|---|---|---|---|---|---|
| 18.52 | 11507.98 | 18.785 | 1849.12 | 19.05 | 1086.51 | 19.315 | 364.93 | 19.58 | 151 |
| 18.525 | 10992.38 | 18.79 | 1872.79 | 19.055 | 1132.7 | 19.32 | 369.24 | 19.585 | 144.44 |
| 18.53 | 10488.28 | 18.795 | 1900.65 | 19.06 | 1179.42 | 19.325 | 374.65 | 19.59 | 138.57 |
| 18.535 | 9997.75 | 18.8 | 1930.89 | 19.065 | 1225.9 | 19.33 | 381.23 | 19.595 | 133.28 |
| 18.54 | 9522.33 | 18.805 | 1961.08 | 19.07 | 1271.43 | 19.335 | 389.14 | 19.6 | 128.51 |
| 18.545 | 9063.03 | 18.81 | 1988.6 | 19.075 | 1315.26 | 19.34 | 398.49 | 19.605 | 124.21 |
| 18.55 | 8620.93 | 18.815 | 2010.77 | 19.08 | 1356.68 | 19.345 | 409.41 | 19.61 | 120.3 |
| 18.555 | 8196.4 | 18.82 | 2025.72 | 19.085 | 1395.01 | 19.35 | 422.04 | 19.615 | 116.74 |
| 18.56 | 7789.88 | 18.825 | 2031.16 | 19.09 | 1429.59 | 19.355 | 436.48 | 19.62 | 113.45 |
| 18.565 | 7401.49 | 18.83 | 2025.22 | 19.095 | 1459.89 | 19.36 | 452.77 | 19.625 | 110.4 |
| 18.57 | 7031.63 | 18.835 | 2006.79 | 19.1 | 1485.4 | 19.365 | 470.88 | 19.63 | 107.66 |
| 18.575 | 6680.15 | 18.84 | 1975.12 | 19.105 | 1505.66 | 19.37 | 490.73 | 19.635 | 105.12 |
| 18.58 | 6346.86 | 18.845 | 1930.17 | 19.11 | 1520.3 | 19.375 | 512.13 | 19.64 | 102.77 |
| 18.585 | 6032.04 | 18.85 | 1872.5 | 19.115 | 1528.97 | 19.38 | 534.78 | 19.645 | 100.57 |
| 18.59 | 5735.25 | 18.855 | 1803.13 | 19.12 | 1531.42 | 19.385 | 558.28 | 19.65 | 98.52 |
| 18.595 | 5456.32 | 18.86 | 1723.96 | 19.125 | 1527.43 | 19.39 | 582.23 | 19.655 | 96.58 |
| 18.6 | 5194.76 | 18.865 | 1636.83 | 19.13 | 1516.84 | 19.395 | 606.04 | 19.66 | 94.77 |
| 18.605 | 4950.42 | 18.87 | 1543.94 | 19.135 | 1499.54 | 19.4 | 629.09 | 19.665 | 93.06 |
| 18.61 | 4722.7 | 18.875 | 1447.64 | 19.14 | 1475.7 | 19.405 | 650.82 | 19.67 | 91.44 |
| 18.615 | 4511.04 | 18.88 | 1350.3 | 19.145 | 1445.35 | 19.41 | 670.53 | 19.675 | 89.9 |
| 18.62 | 4314.48 | 18.885 | 1254.15 | 19.15 | 1408.81 | 19.415 | 687.65 | 19.68 | 88.45 |
| 18.625 | 4133.12 | 18.89 | 1161.15 | 19.155 | 1366.46 | 19.42 | 701.39 | 19.685 | 87.06 |
| 18.63 | 3965.59 | 18.895 | 1073.11 | 19.16 | 1318.86 | 19.425 | 711.64 | 19.69 | 85.71 |
| 18.635 | 3811.01 | 18.9 | 991.35 | 19.165 | 1266.7 | 19.43 | 717.8 | 19.695 | 84.46 |
| 18.64 | 3668.59 | 18.905 | 916.93 | 19.17 | 1210.77 | 19.435 | 719.6 | 19.7 | 83.25 |
| 18.645 | 3537.23 | 18.91 | 850.51 | 19.175 | 1151.95 | 19.44 | 716.88 | 19.705 | 82.09 |
| 18.65 | 3415.77 | 18.915 | 792.57 | 19.18 | 1091.23 | 19.445 | 709.63 | 19.71 | 80.97 |
| 18.655 | 3303.23 | 18.92 | 743.11 | 19.185 | 1029.55 | 19.45 | 697.97 | 19.715 | 79.9 |
| 18.66 | 3198.45 | 18.925 | 701.99 | 19.19 | 967.78 | 19.455 | 682.15 | 19.72 | 78.87 |
| 18.665 | 3100.24 | 18.93 | 668.79 | 19.195 | 907 | 19.46 | 662.52 | 19.725 | 77.87 |
| 18.67 | 3007.76 | 18.935 | 643.14 | 19.2 | 847.94 | 19.465 | 639.57 | 19.73 | 76.9 |
| 18.675 | 2919.86 | 18.94 | 624.33 | 19.205 | 791.3 | 19.47 | 613.82 | 19.735 | 75.97 |
| 18.68 | 2835.48 | 18.945 | 611.91 | 19.21 | 737.67 | 19.475 | 585.84 | 19.74 | 75.07 |
| 18.685 | 2754.36 | 18.95 | 605.13 | 19.215 | 687.46 | 19.48 | 556.22 | 19.745 | 74.2 |
| 18.69 | 2674.84 | 18.955 | 603.34 | 19.22 | 641 | 19.485 | 525.58 | 19.75 | 73.35 |
| 18.695 | 2597.91 | 18.96 | 605.94 | 19.225 | 598.51 | 19.49 | 494.47 | 19.755 | 72.54 |
| 18.7 | 2522.52 | 18.965 | 612.33 | 19.23 | 560.05 | 19.495 | 463.42 | 19.76 | 71.7 |
| 18.705 | 2448.44 | 18.97 | 622.04 | 19.235 | 525.58 | 19.5 | 432.89 | 19.765 | 70.95 |
| 18.71 | 2375.79 | 18.975 | 634.57 | 19.24 | 495.02 | 19.505 | 403.33 | 19.77 | 70.21 |
| 18.715 | 2304.75 | 18.98 | 649.64 | 19.245 | 468.21 | 19.51 | 375.04 | 19.775 | 69.49 |
| 18.72 | 2235.72 | 18.985 | 666.93 | 19.25 | 445.02 | 19.515 | 348.27 | 19.78 | 68.74 |
| 18.725 | 2169.25 | 18.99 | 686.31 | 19.255 | 425.2 | 19.52 | 323.16 | 19.785 | 68.06 |
| 18.73 | 2105.94 | 18.995 | 707.59 | 19.26 | 408.5 | 19.525 | 299.88 | 19.79 | 67.37 |
| 18.735 | 2046.83 | 19 | 730.89 | 19.265 | 394.69 | 19.53 | 278.45 | 19.795 | 66.73 |
| 18.74 | 1992.68 | 19.005 | 756.21 | 19.27 | 383.49 | 19.535 | 258.87 | 19.8 | 66.11 |
| 18.745 | 1944.05 | 19.01 | 783.63 | 19.275 | 374.69 | 19.54 | 241.09 | 19.805 | 65.5 |
| 18.75 | 1902.66 | 19.015 | 813.29 | 19.28 | 367.99 | 19.545 | 225.03 | 19.81 | 64.89 |
| 18.755 | 1869.02 | 19.02 | 845.24 | 19.285 | 363.25 | 19.55 | 210.59 | 19.815 | 64.3 |
| 18.76 | 1843.75 | 19.025 | 879.73 | 19.29 | 360.22 | 19.555 | 197.65 | 19.82 | 63.73 |
| 18.765 | 1827.35 | 19.03 | 916.71 | 19.295 | 358.7 | 19.56 | 186.09 | 19.825 | 63.16 |
| 18.77 | 1819.95 | 19.035 | 956.09 | 19.3 | 358.51 | 19.565 | 175.76 | 19.83 | 62.56 |
| 18.775 | 1821.6 | 19.04 | 997.74 | 19.305 | 359.55 | 19.57 | 166.55 | 19.835 | 62.02 |
| 18.78 | 1831.64 | 19.045 | 1041.37 | 19.31 | 361.7 | 19.575 | 158.33 | 19.84 | 61.5 |

| | |
|---|---|
| 19.845 | 60.99 |
| 19.85 | 60.48 |
| 19.855 | 59.92 |
| 19.86 | 59.45 |
| 19.865 | 58.86 |
| 19.87 | 58.43 |
| 19.875 | 57.99 |
| 19.88 | 57.57 |
| 19.885 | 57.16 |
| 19.89 | 56.71 |
| 19.895 | 56.33 |
| 19.9 | 55.96 |
| 19.905 | 55.6 |
| 19.91 | 55.25 |
| 19.915 | 54.91 |
| 19.92 | 54.57 |
| 19.925 | 54.19 |
| 19.93 | 53.89 |
| 19.935 | 53.62 |
| 19.94 | 53.35 |
| 19.945 | 53.12 |
| 19.95 | 52.84 |
| 19.955 | 52.63 |
| 19.96 | 52.46 |
| 19.965 | 52.31 |
| 19.97 | 52.14 |
| 19.975 | 52.03 |
| 19.98 | 51.95 |
| 19.985 | 51.9 |
| 19.99 | 51.86 |
| 19.995 | 51.88 |
| 20 | 51.95 |

**$Ce^{2+}$ : Energy vs DR cross section**

| Energy (eV) | Barn |
|---|---|
| 0 | 8.67735E8 |
| 0.005 | 8.67679E8 |
| 0.01 | 8.56296E8 |
| 0.015 | 8.34114E8 |
| 0.02 | 8.02076E8 |
| 0.025 | 7.6148E8 |
| 0.03 | 7.13892E8 |
| 0.035 | 6.61046E8 |
| 0.04 | 6.04746E8 |
| 0.045 | 5.46762E8 |
| 0.05 | 4.88745E8 |
| 0.055 | 4.32158E8 |
| 0.06 | 3.78219E8 |
| 0.065 | 3.27878E8 |
| 0.07 | 2.81807E8 |
| 0.075 | 2.40407E8 |
| 0.08 | 2.03839E8 |
| 0.085 | 1.72056E8 |
| 0.09 | 1.44843E8 |
| 0.095 | 1.21867E8 |
| 0.1 | 1.02711E8 |
| 0.105 | 8.69194E7 |
| 0.11 | 7.40224E7 |
| 0.115 | 6.35659E7 |
| 0.12 | 5.51272E7 |
| 0.125 | 4.83271E7 |
| 0.13 | 4.28356E7 |
| 0.135 | 3.83736E7 |
| 0.14 | 3.47114E7 |
| 0.145 | 3.16642E7 |
| 0.15 | 2.90874E7 |
| 0.155 | 2.687E7 |
| 0.16 | 2.49293E7 |
| 0.165 | 2.3205E7 |
| 0.17 | 2.1654E7 |
| 0.175 | 2.02465E7 |
| 0.18 | 1.89624E7 |
| 0.185 | 1.77881E7 |
| 0.19 | 1.66801E7 |
| 0.195 | 1.57135E7 |
| 0.2 | 1.48317E7 |
| 0.205 | 1.40322E7 |
| 0.21 | 1.33122E7 |
| 0.215 | 1.2669E7 |
| 0.22 | 1.2098E7 |
| 0.225 | 1.15947E7 |
| 0.23 | 1.11539E7 |
| 0.235 | 1.07702E7 |
| 0.24 | 1.04376E7 |
| 0.245 | 1.01498E7 |
| 0.25 | 9.90077E6 |
| 0.255 | 9.68422E6 |
| 0.26 | 9.49403E6 |
| 0.265 | 9.32437E6 |
| 0.27 | 9.16955E6 |
| 0.275 | 9.02459E6 |
| 0.28 | 8.88473E6 |
| 0.285 | 8.74594E6 |
| 0.29 | 8.60467E6 |
| 0.295 | 8.45803E6 |
| 0.3 | 8.30379E6 |
| 0.305 | 8.14053E6 |
| 0.31 | 7.96724E6 |
| 0.315 | 7.78375E6 |
| 0.32 | 7.59034E6 |
| 0.325 | 7.38779E6 |
| 0.33 | 7.17744E6 |
| 0.335 | 6.96096E6 |
| 0.34 | 6.74023E6 |
| 0.345 | 6.51735E6 |
| 0.35 | 6.29444E6 |
| 0.355 | 6.0736E6 |
| 0.36 | 5.85683E6 |
| 0.365 | 5.64611E6 |
| 0.37 | 5.44297E6 |
| 0.375 | 5.2487E6 |
| 0.38 | 5.06422E6 |
| 0.385 | 4.8902E6 |
| 0.39 | 4.7269E6 |
| 0.395 | 4.5743E6 |
| 0.4 | 4.43208E6 |
| 0.405 | 4.29969E6 |
| 0.41 | 4.17636E6 |
| 0.415 | 4.0613E6 |
| 0.42 | 3.9535E6 |
| 0.425 | 3.85202E6 |
| 0.43 | 3.75593E6 |
| 0.435 | 3.66431E6 |
| 0.44 | 3.57644E6 |
| 0.445 | 3.49154E6 |
| 0.45 | 3.40912E6 |
| 0.455 | 3.32865E6 |
| 0.46 | 3.24973E6 |
| 0.465 | 3.17204E6 |
| 0.47 | 3.09537E6 |
| 0.475 | 3.01945E6 |
| 0.48 | 2.94411E6 |
| 0.485 | 2.86918E6 |
| 0.49 | 2.79454E6 |
| 0.495 | 2.72005E6 |
| 0.5 | 2.64566E6 |
| 0.505 | 2.57133E6 |
| 0.51 | 2.49714E6 |
| 0.515 | 2.42321E6 |
| 0.52 | 2.34977E6 |
| 0.525 | 2.27714E6 |
| 0.53 | 2.20561E6 |
| 0.535 | 2.13581E6 |
| 0.54 | 2.06813E6 |
| 0.545 | 2.00304E6 |
| 0.55 | 1.94105E6 |
| 0.555 | 1.88253E6 |
| 0.56 | 1.8278E6 |
| 0.565 | 1.77705E6 |
| 0.57 | 1.73032E6 |
| 0.575 | 1.68756E6 |
| 0.58 | 1.64851E6 |
| 0.585 | 1.61282E6 |
| 0.59 | 1.57998E6 |
| 0.595 | 1.54941E6 |
| 0.6 | 1.52052E6 |

**$Y^+$ : Temperature Vs DR Rate coefficient**

| Temp. (K) | $cm^3/s$ ($10^{-11}$) |
|---|---|
| 2 | 1193.09721 |
| 3 | 976.80724 |
| 4 | 815.57045 |
| 5 | 691.45721 |
| 6 | 594.32934 |
| 7 | 517.27427 |
| 8 | 455.32395 |
| 9 | 404.87023 |
| 10 | 363.28474 |
| 20 | 172.0206 |
| 30 | 113.16594 |
| 40 | 86.64106 |
| 50 | 72.12371 |
| 60 | 63.09265 |
| 70 | 56.90743 |
| 80 | 52.34658 |
| 90 | 48.78964 |
| 100 | 45.89656 |
| 200 | 30.97821 |
| 300 | 24.62323 |
| 400 | 21.21541 |
| 500 | 19.26171 |
| 600 | 18.13182 |
| 700 | 17.50136 |
| 800 | 17.17944 |
| 900 | 17.04553 |
| 1000 | 17.02138 |
| 2000 | 17.2337 |
| 3000 | 16.1729 |
| 4000 | 14.81151 |
| 5000 | 13.58176 |
| 6000 | 12.53731 |
| 7000 | 11.64878 |
| 8000 | 10.88171 |
| 9000 | 10.20974 |
| 10000 | 9.61403 |
| 20000 | 5.95864 |
| 30000 | 4.18445 |
| 40000 | 3.1475 |
| 50000 | 2.47772 |
| 60000 | 2.01547 |
| 70000 | 1.68073 |
| 80000 | 1.42921 |
| 90000 | 1.23461 |
| 100000 | 1.08042 |
| 200000 | 0.42864 |
| 300000 | 0.24286 |
| 400000 | 0.16098 |
| 500000 | 0.11662 |
| 600000 | 0.08945 |
| 700000 | 0.0714 |
| 800000 | 0.0587 |
| 900000 | 0.04937 |
| 1000000 | 0.04227 |
| 2E6 | 0.01513 |
| 3E6 | 0.00827 |
| 4E6 | 0.00538 |
| 5E6 | 0.00386 |
| 6E6 | 0.00294 |
| 7E6 | 0.00233 |
| 8E6 | 0.00191 |
| 9E6 | 0.0016 |
| 1E7 | 0.00137 |
| 2E7 | 4.83998E-4 |
| 3E7 | 2.63566E-4 |
| 4E7 | 1.71228E-4 |
| 5E7 | 1.22536E-4 |
| 6E7 | 9.32241E-5 |
| 7E7 | 7.39834E-5 |
| 8E7 | 6.05572E-5 |
| 9E7 | 5.07519E-5 |
| 1E8 | 4.33339E-5 |
| 2E8 | 1.53228E-5 |
| 3E8 | 8.34103E-6 |
| 4E8 | 5.41777E-6 |
| 5E8 | 3.87669E-6 |
| 6E8 | 2.94912E-6 |
| 7E8 | 2.34032E-6 |
| 8E8 | 1.91553E-6 |
| 9E8 | 1.60532E-6 |
| 1E9 | 1.37065E-6 |
| 2E9 | 4.84605E-7 |
| 3E9 | 2.63787E-7 |
| 4E9 | 1.71335E-7 |
| 5E9 | 1.22597E-7 |
| 6E9 | 9.3263E-8 |
| 7E9 | 7.40099E-8 |
| 8E9 | 6.05762E-8 |
| 9E9 | 5.0766E-8 |
| 1E10 | 4.33448E-8 |
| 2E10 | 1.53247E-8 |
| 3E10 | 8.34173E-9 |
| 4E10 | 5.41811E-9 |
| 5E10 | 3.87689E-9 |
| 6E10 | 2.94925E-9 |
| 7E10 | 2.3404E-9 |
| 8E10 | 1.91559E-9 |
| 9E10 | 1.60537E-9 |
| 1E11 | 1.37069E-9 |

**<u>$Sr^+$ : Temperature Vs DR Rate coefficient</u>**

| Temp. (K) | $cm^3/s$ ($10^{-11}$) |
|---|---|
| 2 | 1.57823 |
| 3 | 8.51942 |
| 4 | 17.4257 |
| 5 | 24.8164 |
| 6 | 29.8705 |
| 7 | 32.8975 |
| 8 | 34.4294 |
| 9 | 34.9327 |
| 10 | 34.7553 |
| 20 | 24.4562 |
| 30 | 16.7452 |
| 40 | 12.1983 |
| 50 | 9.35034 |
| 60 | 7.44703 |
| 70 | 6.10656 |
| 80 | 5.12253 |
| 90 | 4.37581 |
| 100 | 3.79372 |
| 200 | 1.43685 |
| 300 | 0.80027 |
| 400 | 0.52579 |
| 500 | 0.37883 |
| 600 | 0.28952 |
| 700 | 0.23054 |
| 800 | 0.18923 |
| 900 | 0.15899 |
| 1000 | 0.1361 |
| 2000 | 0.05289 |
| 3000 | 0.04184 |
| 4000 | 0.0509 |
| 5000 | 0.07201 |
| 6000 | 0.10037 |
| 7000 | 0.13148 |
| 8000 | 0.16194 |
| 9000 | 0.18966 |
| 10000 | 0.21363 |
| 20000 | 0.28507 |
| 30000 | 0.24722 |
| 40000 | 0.20339 |
| 50000 | 0.1679 |
| 60000 | 0.14056 |
| 70000 | 0.11947 |
| 80000 | 0.10297 |
| 90000 | 0.08984 |
| 100000 | 0.07922 |
| 200000 | 0.03241 |
| 300000 | 0.01852 |
| 400000 | 0.01233 |
| 500000 | 0.00895 |
| 600000 | 0.00688 |
| 700000 | 0.0055 |
| 800000 | 0.00452 |
| 900000 | 0.00381 |
| 1000000 | 0.00326 |
| 2E6 | 0.00117 |
| 3E6 | 6.40016E-4 |
| 4E6 | 4.1673E-4 |
| 5E6 | 2.98629E-4 |
| 6E6 | 2.27399E-4 |
| 7E6 | 1.80582E-4 |
| 8E6 | 1.47882E-4 |
| 9E6 | 1.23984E-4 |
| 1E7 | 1.05894E-4 |
| 2E7 | 3.74948E-5 |
| 3E7 | 2.04197E-5 |
| 4E7 | 1.32662E-5 |
| 5E7 | 9.49396E-6 |
| 6E7 | 7.22301E-6 |
| 7E7 | 5.73229E-6 |
| 8E7 | 4.69206E-6 |
| 9E7 | 3.93235E-6 |
| 1E8 | 3.35761E-6 |
| 2E8 | 1.18727E-6 |
| 3E8 | 6.46301E-7 |
| 4E8 | 4.19795E-7 |
| 5E8 | 3.00385E-7 |
| 6E8 | 2.28513E-7 |
| 7E8 | 1.8134E-7 |
| 8E8 | 1.48425E-7 |
| 9E8 | 1.24389E-7 |
| 1E9 | 1.06205E-7 |
| 2E9 | 3.75498E-8 |
| 3E9 | 2.04396E-8 |
| 4E9 | 1.3276E-8 |
| 5E9 | 9.49953E-9 |
| 6E9 | 7.22654E-9 |
| 7E9 | 5.7347E-9 |
| 8E9 | 4.69378E-9 |
| 9E9 | 3.93363E-9 |
| 1E10 | 3.3586E-9 |
| 2E10 | 1.18745E-9 |
| 3E10 | 6.46364E-10 |
| 4E10 | 4.19826E-10 |
| 5E10 | 3.00403E-10 |
| 6E10 | 2.28524E-10 |
| 7E10 | 1.81348E-10 |
| 8E10 | 1.48431E-10 |
| 9E10 | 1.24393E-10 |
| 1E11 | 1.06208E-10 |

**$Te^{2+}$ : Temperature Vs DR Rate coefficient**

| Temp. (K) | $cm^3/s$ ($10^{-11}$) |
|---|---|
| 2 | 9.9258E-156 |
| 3 | 9.1727E-103 |
| 4 | 2.45484E-76 |
| 5 | 1.63538E-60 |
| 6 | 5.50581E-50 |
| 7 | 1.75658E-42 |
| 8 | 7.25906E-37 |
| 9 | 1.65949E-32 |
| 10 | 5.01182E-29 |
| 20 | 1.64972E-13 |
| 30 | 1.88912E-8 |
| 40 | 5.6279E-6 |
| 50 | 1.59176E-4 |
| 60 | 0.00141 |
| 70 | 0.00642 |
| 80 | 0.01955 |
| 90 | 0.04549 |
| 100 | 0.08793 |
| 200 | 1.22882 |
| 300 | 2.28118 |
| 400 | 2.7516 |
| 500 | 2.88519 |
| 600 | 2.86918 |
| 700 | 2.79308 |
| 800 | 2.69525 |
| 900 | 2.59159 |
| 1000 | 2.48856 |
| 2000 | 1.68077 |
| 3000 | 1.20119 |
| 4000 | 0.90599 |
| 5000 | 0.71317 |
| 6000 | 0.58029 |
| 7000 | 0.48464 |
| 8000 | 0.41338 |
| 9000 | 0.3589 |
| 10000 | 0.31646 |
| 20000 | 0.19516 |
| 30000 | 0.36092 |
| 40000 | 0.65499 |
| 50000 | 0.94707 |
| 60000 | 1.17938 |
| 70000 | 1.34266 |
| 80000 | 1.44632 |
| 90000 | 1.50388 |
| 100000 | 1.52769 |
| 200000 | 1.1936 |
| 300000 | 0.84919 |
| 400000 | 0.63093 |
| 500000 | 0.48946 |
| 600000 | 0.39299 |
| 700000 | 0.32413 |
| 800000 | 0.27308 |
| 900000 | 0.23407 |
| 1000000 | 0.20349 |
| 2E6 | 0.07803 |
| 3E6 | 0.04364 |
| 4E6 | 0.02873 |
| 5E6 | 0.02073 |
| 6E6 | 0.01585 |
| 7E6 | 0.01263 |
| 8E6 | 0.01037 |
| 9E6 | 0.00871 |
| 1E7 | 0.00745 |
| 2E7 | 0.00265 |
| 3E7 | 0.00145 |
| 4E7 | 9.42448E-4 |
| 5E7 | 6.7491E-4 |
| 6E7 | 5.137E-4 |
| 7E7 | 4.0781E-4 |
| 8E7 | 3.33884E-4 |
| 9E7 | 2.79876E-4 |
| 1E8 | 2.39005E-4 |
| 2E8 | 8.45698E-5 |
| 3E8 | 4.60465E-5 |
| 4E8 | 2.99122E-5 |
| 5E8 | 2.14051E-5 |
| 6E8 | 1.62843E-5 |
| 7E8 | 1.29231E-5 |
| 8E8 | 1.05777E-5 |
| 9E8 | 8.86486E-6 |
| 1E9 | 7.56909E-6 |
| 2E9 | 2.6763E-6 |
| 3E9 | 1.45683E-6 |
| 4E9 | 9.46251E-7 |
| 5E9 | 6.77088E-7 |
| 6E9 | 5.15081E-7 |
| 7E9 | 4.08749E-7 |
| 8E9 | 3.34557E-7 |
| 9E9 | 2.80377E-7 |
| 1E10 | 2.39391E-7 |
| 2E10 | 8.4638E-8 |
| 3E10 | 4.60713E-8 |
| 4E10 | 2.99242E-8 |
| 5E10 | 2.1412E-8 |
| 6E10 | 1.62887E-8 |
| 7E10 | 1.29261E-8 |
| 8E10 | 1.05798E-8 |
| 9E10 | 8.86645E-9 |
| 1E11 | 7.57031E-9 |

**$Ce^{2+}$ : Temperature Vs DR Rate coefficient**

| Temp. (K) | $cm^3/s$ $(10^{-11})$ |
|---|---|
| 2 | 2979.07077 |
| 3 | 2155.09568 |
| 4 | 1759.14619 |
| 5 | 1524.7787 |
| 6 | 1371.04422 |
| 7 | 1263.03124 |
| 8 | 1182.72222 |
| 9 | 1119.95344 |
| 10 | 1068.71788 |
| 20 | 782.36266 |
| 30 | 634.00083 |
| 40 | 542.58653 |
| 50 | 481.42354 |
| 60 | 437.41332 |
| 70 | 403.84017 |
| 80 | 377.07111 |
| 90 | 355.01142 |
| 100 | 336.37377 |
| 200 | 234.07662 |
| 300 | 187.53026 |
| 400 | 159.56064 |
| 500 | 140.32662 |
| 600 | 125.96792 |
| 700 | 114.66618 |
| 800 | 105.44548 |
| 900 | 97.72562 |
| 1000 | 91.13522 |
| 2000 | 54.68981 |
| 3000 | 38.63262 |
| 4000 | 29.48307 |
| 5000 | 23.58738 |
| 6000 | 19.48825 |
| 7000 | 16.48513 |
| 8000 | 14.19886 |
| 9000 | 12.40636 |
| 10000 | 10.96779 |
| 20000 | 4.61876 |
| 30000 | 2.6861 |
| 40000 | 1.80647 |
| 50000 | 1.32066 |
| 60000 | 1.0194 |
| 70000 | 0.81752 |
| 80000 | 0.67448 |
| 90000 | 0.56879 |
| 100000 | 0.48809 |
| 200000 | 0.17656 |
| 300000 | 0.09685 |
| 400000 | 0.06315 |
| 500000 | 0.04529 |
| 600000 | 0.03451 |
| 700000 | 0.02742 |
| 800000 | 0.02246 |
| 900000 | 0.01883 |
| 1000000 | 0.01609 |
| 2E6 | 0.0057 |
| 3E6 | 0.00311 |
| 4E6 | 0.00202 |
| 5E6 | 0.00144 |
| 6E6 | 0.0011 |
| 7E6 | 8.72276E-4 |
| 8E6 | 7.14007E-4 |
| 9E6 | 5.98415E-4 |
| 1E7 | 5.10962E-4 |
| 2E7 | 1.80695E-4 |
| 3E7 | 9.83657E-5 |
| 4E7 | 6.38929E-5 |
| 5E7 | 4.57191E-5 |
| 6E7 | 3.47803E-5 |
| 7E7 | 2.76005E-5 |
| 8E7 | 2.25909E-5 |
| 9E7 | 1.89325E-5 |
| 1E8 | 1.61649E-5 |
| 2E8 | 5.7153E-6 |
| 3E8 | 3.11104E-6 |
| 4E8 | 2.02069E-6 |
| 5E8 | 1.44589E-6 |
| 6E8 | 1.09993E-6 |
| 7E8 | 8.72859E-7 |
| 8E8 | 7.14425E-7 |
| 9E8 | 5.98726E-7 |
| 1E9 | 5.11201E-7 |
| 2E9 | 1.80737E-7 |
| 3E9 | 9.83811E-8 |
| 4E9 | 6.39004E-8 |
| 5E9 | 4.57234E-8 |
| 6E9 | 3.4783E-8 |
| 7E9 | 2.76024E-8 |
| 8E9 | 2.25922E-8 |
| 9E9 | 1.89335E-8 |
| 1E10 | 1.61657E-8 |
| 2E10 | 5.71543E-9 |
| 3E10 | 3.11109E-9 |
| 4E10 | 2.02071E-9 |
| 5E10 | 1.4459E-9 |
| 6E10 | 1.09994E-9 |
| 7E10 | 8.72865E-10 |
| 8E10 | 7.14429E-10 |
| 9E10 | 5.98729E-10 |
| 1E11 | 5.11204E-10 |
